# Supplementary material for: Computationally Efficient Neural Image Compression
Source: arXiv:1912.08771 source file (2019-12-18)
Supplement: Supplementary file 1 [file supplementary_table_generated.tex]

\hline1 & MS-SSIM & 64.0 & 5x5deconv,2,10 & 5x5deconv,2,2 & Kodak 1: 0.093272\\ &  &  & 5x5deconv,2,10 & 5x5deconv,2,8 & Kodak 2: 0.100056\\ &  &  & 5x5deconv,2,320 & 5x5deconv,2,1 & Kodak 3: 0.098977\\ &  &  &  & 5x5deconv,2,3 & Kodak 4: 0.099448\\ &  &  &  &  & Kodak 5: 0.101219\\ &  &  &  &  & Kodak 6: 0.102863\\ &  &  &  &  & Kodak 7: 0.100162\\ &  &  &  &  & Kodak 8: 0.098724\\ &  &  &  &  & Kodak 9: 0.100153\\ &  &  &  &  & Kodak 10: 0.105691\\ &  &  &  &  & Kodak 11: 0.101826\\ &  &  &  &  & Kodak 12: 0.102735\\ &  &  &  &  & Kodak 13: 0.099538\\ &  &  &  &  & Kodak 14: 0.106394\\ &  &  &  &  & Kodak 15: 0.102547\\ &  &  &  &  & Kodak 16: 0.098549\\ &  &  &  &  & Kodak 17: 0.101968\\ &  &  &  &  & Kodak 18: 0.106175\\ &  &  &  &  & Kodak 19: 0.107539\\ &  &  &  &  & Kodak 20: 0.099550\\ &  &  &  &  & Kodak 21: 0.098529\\ &  &  &  &  & Kodak 22: 0.101302\\ &  &  &  &  & Kodak 23: 0.102191\\ &  &  &  &  & Kodak 24: 0.102240\\\hline\hline2 & MS-SSIM & 64.0 & 5x5deconv,2,40 & 5x5deconv,2,149 & Kodak 1: 0.140238\\ &  &  & 5x5deconv,2,67 & 5x5deconv,2,35 & Kodak 2: 0.156753\\ &  &  & 5x5deconv,2,320 & 5x5deconv,2,39 & Kodak 3: 0.132692\\ &  &  &  & 5x5deconv,2,3 & Kodak 4: 0.135062\\ &  &  &  &  & Kodak 5: 0.148216\\ &  &  &  &  & Kodak 6: 0.145200\\ &  &  &  &  & Kodak 7: 0.143641\\ &  &  &  &  & Kodak 8: 0.154474\\ &  &  &  &  & Kodak 9: 0.138279\\ &  &  &  &  & Kodak 10: 0.140455\\ &  &  &  &  & Kodak 11: 0.144452\\ &  &  &  &  & Kodak 12: 0.139634\\ &  &  &  &  & Kodak 13: 0.152827\\ &  &  &  &  & Kodak 14: 0.140601\\ &  &  &  &  & Kodak 15: 0.138134\\ &  &  &  &  & Kodak 16: 0.149907\\ &  &  &  &  & Kodak 17: 0.133547\\ &  &  &  &  & Kodak 18: 0.138683\\ &  &  &  &  & Kodak 19: 0.147003\\ &  &  &  &  & Kodak 20: 0.139984\\ &  &  &  &  & Kodak 21: 0.136904\\ &  &  &  &  & Kodak 22: 0.147348\\ &  &  &  &  & Kodak 23: 0.143637\\ &  &  &  &  & Kodak 24: 0.135121\\\hline\hline3 & MS-SSIM & 64.0 & 5x5deconv,2,10 & 5x5deconv,2,1 & Kodak 1: 0.114582\\ &  &  & 5x5deconv,2,10 & 5x5deconv,2,1 & Kodak 2: 0.101269\\ &  &  & 5x5deconv,2,320 & 5x5deconv,2,1 & Kodak 3: 0.096301\\ &  &  &  & 5x5deconv,2,3 & Kodak 4: 0.097648\\ &  &  &  &  & Kodak 5: 0.100836\\ &  &  &  &  & Kodak 6: 0.096909\\ &  &  &  &  & Kodak 7: 0.097554\\ &  &  &  &  & Kodak 8: 0.102259\\ &  &  &  &  & Kodak 9: 0.098885\\ &  &  &  &  & Kodak 10: 0.097325\\ &  &  &  &  & Kodak 11: 0.098470\\ &  &  &  &  & Kodak 12: 0.098390\\ &  &  &  &  & Kodak 13: 0.095414\\ &  &  &  &  & Kodak 14: 0.096647\\ &  &  &  &  & Kodak 15: 0.101267\\ &  &  &  &  & Kodak 16: 0.100629\\ &  &  &  &  & Kodak 17: 0.094195\\ &  &  &  &  & Kodak 18: 0.100423\\ &  &  &  &  & Kodak 19: 0.102808\\ &  &  &  &  & Kodak 20: 0.095789\\ &  &  &  &  & Kodak 21: 0.097336\\ &  &  &  &  & Kodak 22: 0.095855\\ &  &  &  &  & Kodak 23: 0.094633\\ &  &  &  &  & Kodak 24: 0.099954\\\hline\hline4 & MS-SSIM & 64.0 & 5x5deconv,2,10 & 5x5deconv,2,31 & Kodak 1: 0.111265\\ &  &  & 5x5deconv,2,10 & 5x5deconv,2,21 & Kodak 2: 0.121161\\ &  &  & 5x5deconv,2,320 & 5x5deconv,2,11 & Kodak 3: 0.115429\\ &  &  &  & 5x5deconv,2,3 & Kodak 4: 0.113200\\ &  &  &  &  & Kodak 5: 0.119374\\ &  &  &  &  & Kodak 6: 0.117953\\ &  &  &  &  & Kodak 7: 0.119583\\ &  &  &  &  & Kodak 8: 0.117545\\ &  &  &  &  & Kodak 9: 0.110296\\ &  &  &  &  & Kodak 10: 0.118823\\ &  &  &  &  & Kodak 11: 0.120562\\ &  &  &  &  & Kodak 12: 0.114690\\ &  &  &  &  & Kodak 13: 0.120424\\ &  &  &  &  & Kodak 14: 0.115565\\ &  &  &  &  & Kodak 15: 0.122402\\ &  &  &  &  & Kodak 16: 0.117236\\ &  &  &  &  & Kodak 17: 0.114285\\ &  &  &  &  & Kodak 18: 0.112874\\ &  &  &  &  & Kodak 19: 0.115649\\ &  &  &  &  & Kodak 20: 0.114001\\ &  &  &  &  & Kodak 21: 0.116023\\ &  &  &  &  & Kodak 22: 0.113528\\ &  &  &  &  & Kodak 23: 0.120143\\ &  &  &  &  & Kodak 24: 0.111650\\\hline\hline5 & MS-SSIM & 64.0 & 5x5deconv,2,16 & 5x5deconv,2,79 & Kodak 1: 0.129954\\ &  &  & 5x5deconv,2,37 & 5x5deconv,2,22 & Kodak 2: 0.139117\\ &  &  & 5x5deconv,2,320 & 5x5deconv,2,24 & Kodak 3: 0.134138\\ &  &  &  & 5x5deconv,2,3 & Kodak 4: 0.133833\\ &  &  &  &  & Kodak 5: 0.132493\\ &  &  &  &  & Kodak 6: 0.138845\\ &  &  &  &  & Kodak 7: 0.138191\\ &  &  &  &  & Kodak 8: 0.145559\\ &  &  &  &  & Kodak 9: 0.124767\\ &  &  &  &  & Kodak 10: 0.126931\\ &  &  &  &  & Kodak 11: 0.131875\\ &  &  &  &  & Kodak 12: 0.137800\\ &  &  &  &  & Kodak 13: 0.142881\\ &  &  &  &  & Kodak 14: 0.128475\\ &  &  &  &  & Kodak 15: 0.126069\\ &  &  &  &  & Kodak 16: 0.130390\\ &  &  &  &  & Kodak 17: 0.134005\\ &  &  &  &  & Kodak 18: 0.130412\\ &  &  &  &  & Kodak 19: 0.131022\\ &  &  &  &  & Kodak 20: 0.140434\\ &  &  &  &  & Kodak 21: 0.134485\\ &  &  &  &  & Kodak 22: 0.124116\\ &  &  &  &  & Kodak 23: 0.128041\\ &  &  &  &  & Kodak 24: 0.128523\\\hline\hline6 & MS-SSIM & 64.0 & 5x5deconv,2,10 & 5x5deconv,2,1 & Kodak 1: 0.095959\\ &  &  & 5x5deconv,2,10 & 5x5deconv,2,1 & Kodak 2: 0.097427\\ &  &  & 5x5deconv,2,320 & 5x5deconv,2,1 & Kodak 3: 0.098948\\ &  &  &  & 5x5deconv,2,3 & Kodak 4: 0.099438\\ &  &  &  &  & Kodak 5: 0.098589\\ &  &  &  &  & Kodak 6: 0.100879\\ &  &  &  &  & Kodak 7: 0.097406\\ &  &  &  &  & Kodak 8: 0.101494\\ &  &  &  &  & Kodak 9: 0.103918\\ &  &  &  &  & Kodak 10: 0.107349\\ &  &  &  &  & Kodak 11: 0.098948\\ &  &  &  &  & Kodak 12: 0.095828\\ &  &  &  &  & Kodak 13: 0.103889\\ &  &  &  &  & Kodak 14: 0.098221\\ &  &  &  &  & Kodak 15: 0.097311\\ &  &  &  &  & Kodak 16: 0.098389\\ &  &  &  &  & Kodak 17: 0.095941\\ &  &  &  &  & Kodak 18: 0.096014\\ &  &  &  &  & Kodak 19: 0.101755\\ &  &  &  &  & Kodak 20: 0.107805\\ &  &  &  &  & Kodak 21: 0.103185\\ &  &  &  &  & Kodak 22: 0.098981\\ &  &  &  &  & Kodak 23: 0.097358\\ &  &  &  &  & Kodak 24: 0.097596\\\hline\hline7 & MS-SSIM & 64.0 & 5x5deconv,2,10 & 5x5deconv,2,13 & Kodak 1: 0.102687\\ &  &  & 5x5deconv,2,10 & 5x5deconv,2,12 & Kodak 2: 0.119075\\ &  &  & 5x5deconv,2,320 & 5x5deconv,2,3 & Kodak 3: 0.109017\\ &  &  &  & 5x5deconv,2,3 & Kodak 4: 0.115623\\ &  &  &  &  & Kodak 5: 0.111503\\ &  &  &  &  & Kodak 6: 0.109484\\ &  &  &  &  & Kodak 7: 0.109139\\ &  &  &  &  & Kodak 8: 0.100209\\ &  &  &  &  & Kodak 9: 0.109469\\ &  &  &  &  & Kodak 10: 0.105452\\ &  &  &  &  & Kodak 11: 0.104147\\ &  &  &  &  & Kodak 12: 0.106006\\ &  &  &  &  & Kodak 13: 0.102768\\ &  &  &  &  & Kodak 14: 0.113828\\ &  &  &  &  & Kodak 15: 0.100484\\ &  &  &  &  & Kodak 16: 0.105011\\ &  &  &  &  & Kodak 17: 0.102770\\ &  &  &  &  & Kodak 18: 0.105477\\ &  &  &  &  & Kodak 19: 0.103627\\ &  &  &  &  & Kodak 20: 0.104898\\ &  &  &  &  & Kodak 21: 0.111625\\ &  &  &  &  & Kodak 22: 0.110366\\ &  &  &  &  & Kodak 23: 0.116081\\ &  &  &  &  & Kodak 24: 0.101002\\\hline\hline\hline\hline9 & MS-SSIM & 64.0 & 5x5deconv,2,10 & 5x5deconv,2,1 & Kodak 1: 0.087408\\ &  &  & 5x5deconv,2,10 & 5x5deconv,2,1 & Kodak 2: 0.094874\\ &  &  & 5x5deconv,2,320 & 5x5deconv,2,1 & Kodak 3: 0.092652\\ &  &  &  & 5x5deconv,2,3 & Kodak 4: 0.093590\\ &  &  &  &  & Kodak 5: 0.113031\\ &  &  &  &  & Kodak 6: 0.093179\\ &  &  &  &  & Kodak 7: 0.096246\\ &  &  &  &  & Kodak 8: 0.094199\\ &  &  &  &  & Kodak 9: 0.092242\\ &  &  &  &  & Kodak 10: 0.094997\\ &  &  &  &  & Kodak 11: 0.097419\\ &  &  &  &  & Kodak 12: 0.098054\\ &  &  &  &  & Kodak 13: 0.094457\\ &  &  &  &  & Kodak 14: 0.096346\\ &  &  &  &  & Kodak 15: 0.094492\\ &  &  &  &  & Kodak 16: 0.095043\\ &  &  &  &  & Kodak 17: 0.096040\\ &  &  &  &  & Kodak 18: 0.095507\\ &  &  &  &  & Kodak 19: 0.094160\\ &  &  &  &  & Kodak 20: 0.095833\\ &  &  &  &  & Kodak 21: 0.098892\\ &  &  &  &  & Kodak 22: 0.092088\\ &  &  &  &  & Kodak 23: 0.096637\\ &  &  &  &  & Kodak 24: 0.094732\\\hline\hline10 & MS-SSIM & 64.0 & 5x5deconv,2,66 & 5x5deconv,2,180 & Kodak 1: 0.171107\\ &  &  & 5x5deconv,2,95 & 5x5deconv,2,58 & Kodak 2: 0.182672\\ &  &  & 5x5deconv,2,320 & 5x5deconv,2,73 & Kodak 3: 0.175195\\ &  &  &  & 5x5deconv,2,3 & Kodak 4: 0.167105\\ &  &  &  &  & Kodak 5: 0.172271\\ &  &  &  &  & Kodak 6: 0.167401\\ &  &  &  &  & Kodak 7: 0.175592\\ &  &  &  &  & Kodak 8: 0.182968\\ &  &  &  &  & Kodak 9: 0.164245\\ &  &  &  &  & Kodak 10: 0.159570\\ &  &  &  &  & Kodak 11: 0.159513\\ &  &  &  &  & Kodak 12: 0.168965\\ &  &  &  &  & Kodak 13: 0.191234\\ &  &  &  &  & Kodak 14: 0.179241\\ &  &  &  &  & Kodak 15: 0.170850\\ &  &  &  &  & Kodak 16: 0.161020\\ &  &  &  &  & Kodak 17: 0.163237\\ &  &  &  &  & Kodak 18: 0.165196\\ &  &  &  &  & Kodak 19: 0.164091\\ &  &  &  &  & Kodak 20: 0.160178\\ &  &  &  &  & Kodak 21: 0.170459\\ &  &  &  &  & Kodak 22: 0.163610\\ &  &  &  &  & Kodak 23: 0.159231\\ &  &  &  &  & Kodak 24: 0.176816\\\hline\hline11 & MS-SSIM & 64.0 & 5x5deconv,2,131 & 5x5deconv,2,275 & Kodak 1: 0.235752\\ &  &  & 5x5deconv,2,195 & 5x5deconv,2,103 & Kodak 2: 0.207489\\ &  &  & 5x5deconv,2,320 & 5x5deconv,2,117 & Kodak 3: 0.204948\\ &  &  &  & 5x5deconv,2,3 & Kodak 4: 0.230348\\ &  &  &  &  & Kodak 5: 0.214000\\ &  &  &  &  & Kodak 6: 0.209886\\ &  &  &  &  & Kodak 7: 0.205829\\ &  &  &  &  & Kodak 8: 0.227582\\ &  &  &  &  & Kodak 9: 0.208464\\ &  &  &  &  & Kodak 10: 0.212098\\ &  &  &  &  & Kodak 11: 0.214847\\ &  &  &  &  & Kodak 12: 0.207423\\ &  &  &  &  & Kodak 13: 0.208283\\ &  &  &  &  & Kodak 14: 0.210726\\ &  &  &  &  & Kodak 15: 0.206174\\ &  &  &  &  & Kodak 16: 0.210848\\ &  &  &  &  & Kodak 17: 0.233174\\ &  &  &  &  & Kodak 18: 0.213290\\ &  &  &  &  & Kodak 19: 0.217247\\ &  &  &  &  & Kodak 20: 0.205603\\ &  &  &  &  & Kodak 21: 0.205752\\ &  &  &  &  & Kodak 22: 0.207032\\ &  &  &  &  & Kodak 23: 0.235808\\ &  &  &  &  & Kodak 24: 0.209783\\\hline\hline12 & MS-SSIM & 64.0 & 5x5deconv,2,165 & 5x5deconv,2,317 & Kodak 1: 0.325368\\ &  &  & 5x5deconv,2,261 & 5x5deconv,2,160 & Kodak 2: 0.279674\\ &  &  & 5x5deconv,2,320 & 5x5deconv,2,183 & Kodak 3: 0.269929\\ &  &  &  & 5x5deconv,2,3 & Kodak 4: 0.276418\\ &  &  &  &  & Kodak 5: 0.272414\\ &  &  &  &  & Kodak 6: 0.275927\\ &  &  &  &  & Kodak 7: 0.272962\\ &  &  &  &  & Kodak 8: 0.311311\\ &  &  &  &  & Kodak 9: 0.279157\\ &  &  &  &  & Kodak 10: 0.272621\\ &  &  &  &  & Kodak 11: 0.272800\\ &  &  &  &  & Kodak 12: 0.277362\\ &  &  &  &  & Kodak 13: 0.272902\\ &  &  &  &  & Kodak 14: 0.275124\\ &  &  &  &  & Kodak 15: 0.267915\\ &  &  &  &  & Kodak 16: 0.311603\\ &  &  &  &  & Kodak 17: 0.276464\\ &  &  &  &  & Kodak 18: 0.271998\\ &  &  &  &  & Kodak 19: 0.273097\\ &  &  &  &  & Kodak 20: 0.269020\\ &  &  &  &  & Kodak 21: 0.273418\\ &  &  &  &  & Kodak 22: 0.277777\\ &  &  &  &  & Kodak 23: 0.272125\\ &  &  &  &  & Kodak 24: 0.308925\\\hline\hline13 & MS-SSIM & 64.0 & 5x5deconv,2,165 & 5x5deconv,2,315 & Kodak 1: 0.276116\\ &  &  & 5x5deconv,2,263 & 5x5deconv,2,152 & Kodak 2: 0.270486\\ &  &  & 5x5deconv,2,320 & 5x5deconv,2,182 & Kodak 3: 0.267774\\ &  &  &  & 5x5deconv,2,3 & Kodak 4: 0.269958\\ &  &  &  &  & Kodak 5: 0.270306\\ &  &  &  &  & Kodak 6: 0.270013\\ &  &  &  &  & Kodak 7: 0.264474\\ &  &  &  &  & Kodak 8: 0.267648\\ &  &  &  &  & Kodak 9: 0.259643\\ &  &  &  &  & Kodak 10: 0.265735\\ &  &  &  &  & Kodak 11: 0.275494\\ &  &  &  &  & Kodak 12: 0.269859\\ &  &  &  &  & Kodak 13: 0.269692\\ &  &  &  &  & Kodak 14: 0.276374\\ &  &  &  &  & Kodak 15: 0.268192\\ &  &  &  &  & Kodak 16: 0.278923\\ &  &  &  &  & Kodak 17: 0.296440\\ &  &  &  &  & Kodak 18: 0.278199\\ &  &  &  &  & Kodak 19: 0.279521\\ &  &  &  &  & Kodak 20: 0.264949\\ &  &  &  &  & Kodak 21: 0.271295\\ &  &  &  &  & Kodak 22: 0.270153\\ &  &  &  &  & Kodak 23: 0.266060\\ &  &  &  &  & Kodak 24: 0.268310\\\hline\hline14 & MSE & 0.0015625 & 5x5deconv,2,10 & 5x5deconv,2,1 & Kodak 1: 0.092512\\ &  &  & 5x5deconv,2,10 & 5x5deconv,2,2 & Kodak 2: 0.097237\\ &  &  & 5x5deconv,2,320 & 5x5deconv,2,2 & Kodak 3: 0.095009\\ &  &  &  & 5x5deconv,2,3 & Kodak 4: 0.100669\\ &  &  &  &  & Kodak 5: 0.096078\\ &  &  &  &  & Kodak 6: 0.096552\\ &  &  &  &  & Kodak 7: 0.098373\\ &  &  &  &  & Kodak 8: 0.102293\\ &  &  &  &  & Kodak 9: 0.094603\\ &  &  &  &  & Kodak 10: 0.095853\\ &  &  &  &  & Kodak 11: 0.097187\\ &  &  &  &  & Kodak 12: 0.101117\\ &  &  &  &  & Kodak 13: 0.095438\\ &  &  &  &  & Kodak 14: 0.091758\\ &  &  &  &  & Kodak 15: 0.093666\\ &  &  &  &  & Kodak 16: 0.099683\\ &  &  &  &  & Kodak 17: 0.094442\\ &  &  &  &  & Kodak 18: 0.098339\\ &  &  &  &  & Kodak 19: 0.099576\\ &  &  &  &  & Kodak 20: 0.096081\\ &  &  &  &  & Kodak 21: 0.094099\\ &  &  &  &  & Kodak 22: 0.093441\\ &  &  &  &  & Kodak 23: 0.101644\\ &  &  &  &  & Kodak 24: 0.099062\\\hline\hline15 & MSE & 0.0015625 & 5x5deconv,2,211 & 5x5deconv,2,312 & Kodak 1: 0.431337\\ &  &  & 5x5deconv,2,263 & 5x5deconv,2,257 & Kodak 2: 0.418471\\ &  &  & 5x5deconv,2,320 & 5x5deconv,2,315 & Kodak 3: 0.439480\\ &  &  &  & 5x5deconv,2,3 & Kodak 4: 0.428087\\ &  &  &  &  & Kodak 5: 0.418142\\ &  &  &  &  & Kodak 6: 0.421950\\ &  &  &  &  & Kodak 7: 0.423941\\ &  &  &  &  & Kodak 8: 0.420487\\ &  &  &  &  & Kodak 9: 0.417821\\ &  &  &  &  & Kodak 10: 0.423731\\ &  &  &  &  & Kodak 11: 0.417543\\ &  &  &  &  & Kodak 12: 0.425438\\ &  &  &  &  & Kodak 13: 0.423247\\ &  &  &  &  & Kodak 14: 0.429344\\ &  &  &  &  & Kodak 15: 0.419069\\ &  &  &  &  & Kodak 16: 0.417620\\ &  &  &  &  & Kodak 17: 0.456467\\ &  &  &  &  & Kodak 18: 0.423475\\ &  &  &  &  & Kodak 19: 0.462917\\ &  &  &  &  & Kodak 20: 0.430783\\ &  &  &  &  & Kodak 21: 0.420374\\ &  &  &  &  & Kodak 22: 0.419500\\ &  &  &  &  & Kodak 23: 0.423072\\ &  &  &  &  & Kodak 24: 0.414856\\\hline\hline16 & MSE & 0.0015625 & 5x5deconv,2,84 & 5x5deconv,2,53 & Kodak 1: 0.110619\\ &  &  & 5x5deconv,2,86 & 5x5deconv,2,28 & Kodak 2: 0.129833\\ &  &  & 5x5deconv,2,320 & 5x5deconv,2,30 & Kodak 3: 0.130570\\ &  &  &  & 5x5deconv,2,3 & Kodak 4: 0.121770\\ &  &  &  &  & Kodak 5: 0.118524\\ &  &  &  &  & Kodak 6: 0.114241\\ &  &  &  &  & Kodak 7: 0.126988\\ &  &  &  &  & Kodak 8: 0.125351\\ &  &  &  &  & Kodak 9: 0.125748\\ &  &  &  &  & Kodak 10: 0.121634\\ &  &  &  &  & Kodak 11: 0.121302\\ &  &  &  &  & Kodak 12: 0.118922\\ &  &  &  &  & Kodak 13: 0.120758\\ &  &  &  &  & Kodak 14: 0.120584\\ &  &  &  &  & Kodak 15: 0.117562\\ &  &  &  &  & Kodak 16: 0.124406\\ &  &  &  &  & Kodak 17: 0.117166\\ &  &  &  &  & Kodak 18: 0.117616\\ &  &  &  &  & Kodak 19: 0.122705\\ &  &  &  &  & Kodak 20: 0.125896\\ &  &  &  &  & Kodak 21: 0.131406\\ &  &  &  &  & Kodak 22: 0.117561\\ &  &  &  &  & Kodak 23: 0.122774\\ &  &  &  &  & Kodak 24: 0.119143\\\hline\hline17 & MSE & 0.0015625 & 5x5deconv,2,10 & 5x5deconv,2,1 & Kodak 1: 0.092220\\ &  &  & 5x5deconv,2,10 & 5x5deconv,2,2 & Kodak 2: 0.098410\\ &  &  & 5x5deconv,2,320 & 5x5deconv,2,1 & Kodak 3: 0.096245\\ &  &  &  & 5x5deconv,2,3 & Kodak 4: 0.097425\\ &  &  &  &  & Kodak 5: 0.098397\\ &  &  &  &  & Kodak 6: 0.100355\\ &  &  &  &  & Kodak 7: 0.096522\\ &  &  &  &  & Kodak 8: 0.095518\\ &  &  &  &  & Kodak 9: 0.092845\\ &  &  &  &  & Kodak 10: 0.097041\\ &  &  &  &  & Kodak 11: 0.095561\\ &  &  &  &  & Kodak 12: 0.094760\\ &  &  &  &  & Kodak 13: 0.097216\\ &  &  &  &  & Kodak 14: 0.098199\\ &  &  &  &  & Kodak 15: 0.095307\\ &  &  &  &  & Kodak 16: 0.095351\\ &  &  &  &  & Kodak 17: 0.098662\\ &  &  &  &  & Kodak 18: 0.101498\\ &  &  &  &  & Kodak 19: 0.096930\\ &  &  &  &  & Kodak 20: 0.095359\\ &  &  &  &  & Kodak 21: 0.099030\\ &  &  &  &  & Kodak 22: 0.097659\\ &  &  &  &  & Kodak 23: 0.096074\\ &  &  &  &  & Kodak 24: 0.099201\\\hline\hline18 & MSE & 0.0015625 & 5x5deconv,2,41 & 5x5deconv,2,18 & Kodak 1: 0.101650\\ &  &  & 5x5deconv,2,27 & 5x5deconv,2,25 & Kodak 2: 0.100158\\ &  &  & 5x5deconv,2,320 & 5x5deconv,2,9 & Kodak 3: 0.102526\\ &  &  &  & 5x5deconv,2,3 & Kodak 4: 0.105005\\ &  &  &  &  & Kodak 5: 0.104515\\ &  &  &  &  & Kodak 6: 0.106779\\ &  &  &  &  & Kodak 7: 0.105053\\ &  &  &  &  & Kodak 8: 0.112423\\ &  &  &  &  & Kodak 9: 0.104368\\ &  &  &  &  & Kodak 10: 0.103739\\ &  &  &  &  & Kodak 11: 0.106082\\ &  &  &  &  & Kodak 12: 0.104529\\ &  &  &  &  & Kodak 13: 0.105445\\ &  &  &  &  & Kodak 14: 0.111130\\ &  &  &  &  & Kodak 15: 0.113776\\ &  &  &  &  & Kodak 16: 0.106635\\ &  &  &  &  & Kodak 17: 0.107942\\ &  &  &  &  & Kodak 18: 0.113061\\ &  &  &  &  & Kodak 19: 0.104891\\ &  &  &  &  & Kodak 20: 0.103573\\ &  &  &  &  & Kodak 21: 0.112032\\ &  &  &  &  & Kodak 22: 0.101836\\ &  &  &  &  & Kodak 23: 0.110206\\ &  &  &  &  & Kodak 24: 0.110484\\\hline\hline19 & MSE & 0.0015625 & 5x5deconv,2,212 & 5x5deconv,2,105 & Kodak 1: 0.151509\\ &  &  & 5x5deconv,2,146 & 5x5deconv,2,60 & Kodak 2: 0.148534\\ &  &  & 5x5deconv,2,320 & 5x5deconv,2,66 & Kodak 3: 0.148035\\ &  &  &  & 5x5deconv,2,3 & Kodak 4: 0.147313\\ &  &  &  &  & Kodak 5: 0.151534\\ &  &  &  &  & Kodak 6: 0.158716\\ &  &  &  &  & Kodak 7: 0.153656\\ &  &  &  &  & Kodak 8: 0.148211\\ &  &  &  &  & Kodak 9: 0.148983\\ &  &  &  &  & Kodak 10: 0.152566\\ &  &  &  &  & Kodak 11: 0.145784\\ &  &  &  &  & Kodak 12: 0.156267\\ &  &  &  &  & Kodak 13: 0.149760\\ &  &  &  &  & Kodak 14: 0.152226\\ &  &  &  &  & Kodak 15: 0.149298\\ &  &  &  &  & Kodak 16: 0.153023\\ &  &  &  &  & Kodak 17: 0.147134\\ &  &  &  &  & Kodak 18: 0.145275\\ &  &  &  &  & Kodak 19: 0.155837\\ &  &  &  &  & Kodak 20: 0.147641\\ &  &  &  &  & Kodak 21: 0.155201\\ &  &  &  &  & Kodak 22: 0.147829\\ &  &  &  &  & Kodak 23: 0.158505\\ &  &  &  &  & Kodak 24: 0.152366\\\hline\hline20 & MSE & 0.0015625 & 5x5deconv,2,14 & 5x5deconv,2,7 & Kodak 1: 0.101025\\ &  &  & 5x5deconv,2,12 & 5x5deconv,2,18 & Kodak 2: 0.106677\\ &  &  & 5x5deconv,2,320 & 5x5deconv,2,5 & Kodak 3: 0.099697\\ &  &  &  & 5x5deconv,2,3 & Kodak 4: 0.099012\\ &  &  &  &  & Kodak 5: 0.102437\\ &  &  &  &  & Kodak 6: 0.105668\\ &  &  &  &  & Kodak 7: 0.101996\\ &  &  &  &  & Kodak 8: 0.101835\\ &  &  &  &  & Kodak 9: 0.105227\\ &  &  &  &  & Kodak 10: 0.101879\\ &  &  &  &  & Kodak 11: 0.102854\\ &  &  &  &  & Kodak 12: 0.104633\\ &  &  &  &  & Kodak 13: 0.106521\\ &  &  &  &  & Kodak 14: 0.103718\\ &  &  &  &  & Kodak 15: 0.100251\\ &  &  &  &  & Kodak 16: 0.102416\\ &  &  &  &  & Kodak 17: 0.110959\\ &  &  &  &  & Kodak 18: 0.103931\\ &  &  &  &  & Kodak 19: 0.101947\\ &  &  &  &  & Kodak 20: 0.099087\\ &  &  &  &  & Kodak 21: 0.100133\\ &  &  &  &  & Kodak 22: 0.100540\\ &  &  &  &  & Kodak 23: 0.111679\\ &  &  &  &  & Kodak 24: 0.102906\\\hline\hline21 & MSE & 0.0015625 & 5x5deconv,2,509 & 5x5deconv,2,173 & Kodak 1: 0.273487\\ &  &  & 5x5deconv,2,222 & 5x5deconv,2,106 & Kodak 2: 0.245706\\ &  &  & 5x5deconv,2,320 & 5x5deconv,2,190 & Kodak 3: 0.280413\\ &  &  &  & 5x5deconv,2,3 & Kodak 4: 0.247817\\ &  &  &  &  & Kodak 5: 0.252857\\ &  &  &  &  & Kodak 6: 0.247740\\ &  &  &  &  & Kodak 7: 0.285755\\ &  &  &  &  & Kodak 8: 0.249368\\ &  &  &  &  & Kodak 9: 0.247750\\ &  &  &  &  & Kodak 10: 0.245309\\ &  &  &  &  & Kodak 11: 0.278790\\ &  &  &  &  & Kodak 12: 0.251202\\ &  &  &  &  & Kodak 13: 0.284135\\ &  &  &  &  & Kodak 14: 0.249705\\ &  &  &  &  & Kodak 15: 0.249708\\ &  &  &  &  & Kodak 16: 0.243078\\ &  &  &  &  & Kodak 17: 0.245214\\ &  &  &  &  & Kodak 18: 0.255314\\ &  &  &  &  & Kodak 19: 0.249354\\ &  &  &  &  & Kodak 20: 0.245806\\ &  &  &  &  & Kodak 21: 0.248449\\ &  &  &  &  & Kodak 22: 0.286810\\ &  &  &  &  & Kodak 23: 0.250695\\ &  &  &  &  & Kodak 24: 0.247597\\\hline\hline22 & MSE & 0.0015625 & 5x5deconv,2,149 & 5x5deconv,2,320 & Kodak 1: 0.500160\\ &  &  & 5x5deconv,2,274 & 5x5deconv,2,320 & Kodak 2: 0.474440\\ &  &  & 5x5deconv,2,320 & 5x5deconv,2,319 & Kodak 3: 0.472575\\ &  &  &  & 5x5deconv,2,3 & Kodak 4: 0.480181\\ &  &  &  &  & Kodak 5: 0.480926\\ &  &  &  &  & Kodak 6: 0.474378\\ &  &  &  &  & Kodak 7: 0.474205\\ &  &  &  &  & Kodak 8: 0.476402\\ &  &  &  &  & Kodak 9: 0.470146\\ &  &  &  &  & Kodak 10: 0.475142\\ &  &  &  &  & Kodak 11: 0.481924\\ &  &  &  &  & Kodak 12: 0.493361\\ &  &  &  &  & Kodak 13: 0.481592\\ &  &  &  &  & Kodak 14: 0.474290\\ &  &  &  &  & Kodak 15: 0.473110\\ &  &  &  &  & Kodak 16: 0.472871\\ &  &  &  &  & Kodak 17: 0.484714\\ &  &  &  &  & Kodak 18: 0.471219\\ &  &  &  &  & Kodak 19: 0.471940\\ &  &  &  &  & Kodak 20: 0.468079\\ &  &  &  &  & Kodak 21: 0.475723\\ &  &  &  &  & Kodak 22: 0.474125\\ &  &  &  &  & Kodak 23: 0.479670\\ &  &  &  &  & Kodak 24: 0.490220\\\hline\hline23 & MSE & 0.0015625 & 5x5deconv,2,586 & 5x5deconv,2,241 & Kodak 1: 0.366966\\ &  &  & 5x5deconv,2,245 & 5x5deconv,2,157 & Kodak 2: 0.324513\\ &  &  & 5x5deconv,2,320 & 5x5deconv,2,269 & Kodak 3: 0.325068\\ &  &  &  & 5x5deconv,2,3 & Kodak 4: 0.323953\\ &  &  &  &  & Kodak 5: 0.328388\\ &  &  &  &  & Kodak 6: 0.326385\\ &  &  &  &  & Kodak 7: 0.326264\\ &  &  &  &  & Kodak 8: 0.326265\\ &  &  &  &  & Kodak 9: 0.333325\\ &  &  &  &  & Kodak 10: 0.330134\\ &  &  &  &  & Kodak 11: 0.325961\\ &  &  &  &  & Kodak 12: 0.328356\\ &  &  &  &  & Kodak 13: 0.329735\\ &  &  &  &  & Kodak 14: 0.329979\\ &  &  &  &  & Kodak 15: 0.328862\\ &  &  &  &  & Kodak 16: 0.375797\\ &  &  &  &  & Kodak 17: 0.328059\\ &  &  &  &  & Kodak 18: 0.334174\\ &  &  &  &  & Kodak 19: 0.324023\\ &  &  &  &  & Kodak 20: 0.325440\\ &  &  &  &  & Kodak 21: 0.375120\\ &  &  &  &  & Kodak 22: 0.328274\\ &  &  &  &  & Kodak 23: 0.374461\\ &  &  &  &  & Kodak 24: 0.326055\\\hline\hline24 & MSE & 0.0015625 & 5x5deconv,2,4 & 5x5deconv,2,4 & Kodak 1: 0.094844\\ &  &  & 5x5deconv,2,3 & 5x5deconv,2,7 & Kodak 2: 0.098531\\ &  &  & 5x5deconv,2,320 & 5x5deconv,2,3 & Kodak 3: 0.098840\\ &  &  &  & 5x5deconv,2,3 & Kodak 4: 0.102044\\ &  &  &  &  & Kodak 5: 0.102085\\ &  &  &  &  & Kodak 6: 0.100036\\ &  &  &  &  & Kodak 7: 0.100846\\ &  &  &  &  & Kodak 8: 0.100104\\ &  &  &  &  & Kodak 9: 0.100471\\ &  &  &  &  & Kodak 10: 0.099745\\ &  &  &  &  & Kodak 11: 0.097652\\ &  &  &  &  & Kodak 12: 0.098741\\ &  &  &  &  & Kodak 13: 0.107182\\ &  &  &  &  & Kodak 14: 0.098099\\ &  &  &  &  & Kodak 15: 0.102872\\ &  &  &  &  & Kodak 16: 0.091896\\ &  &  &  &  & Kodak 17: 0.097761\\ &  &  &  &  & Kodak 18: 0.103457\\ &  &  &  &  & Kodak 19: 0.097884\\ &  &  &  &  & Kodak 20: 0.100127\\ &  &  &  &  & Kodak 21: 0.100738\\ &  &  &  &  & Kodak 22: 0.100513\\ &  &  &  &  & Kodak 23: 0.098918\\ &  &  &  &  & Kodak 24: 0.101408\\\hline\hline25 & MSE & 0.0015625 & 5x5deconv,2,10 & 5x5deconv,2,3 & Kodak 1: 0.105280\\ &  &  & 5x5deconv,2,10 & 5x5deconv,2,4 & Kodak 2: 0.098533\\ &  &  & 5x5deconv,2,320 & 5x5deconv,2,1 & Kodak 3: 0.105095\\ &  &  &  & 5x5deconv,2,3 & Kodak 4: 0.096268\\ &  &  &  &  & Kodak 5: 0.094461\\ &  &  &  &  & Kodak 6: 0.099973\\ &  &  &  &  & Kodak 7: 0.100555\\ &  &  &  &  & Kodak 8: 0.098986\\ &  &  &  &  & Kodak 9: 0.098745\\ &  &  &  &  & Kodak 10: 0.103517\\ &  &  &  &  & Kodak 11: 0.101530\\ &  &  &  &  & Kodak 12: 0.099177\\ &  &  &  &  & Kodak 13: 0.096153\\ &  &  &  &  & Kodak 14: 0.098984\\ &  &  &  &  & Kodak 15: 0.099340\\ &  &  &  &  & Kodak 16: 0.103102\\ &  &  &  &  & Kodak 17: 0.099710\\ &  &  &  &  & Kodak 18: 0.102090\\ &  &  &  &  & Kodak 19: 0.096819\\ &  &  &  &  & Kodak 20: 0.105584\\ &  &  &  &  & Kodak 21: 0.101530\\ &  &  &  &  & Kodak 22: 0.095476\\ &  &  &  &  & Kodak 23: 0.102936\\ &  &  &  &  & Kodak 24: 0.095722\\\hline\hline26 & MS-SSIM & 2.0 & 5x5deconv,2,10 & 5x5deconv,2,1 & Kodak 1: 0.092743\\ &  &  & 5x5deconv,2,10 & 5x5deconv,2,1 & Kodak 2: 0.098528\\ &  &  & 5x5deconv,2,320 & 5x5deconv,2,1 & Kodak 3: 0.101634\\ &  &  &  & 5x5deconv,2,3 & Kodak 4: 0.099489\\ &  &  &  &  & Kodak 5: 0.099388\\ &  &  &  &  & Kodak 6: 0.117652\\ &  &  &  &  & Kodak 7: 0.098822\\ &  &  &  &  & Kodak 8: 0.096840\\ &  &  &  &  & Kodak 9: 0.102367\\ &  &  &  &  & Kodak 10: 0.094328\\ &  &  &  &  & Kodak 11: 0.100442\\ &  &  &  &  & Kodak 12: 0.097059\\ &  &  &  &  & Kodak 13: 0.095411\\ &  &  &  &  & Kodak 14: 0.095928\\ &  &  &  &  & Kodak 15: 0.099543\\ &  &  &  &  & Kodak 16: 0.097133\\ &  &  &  &  & Kodak 17: 0.096665\\ &  &  &  &  & Kodak 18: 0.101632\\ &  &  &  &  & Kodak 19: 0.097240\\ &  &  &  &  & Kodak 20: 0.096758\\ &  &  &  &  & Kodak 21: 0.097461\\ &  &  &  &  & Kodak 22: 0.096932\\ &  &  &  &  & Kodak 23: 0.101012\\ &  &  &  &  & Kodak 24: 0.097938\\\hline\hline27 & MS-SSIM & 2.0 & 5x5deconv,2,10 & 5x5deconv,2,1 & Kodak 1: 0.089020\\ &  &  & 5x5deconv,2,10 & 5x5deconv,2,1 & Kodak 2: 0.097048\\ &  &  & 5x5deconv,2,320 & 5x5deconv,2,1 & Kodak 3: 0.104612\\ &  &  &  & 5x5deconv,2,3 & Kodak 4: 0.096808\\ &  &  &  &  & Kodak 5: 0.097988\\ &  &  &  &  & Kodak 6: 0.110646\\ &  &  &  &  & Kodak 7: 0.096642\\ &  &  &  &  & Kodak 8: 0.098038\\ &  &  &  &  & Kodak 9: 0.094994\\ &  &  &  &  & Kodak 10: 0.101120\\ &  &  &  &  & Kodak 11: 0.094307\\ &  &  &  &  & Kodak 12: 0.095246\\ &  &  &  &  & Kodak 13: 0.096688\\ &  &  &  &  & Kodak 14: 0.098938\\ &  &  &  &  & Kodak 15: 0.097632\\ &  &  &  &  & Kodak 16: 0.101731\\ &  &  &  &  & Kodak 17: 0.101537\\ &  &  &  &  & Kodak 18: 0.100044\\ &  &  &  &  & Kodak 19: 0.095891\\ &  &  &  &  & Kodak 20: 0.102832\\ &  &  &  &  & Kodak 21: 0.094462\\ &  &  &  &  & Kodak 22: 0.100520\\ &  &  &  &  & Kodak 23: 0.096222\\ &  &  &  &  & Kodak 24: 0.097420\\\hline\hline28 & MS-SSIM & 2.0 & 5x5deconv,2,10 & 5x5deconv,2,1 & Kodak 1: 0.090243\\ &  &  & 5x5deconv,2,10 & 5x5deconv,2,1 & Kodak 2: 0.098429\\ &  &  & 5x5deconv,2,320 & 5x5deconv,2,1 & Kodak 3: 0.098173\\ &  &  &  & 5x5deconv,2,3 & Kodak 4: 0.098195\\ &  &  &  &  & Kodak 5: 0.102242\\ &  &  &  &  & Kodak 6: 0.105776\\ &  &  &  &  & Kodak 7: 0.097441\\ &  &  &  &  & Kodak 8: 0.099857\\ &  &  &  &  & Kodak 9: 0.099468\\ &  &  &  &  & Kodak 10: 0.098980\\ &  &  &  &  & Kodak 11: 0.094879\\ &  &  &  &  & Kodak 12: 0.097696\\ &  &  &  &  & Kodak 13: 0.104716\\ &  &  &  &  & Kodak 14: 0.094627\\ &  &  &  &  & Kodak 15: 0.097783\\ &  &  &  &  & Kodak 16: 0.099771\\ &  &  &  &  & Kodak 17: 0.105615\\ &  &  &  &  & Kodak 18: 0.107687\\ &  &  &  &  & Kodak 19: 0.103283\\ &  &  &  &  & Kodak 20: 0.104051\\ &  &  &  &  & Kodak 21: 0.105016\\ &  &  &  &  & Kodak 22: 0.097299\\ &  &  &  &  & Kodak 23: 0.105011\\ &  &  &  &  & Kodak 24: 0.101203\\\hline\hline29 & MS-SSIM & 2.0 & 5x5deconv,2,448 & 5x5deconv,2,220 & Kodak 1: 0.329634\\ &  &  & 5x5deconv,2,426 & 5x5deconv,2,288 & Kodak 2: 0.335093\\ &  &  & 5x5deconv,2,320 & 5x5deconv,2,160 & Kodak 3: 0.302241\\ &  &  &  & 5x5deconv,2,3 & Kodak 4: 0.297919\\ &  &  &  &  & Kodak 5: 0.309639\\ &  &  &  &  & Kodak 6: 0.310477\\ &  &  &  &  & Kodak 7: 0.304693\\ &  &  &  &  & Kodak 8: 0.309717\\ &  &  &  &  & Kodak 9: 0.299755\\ &  &  &  &  & Kodak 10: 0.299757\\ &  &  &  &  & Kodak 11: 0.310184\\ &  &  &  &  & Kodak 12: 0.316781\\ &  &  &  &  & Kodak 13: 0.315323\\ &  &  &  &  & Kodak 14: 0.303319\\ &  &  &  &  & Kodak 15: 0.302174\\ &  &  &  &  & Kodak 16: 0.302094\\ &  &  &  &  & Kodak 17: 0.331441\\ &  &  &  &  & Kodak 18: 0.367038\\ &  &  &  &  & Kodak 19: 0.299159\\ &  &  &  &  & Kodak 20: 0.307532\\ &  &  &  &  & Kodak 21: 0.303464\\ &  &  &  &  & Kodak 22: 0.305068\\ &  &  &  &  & Kodak 23: 0.336737\\ &  &  &  &  & Kodak 24: 0.304921\\\hline\hline30 & MS-SSIM & 2.0 & 5x5deconv,2,4 & 5x5deconv,2,9 & Kodak 1: 0.095700\\ &  &  & 5x5deconv,2,20 & 5x5deconv,2,22 & Kodak 2: 0.100805\\ &  &  & 5x5deconv,2,320 & 5x5deconv,2,2 & Kodak 3: 0.102477\\ &  &  &  & 5x5deconv,2,3 & Kodak 4: 0.098977\\ &  &  &  &  & Kodak 5: 0.102099\\ &  &  &  &  & Kodak 6: 0.108808\\ &  &  &  &  & Kodak 7: 0.104401\\ &  &  &  &  & Kodak 8: 0.103192\\ &  &  &  &  & Kodak 9: 0.103093\\ &  &  &  &  & Kodak 10: 0.103565\\ &  &  &  &  & Kodak 11: 0.098944\\ &  &  &  &  & Kodak 12: 0.103324\\ &  &  &  &  & Kodak 13: 0.103918\\ &  &  &  &  & Kodak 14: 0.104337\\ &  &  &  &  & Kodak 15: 0.111203\\ &  &  &  &  & Kodak 16: 0.109747\\ &  &  &  &  & Kodak 17: 0.107238\\ &  &  &  &  & Kodak 18: 0.101940\\ &  &  &  &  & Kodak 19: 0.102568\\ &  &  &  &  & Kodak 20: 0.103878\\ &  &  &  &  & Kodak 21: 0.111197\\ &  &  &  &  & Kodak 22: 0.102089\\ &  &  &  &  & Kodak 23: 0.096628\\ &  &  &  &  & Kodak 24: 0.101162\\\hline\hline\hline\hline32 & MS-SSIM & 2.0 & 5x5deconv,2,246 & 5x5deconv,2,100 & Kodak 1: 0.172103\\ &  &  & 5x5deconv,2,176 & 5x5deconv,2,126 & Kodak 2: 0.158540\\ &  &  & 5x5deconv,2,320 & 5x5deconv,2,52 & Kodak 3: 0.161565\\ &  &  &  & 5x5deconv,2,3 & Kodak 4: 0.167513\\ &  &  &  &  & Kodak 5: 0.165571\\ &  &  &  &  & Kodak 6: 0.161807\\ &  &  &  &  & Kodak 7: 0.163902\\ &  &  &  &  & Kodak 8: 0.152826\\ &  &  &  &  & Kodak 9: 0.162120\\ &  &  &  &  & Kodak 10: 0.159618\\ &  &  &  &  & Kodak 11: 0.164069\\ &  &  &  &  & Kodak 12: 0.160986\\ &  &  &  &  & Kodak 13: 0.155940\\ &  &  &  &  & Kodak 14: 0.162848\\ &  &  &  &  & Kodak 15: 0.166172\\ &  &  &  &  & Kodak 16: 0.156546\\ &  &  &  &  & Kodak 17: 0.167898\\ &  &  &  &  & Kodak 18: 0.158738\\ &  &  &  &  & Kodak 19: 0.165188\\ &  &  &  &  & Kodak 20: 0.155985\\ &  &  &  &  & Kodak 21: 0.155443\\ &  &  &  &  & Kodak 22: 0.165359\\ &  &  &  &  & Kodak 23: 0.165800\\ &  &  &  &  & Kodak 24: 0.165839\\\hline\hline33 & MS-SSIM & 2.0 & 5x5deconv,2,10 & 5x5deconv,2,1 & Kodak 1: 0.094146\\ &  &  & 5x5deconv,2,10 & 5x5deconv,2,1 & Kodak 2: 0.098474\\ &  &  & 5x5deconv,2,320 & 5x5deconv,2,1 & Kodak 3: 0.106465\\ &  &  &  & 5x5deconv,2,3 & Kodak 4: 0.095766\\ &  &  &  &  & Kodak 5: 0.099317\\ &  &  &  &  & Kodak 6: 0.103362\\ &  &  &  &  & Kodak 7: 0.097627\\ &  &  &  &  & Kodak 8: 0.096831\\ &  &  &  &  & Kodak 9: 0.100116\\ &  &  &  &  & Kodak 10: 0.098857\\ &  &  &  &  & Kodak 11: 0.096697\\ &  &  &  &  & Kodak 12: 0.099205\\ &  &  &  &  & Kodak 13: 0.098910\\ &  &  &  &  & Kodak 14: 0.099549\\ &  &  &  &  & Kodak 15: 0.098334\\ &  &  &  &  & Kodak 16: 0.101492\\ &  &  &  &  & Kodak 17: 0.102995\\ &  &  &  &  & Kodak 18: 0.098339\\ &  &  &  &  & Kodak 19: 0.093178\\ &  &  &  &  & Kodak 20: 0.094932\\ &  &  &  &  & Kodak 21: 0.104312\\ &  &  &  &  & Kodak 22: 0.096392\\ &  &  &  &  & Kodak 23: 0.100495\\ &  &  &  &  & Kodak 24: 0.101436\\\hline\hline34 & MS-SSIM & 2.0 & 5x5deconv,2,453 & 5x5deconv,2,156 & Kodak 1: 0.224554\\ &  &  & 5x5deconv,2,196 & 5x5deconv,2,227 & Kodak 2: 0.230385\\ &  &  & 5x5deconv,2,320 & 5x5deconv,2,114 & Kodak 3: 0.231838\\ &  &  &  & 5x5deconv,2,3 & Kodak 4: 0.235153\\ &  &  &  &  & Kodak 5: 0.232829\\ &  &  &  &  & Kodak 6: 0.228153\\ &  &  &  &  & Kodak 7: 0.231279\\ &  &  &  &  & Kodak 8: 0.228096\\ &  &  &  &  & Kodak 9: 0.226661\\ &  &  &  &  & Kodak 10: 0.231350\\ &  &  &  &  & Kodak 11: 0.227499\\ &  &  &  &  & Kodak 12: 0.235399\\ &  &  &  &  & Kodak 13: 0.229262\\ &  &  &  &  & Kodak 14: 0.229895\\ &  &  &  &  & Kodak 15: 0.224272\\ &  &  &  &  & Kodak 16: 0.228603\\ &  &  &  &  & Kodak 17: 0.260105\\ &  &  &  &  & Kodak 18: 0.236837\\ &  &  &  &  & Kodak 19: 0.229217\\ &  &  &  &  & Kodak 20: 0.235670\\ &  &  &  &  & Kodak 21: 0.258421\\ &  &  &  &  & Kodak 22: 0.268734\\ &  &  &  &  & Kodak 23: 0.231796\\ &  &  &  &  & Kodak 24: 0.234190\\\hline\hline35 & MS-SSIM & 2.0 & 5x5deconv,2,44 & 5x5deconv,2,32 & Kodak 1: 0.105752\\ &  &  & 5x5deconv,2,25 & 5x5deconv,2,33 & Kodak 2: 0.111380\\ &  &  & 5x5deconv,2,320 & 5x5deconv,2,7 & Kodak 3: 0.109759\\ &  &  &  & 5x5deconv,2,3 & Kodak 4: 0.123373\\ &  &  &  &  & Kodak 5: 0.115546\\ &  &  &  &  & Kodak 6: 0.114466\\ &  &  &  &  & Kodak 7: 0.113416\\ &  &  &  &  & Kodak 8: 0.113003\\ &  &  &  &  & Kodak 9: 0.104442\\ &  &  &  &  & Kodak 10: 0.113626\\ &  &  &  &  & Kodak 11: 0.108919\\ &  &  &  &  & Kodak 12: 0.108002\\ &  &  &  &  & Kodak 13: 0.116355\\ &  &  &  &  & Kodak 14: 0.111757\\ &  &  &  &  & Kodak 15: 0.106473\\ &  &  &  &  & Kodak 16: 0.114290\\ &  &  &  &  & Kodak 17: 0.108663\\ &  &  &  &  & Kodak 18: 0.112271\\ &  &  &  &  & Kodak 19: 0.112997\\ &  &  &  &  & Kodak 20: 0.103612\\ &  &  &  &  & Kodak 21: 0.105884\\ &  &  &  &  & Kodak 22: 0.110382\\ &  &  &  &  & Kodak 23: 0.115561\\ &  &  &  &  & Kodak 24: 0.119853\\\hline\hline36 & MS-SSIM & 2.0 & 5x5deconv,2,10 & 5x5deconv,2,3 & Kodak 1: 0.091986\\ &  &  & 5x5deconv,2,10 & 5x5deconv,2,8 & Kodak 2: 0.095598\\ &  &  & 5x5deconv,2,320 & 5x5deconv,2,1 & Kodak 3: 0.098781\\ &  &  &  & 5x5deconv,2,3 & Kodak 4: 0.095738\\ &  &  &  &  & Kodak 5: 0.104407\\ &  &  &  &  & Kodak 6: 0.098547\\ &  &  &  &  & Kodak 7: 0.100792\\ &  &  &  &  & Kodak 8: 0.100579\\ &  &  &  &  & Kodak 9: 0.097855\\ &  &  &  &  & Kodak 10: 0.093657\\ &  &  &  &  & Kodak 11: 0.095556\\ &  &  &  &  & Kodak 12: 0.096876\\ &  &  &  &  & Kodak 13: 0.098435\\ &  &  &  &  & Kodak 14: 0.097199\\ &  &  &  &  & Kodak 15: 0.096454\\ &  &  &  &  & Kodak 16: 0.096775\\ &  &  &  &  & Kodak 17: 0.097100\\ &  &  &  &  & Kodak 18: 0.096444\\ &  &  &  &  & Kodak 19: 0.094706\\ &  &  &  &  & Kodak 20: 0.099763\\ &  &  &  &  & Kodak 21: 0.100020\\ &  &  &  &  & Kodak 22: 0.091234\\ &  &  &  &  & Kodak 23: 0.097246\\ &  &  &  &  & Kodak 24: 0.100853\\\hline\hline37 & MS-SSIM & 2.0 & 5x5deconv,2,110 & 5x5deconv,2,52 & Kodak 1: 0.133284\\ &  &  & 5x5deconv,2,91 & 5x5deconv,2,99 & Kodak 2: 0.136232\\ &  &  & 5x5deconv,2,320 & 5x5deconv,2,14 & Kodak 3: 0.126143\\ &  &  &  & 5x5deconv,2,3 & Kodak 4: 0.121492\\ &  &  &  &  & Kodak 5: 0.141129\\ &  &  &  &  & Kodak 6: 0.129047\\ &  &  &  &  & Kodak 7: 0.134381\\ &  &  &  &  & Kodak 8: 0.138610\\ &  &  &  &  & Kodak 9: 0.130280\\ &  &  &  &  & Kodak 10: 0.131644\\ &  &  &  &  & Kodak 11: 0.128826\\ &  &  &  &  & Kodak 12: 0.127354\\ &  &  &  &  & Kodak 13: 0.139635\\ &  &  &  &  & Kodak 14: 0.133237\\ &  &  &  &  & Kodak 15: 0.133940\\ &  &  &  &  & Kodak 16: 0.134307\\ &  &  &  &  & Kodak 17: 0.128295\\ &  &  &  &  & Kodak 18: 0.129377\\ &  &  &  &  & Kodak 19: 0.135881\\ &  &  &  &  & Kodak 20: 0.126141\\ &  &  &  &  & Kodak 21: 0.124948\\ &  &  &  &  & Kodak 22: 0.134730\\ &  &  &  &  & Kodak 23: 0.139666\\ &  &  &  &  & Kodak 24: 0.127464\\\hline\hline38 & MS-SSIM & 4.0 & 5x5deconv,2,10 & 5x5deconv,2,1 & Kodak 1: 0.090952\\ &  &  & 5x5deconv,2,10 & 5x5deconv,2,1 & Kodak 2: 0.096738\\ &  &  & 5x5deconv,2,320 & 5x5deconv,2,1 & Kodak 3: 0.095251\\ &  &  &  & 5x5deconv,2,3 & Kodak 4: 0.098782\\ &  &  &  &  & Kodak 5: 0.092690\\ &  &  &  &  & Kodak 6: 0.098315\\ &  &  &  &  & Kodak 7: 0.105282\\ &  &  &  &  & Kodak 8: 0.101947\\ &  &  &  &  & Kodak 9: 0.096050\\ &  &  &  &  & Kodak 10: 0.094927\\ &  &  &  &  & Kodak 11: 0.095138\\ &  &  &  &  & Kodak 12: 0.096854\\ &  &  &  &  & Kodak 13: 0.103976\\ &  &  &  &  & Kodak 14: 0.100366\\ &  &  &  &  & Kodak 15: 0.096226\\ &  &  &  &  & Kodak 16: 0.100781\\ &  &  &  &  & Kodak 17: 0.099065\\ &  &  &  &  & Kodak 18: 0.097624\\ &  &  &  &  & Kodak 19: 0.100249\\ &  &  &  &  & Kodak 20: 0.098001\\ &  &  &  &  & Kodak 21: 0.094369\\ &  &  &  &  & Kodak 22: 0.097500\\ &  &  &  &  & Kodak 23: 0.095584\\ &  &  &  &  & Kodak 24: 0.096745\\\hline\hline39 & MS-SSIM & 4.0 & 5x5deconv,2,10 & 5x5deconv,2,1 & Kodak 1: 0.090721\\ &  &  & 5x5deconv,2,10 & 5x5deconv,2,1 & Kodak 2: 0.096049\\ &  &  & 5x5deconv,2,320 & 5x5deconv,2,1 & Kodak 3: 0.104747\\ &  &  &  & 5x5deconv,2,3 & Kodak 4: 0.094713\\ &  &  &  &  & Kodak 5: 0.096903\\ &  &  &  &  & Kodak 6: 0.098670\\ &  &  &  &  & Kodak 7: 0.097385\\ &  &  &  &  & Kodak 8: 0.094880\\ &  &  &  &  & Kodak 9: 0.097602\\ &  &  &  &  & Kodak 10: 0.097897\\ &  &  &  &  & Kodak 11: 0.105028\\ &  &  &  &  & Kodak 12: 0.092849\\ &  &  &  &  & Kodak 13: 0.094995\\ &  &  &  &  & Kodak 14: 0.096379\\ &  &  &  &  & Kodak 15: 0.100212\\ &  &  &  &  & Kodak 16: 0.094847\\ &  &  &  &  & Kodak 17: 0.096808\\ &  &  &  &  & Kodak 18: 0.094814\\ &  &  &  &  & Kodak 19: 0.095993\\ &  &  &  &  & Kodak 20: 0.093081\\ &  &  &  &  & Kodak 21: 0.093864\\ &  &  &  &  & Kodak 22: 0.123309\\ &  &  &  &  & Kodak 23: 0.102927\\ &  &  &  &  & Kodak 24: 0.095088\\\hline\hline40 & MS-SSIM & 4.0 & 5x5deconv,2,10 & 5x5deconv,2,1 & Kodak 1: 0.091282\\ &  &  & 5x5deconv,2,10 & 5x5deconv,2,1 & Kodak 2: 0.098838\\ &  &  & 5x5deconv,2,320 & 5x5deconv,2,1 & Kodak 3: 0.096525\\ &  &  &  & 5x5deconv,2,3 & Kodak 4: 0.094476\\ &  &  &  &  & Kodak 5: 0.090632\\ &  &  &  &  & Kodak 6: 0.099037\\ &  &  &  &  & Kodak 7: 0.097025\\ &  &  &  &  & Kodak 8: 0.096776\\ &  &  &  &  & Kodak 9: 0.095166\\ &  &  &  &  & Kodak 10: 0.095837\\ &  &  &  &  & Kodak 11: 0.100132\\ &  &  &  &  & Kodak 12: 0.102244\\ &  &  &  &  & Kodak 13: 0.096330\\ &  &  &  &  & Kodak 14: 0.103137\\ &  &  &  &  & Kodak 15: 0.098987\\ &  &  &  &  & Kodak 16: 0.097792\\ &  &  &  &  & Kodak 17: 0.093968\\ &  &  &  &  & Kodak 18: 0.096898\\ &  &  &  &  & Kodak 19: 0.096596\\ &  &  &  &  & Kodak 20: 0.096429\\ &  &  &  &  & Kodak 21: 0.092776\\ &  &  &  &  & Kodak 22: 0.097026\\ &  &  &  &  & Kodak 23: 0.095822\\ &  &  &  &  & Kodak 24: 0.093343\\\hline\hline41 & MS-SSIM & 4.0 & 5x5deconv,2,75 & 5x5deconv,2,71 & Kodak 1: 0.125661\\ &  &  & 5x5deconv,2,65 & 5x5deconv,2,54 & Kodak 2: 0.130713\\ &  &  & 5x5deconv,2,320 & 5x5deconv,2,32 & Kodak 3: 0.127565\\ &  &  &  & 5x5deconv,2,3 & Kodak 4: 0.131184\\ &  &  &  &  & Kodak 5: 0.141488\\ &  &  &  &  & Kodak 6: 0.132865\\ &  &  &  &  & Kodak 7: 0.131176\\ &  &  &  &  & Kodak 8: 0.131162\\ &  &  &  &  & Kodak 9: 0.128955\\ &  &  &  &  & Kodak 10: 0.125191\\ &  &  &  &  & Kodak 11: 0.126054\\ &  &  &  &  & Kodak 12: 0.129388\\ &  &  &  &  & Kodak 13: 0.130984\\ &  &  &  &  & Kodak 14: 0.127012\\ &  &  &  &  & Kodak 15: 0.135156\\ &  &  &  &  & Kodak 16: 0.126891\\ &  &  &  &  & Kodak 17: 0.152366\\ &  &  &  &  & Kodak 18: 0.132795\\ &  &  &  &  & Kodak 19: 0.129301\\ &  &  &  &  & Kodak 20: 0.127178\\ &  &  &  &  & Kodak 21: 0.130082\\ &  &  &  &  & Kodak 22: 0.132800\\ &  &  &  &  & Kodak 23: 0.125170\\ &  &  &  &  & Kodak 24: 0.131402\\\hline\hline42 & MS-SSIM & 4.0 & 5x5deconv,2,155 & 5x5deconv,2,139 & Kodak 1: 0.153511\\ &  &  & 5x5deconv,2,127 & 5x5deconv,2,87 & Kodak 2: 0.171114\\ &  &  & 5x5deconv,2,320 & 5x5deconv,2,69 & Kodak 3: 0.156719\\ &  &  &  & 5x5deconv,2,3 & Kodak 4: 0.153876\\ &  &  &  &  & Kodak 5: 0.161439\\ &  &  &  &  & Kodak 6: 0.158156\\ &  &  &  &  & Kodak 7: 0.161088\\ &  &  &  &  & Kodak 8: 0.156548\\ &  &  &  &  & Kodak 9: 0.162941\\ &  &  &  &  & Kodak 10: 0.160336\\ &  &  &  &  & Kodak 11: 0.157832\\ &  &  &  &  & Kodak 12: 0.161245\\ &  &  &  &  & Kodak 13: 0.157804\\ &  &  &  &  & Kodak 14: 0.163971\\ &  &  &  &  & Kodak 15: 0.158929\\ &  &  &  &  & Kodak 16: 0.162222\\ &  &  &  &  & Kodak 17: 0.159790\\ &  &  &  &  & Kodak 18: 0.171330\\ &  &  &  &  & Kodak 19: 0.164128\\ &  &  &  &  & Kodak 20: 0.159060\\ &  &  &  &  & Kodak 21: 0.164238\\ &  &  &  &  & Kodak 22: 0.152252\\ &  &  &  &  & Kodak 23: 0.162047\\ &  &  &  &  & Kodak 24: 0.156580\\\hline\hline43 & MS-SSIM & 4.0 & 5x5deconv,2,10 & 5x5deconv,2,7 & Kodak 1: 0.095319\\ &  &  & 5x5deconv,2,10 & 5x5deconv,2,11 & Kodak 2: 0.100039\\ &  &  & 5x5deconv,2,320 & 5x5deconv,2,1 & Kodak 3: 0.096868\\ &  &  &  & 5x5deconv,2,3 & Kodak 4: 0.100166\\ &  &  &  &  & Kodak 5: 0.096320\\ &  &  &  &  & Kodak 6: 0.100694\\ &  &  &  &  & Kodak 7: 0.099020\\ &  &  &  &  & Kodak 8: 0.098841\\ &  &  &  &  & Kodak 9: 0.100093\\ &  &  &  &  & Kodak 10: 0.100592\\ &  &  &  &  & Kodak 11: 0.102196\\ &  &  &  &  & Kodak 12: 0.096933\\ &  &  &  &  & Kodak 13: 0.102560\\ &  &  &  &  & Kodak 14: 0.098009\\ &  &  &  &  & Kodak 15: 0.098994\\ &  &  &  &  & Kodak 16: 0.101342\\ &  &  &  &  & Kodak 17: 0.122370\\ &  &  &  &  & Kodak 18: 0.097982\\ &  &  &  &  & Kodak 19: 0.105008\\ &  &  &  &  & Kodak 20: 0.100320\\ &  &  &  &  & Kodak 21: 0.096663\\ &  &  &  &  & Kodak 22: 0.100630\\ &  &  &  &  & Kodak 23: 0.095795\\ &  &  &  &  & Kodak 24: 0.098263\\\hline\hline44 & MS-SSIM & 4.0 & 5x5deconv,2,4 & 5x5deconv,2,11 & Kodak 1: 0.102058\\ &  &  & 5x5deconv,2,22 & 5x5deconv,2,18 & Kodak 2: 0.105419\\ &  &  & 5x5deconv,2,320 & 5x5deconv,2,3 & Kodak 3: 0.107916\\ &  &  &  & 5x5deconv,2,3 & Kodak 4: 0.113027\\ &  &  &  &  & Kodak 5: 0.099606\\ &  &  &  &  & Kodak 6: 0.098894\\ &  &  &  &  & Kodak 7: 0.109882\\ &  &  &  &  & Kodak 8: 0.101118\\ &  &  &  &  & Kodak 9: 0.104975\\ &  &  &  &  & Kodak 10: 0.103633\\ &  &  &  &  & Kodak 11: 0.106851\\ &  &  &  &  & Kodak 12: 0.103239\\ &  &  &  &  & Kodak 13: 0.098100\\ &  &  &  &  & Kodak 14: 0.103297\\ &  &  &  &  & Kodak 15: 0.096719\\ &  &  &  &  & Kodak 16: 0.104902\\ &  &  &  &  & Kodak 17: 0.104119\\ &  &  &  &  & Kodak 18: 0.105919\\ &  &  &  &  & Kodak 19: 0.108194\\ &  &  &  &  & Kodak 20: 0.100576\\ &  &  &  &  & Kodak 21: 0.100738\\ &  &  &  &  & Kodak 22: 0.101734\\ &  &  &  &  & Kodak 23: 0.105508\\ &  &  &  &  & Kodak 24: 0.101128\\\hline\hline45 & MS-SSIM & 4.0 & 5x5deconv,2,10 & 5x5deconv,2,1 & Kodak 1: 0.089756\\ &  &  & 5x5deconv,2,10 & 5x5deconv,2,1 & Kodak 2: 0.103679\\ &  &  & 5x5deconv,2,320 & 5x5deconv,2,1 & Kodak 3: 0.101468\\ &  &  &  & 5x5deconv,2,3 & Kodak 4: 0.096757\\ &  &  &  &  & Kodak 5: 0.095611\\ &  &  &  &  & Kodak 6: 0.094675\\ &  &  &  &  & Kodak 7: 0.096232\\ &  &  &  &  & Kodak 8: 0.093652\\ &  &  &  &  & Kodak 9: 0.098824\\ &  &  &  &  & Kodak 10: 0.096499\\ &  &  &  &  & Kodak 11: 0.099287\\ &  &  &  &  & Kodak 12: 0.097293\\ &  &  &  &  & Kodak 13: 0.097140\\ &  &  &  &  & Kodak 14: 0.096376\\ &  &  &  &  & Kodak 15: 0.094554\\ &  &  &  &  & Kodak 16: 0.095840\\ &  &  &  &  & Kodak 17: 0.094880\\ &  &  &  &  & Kodak 18: 0.094884\\ &  &  &  &  & Kodak 19: 0.095404\\ &  &  &  &  & Kodak 20: 0.094912\\ &  &  &  &  & Kodak 21: 0.089556\\ &  &  &  &  & Kodak 22: 0.095033\\ &  &  &  &  & Kodak 23: 0.097846\\ &  &  &  &  & Kodak 24: 0.092783\\\hline\hline46 & MS-SSIM & 4.0 & 5x5deconv,2,10 & 5x5deconv,2,1 & Kodak 1: 0.093717\\ &  &  & 5x5deconv,2,10 & 5x5deconv,2,1 & Kodak 2: 0.093685\\ &  &  & 5x5deconv,2,320 & 5x5deconv,2,1 & Kodak 3: 0.095882\\ &  &  &  & 5x5deconv,2,3 & Kodak 4: 0.100249\\ &  &  &  &  & Kodak 5: 0.092320\\ &  &  &  &  & Kodak 6: 0.099253\\ &  &  &  &  & Kodak 7: 0.102089\\ &  &  &  &  & Kodak 8: 0.098631\\ &  &  &  &  & Kodak 9: 0.096134\\ &  &  &  &  & Kodak 10: 0.096086\\ &  &  &  &  & Kodak 11: 0.096263\\ &  &  &  &  & Kodak 12: 0.096489\\ &  &  &  &  & Kodak 13: 0.096970\\ &  &  &  &  & Kodak 14: 0.096868\\ &  &  &  &  & Kodak 15: 0.099859\\ &  &  &  &  & Kodak 16: 0.096379\\ &  &  &  &  & Kodak 17: 0.098542\\ &  &  &  &  & Kodak 18: 0.094877\\ &  &  &  &  & Kodak 19: 0.096080\\ &  &  &  &  & Kodak 20: 0.095314\\ &  &  &  &  & Kodak 21: 0.097499\\ &  &  &  &  & Kodak 22: 0.092755\\ &  &  &  &  & Kodak 23: 0.098640\\ &  &  &  &  & Kodak 24: 0.097917\\\hline\hline47 & MS-SSIM & 4.0 & 5x5deconv,2,360 & 5x5deconv,2,213 & Kodak 1: 0.217038\\ &  &  & 5x5deconv,2,167 & 5x5deconv,2,158 & Kodak 2: 0.214989\\ &  &  & 5x5deconv,2,320 & 5x5deconv,2,116 & Kodak 3: 0.212440\\ &  &  &  & 5x5deconv,2,3 & Kodak 4: 0.216266\\ &  &  &  &  & Kodak 5: 0.223473\\ &  &  &  &  & Kodak 6: 0.214093\\ &  &  &  &  & Kodak 7: 0.211378\\ &  &  &  &  & Kodak 8: 0.222914\\ &  &  &  &  & Kodak 9: 0.210782\\ &  &  &  &  & Kodak 10: 0.217579\\ &  &  &  &  & Kodak 11: 0.219613\\ &  &  &  &  & Kodak 12: 0.223588\\ &  &  &  &  & Kodak 13: 0.215721\\ &  &  &  &  & Kodak 14: 0.209539\\ &  &  &  &  & Kodak 15: 0.215554\\ &  &  &  &  & Kodak 16: 0.209600\\ &  &  &  &  & Kodak 17: 0.208878\\ &  &  &  &  & Kodak 18: 0.211996\\ &  &  &  &  & Kodak 19: 0.211284\\ &  &  &  &  & Kodak 20: 0.215736\\ &  &  &  &  & Kodak 21: 0.233208\\ &  &  &  &  & Kodak 22: 0.215157\\ &  &  &  &  & Kodak 23: 0.209401\\ &  &  &  &  & Kodak 24: 0.217229\\\hline\hline48 & MS-SSIM & 4.0 & 5x5deconv,2,36 & 5x5deconv,2,36 & Kodak 1: 0.107691\\ &  &  & 5x5deconv,2,22 & 5x5deconv,2,36 & Kodak 2: 0.112825\\ &  &  & 5x5deconv,2,320 & 5x5deconv,2,8 & Kodak 3: 0.111096\\ &  &  &  & 5x5deconv,2,3 & Kodak 4: 0.114116\\ &  &  &  &  & Kodak 5: 0.114587\\ &  &  &  &  & Kodak 6: 0.111780\\ &  &  &  &  & Kodak 7: 0.111388\\ &  &  &  &  & Kodak 8: 0.114358\\ &  &  &  &  & Kodak 9: 0.115126\\ &  &  &  &  & Kodak 10: 0.113175\\ &  &  &  &  & Kodak 11: 0.111771\\ &  &  &  &  & Kodak 12: 0.110345\\ &  &  &  &  & Kodak 13: 0.114550\\ &  &  &  &  & Kodak 14: 0.110107\\ &  &  &  &  & Kodak 15: 0.109042\\ &  &  &  &  & Kodak 16: 0.105278\\ &  &  &  &  & Kodak 17: 0.105448\\ &  &  &  &  & Kodak 18: 0.113519\\ &  &  &  &  & Kodak 19: 0.102514\\ &  &  &  &  & Kodak 20: 0.107083\\ &  &  &  &  & Kodak 21: 0.107819\\ &  &  &  &  & Kodak 22: 0.114666\\ &  &  &  &  & Kodak 23: 0.105379\\ &  &  &  &  & Kodak 24: 0.108683\\\hline\hline49 & MS-SSIM & 4.0 & 5x5deconv,2,163 & 5x5deconv,2,261 & Kodak 1: 0.270358\\ &  &  & 5x5deconv,2,232 & 5x5deconv,2,191 & Kodak 2: 0.260065\\ &  &  & 5x5deconv,2,320 & 5x5deconv,2,157 & Kodak 3: 0.266279\\ &  &  &  & 5x5deconv,2,3 & Kodak 4: 0.266715\\ &  &  &  &  & Kodak 5: 0.268397\\ &  &  &  &  & Kodak 6: 0.296003\\ &  &  &  &  & Kodak 7: 0.270939\\ &  &  &  &  & Kodak 8: 0.272363\\ &  &  &  &  & Kodak 9: 0.282898\\ &  &  &  &  & Kodak 10: 0.276239\\ &  &  &  &  & Kodak 11: 0.275468\\ &  &  &  &  & Kodak 12: 0.276066\\ &  &  &  &  & Kodak 13: 0.274694\\ &  &  &  &  & Kodak 14: 0.274352\\ &  &  &  &  & Kodak 15: 0.291074\\ &  &  &  &  & Kodak 16: 0.284149\\ &  &  &  &  & Kodak 17: 0.266388\\ &  &  &  &  & Kodak 18: 0.265844\\ &  &  &  &  & Kodak 19: 0.272497\\ &  &  &  &  & Kodak 20: 0.258171\\ &  &  &  &  & Kodak 21: 0.264063\\ &  &  &  &  & Kodak 22: 0.264222\\ &  &  &  &  & Kodak 23: 0.266410\\ &  &  &  &  & Kodak 24: 0.268127\\\hline\hline50 & MS-SSIM & 4.0 & 5x5deconv,2,80 & 5x5deconv,2,47 & Kodak 1: 0.119606\\ &  &  & 5x5deconv,2,34 & 5x5deconv,2,35 & Kodak 2: 0.128004\\ &  &  & 5x5deconv,2,320 & 5x5deconv,2,14 & Kodak 3: 0.138757\\ &  &  &  & 5x5deconv,2,3 & Kodak 4: 0.127672\\ &  &  &  &  & Kodak 5: 0.125565\\ &  &  &  &  & Kodak 6: 0.126440\\ &  &  &  &  & Kodak 7: 0.132676\\ &  &  &  &  & Kodak 8: 0.128505\\ &  &  &  &  & Kodak 9: 0.121650\\ &  &  &  &  & Kodak 10: 0.132925\\ &  &  &  &  & Kodak 11: 0.126584\\ &  &  &  &  & Kodak 12: 0.140687\\ &  &  &  &  & Kodak 13: 0.125284\\ &  &  &  &  & Kodak 14: 0.123980\\ &  &  &  &  & Kodak 15: 0.134480\\ &  &  &  &  & Kodak 16: 0.118036\\ &  &  &  &  & Kodak 17: 0.128416\\ &  &  &  &  & Kodak 18: 0.132844\\ &  &  &  &  & Kodak 19: 0.122069\\ &  &  &  &  & Kodak 20: 0.136086\\ &  &  &  &  & Kodak 21: 0.130614\\ &  &  &  &  & Kodak 22: 0.123697\\ &  &  &  &  & Kodak 23: 0.117460\\ &  &  &  &  & Kodak 24: 0.126308\\\hline\hline51 & MS-SSIM & 16.0 & 5x5deconv,2,4 & 5x5deconv,2,18 & Kodak 1: 0.114585\\ &  &  & 5x5deconv,2,18 & 5x5deconv,2,19 & Kodak 2: 0.113837\\ &  &  & 5x5deconv,2,320 & 5x5deconv,2,8 & Kodak 3: 0.104816\\ &  &  &  & 5x5deconv,2,3 & Kodak 4: 0.104795\\ &  &  &  &  & Kodak 5: 0.111883\\ &  &  &  &  & Kodak 6: 0.107163\\ &  &  &  &  & Kodak 7: 0.114111\\ &  &  &  &  & Kodak 8: 0.106197\\ &  &  &  &  & Kodak 9: 0.105768\\ &  &  &  &  & Kodak 10: 0.112407\\ &  &  &  &  & Kodak 11: 0.113238\\ &  &  &  &  & Kodak 12: 0.113798\\ &  &  &  &  & Kodak 13: 0.127488\\ &  &  &  &  & Kodak 14: 0.117467\\ &  &  &  &  & Kodak 15: 0.116409\\ &  &  &  &  & Kodak 16: 0.108907\\ &  &  &  &  & Kodak 17: 0.105660\\ &  &  &  &  & Kodak 18: 0.113198\\ &  &  &  &  & Kodak 19: 0.126659\\ &  &  &  &  & Kodak 20: 0.105179\\ &  &  &  &  & Kodak 21: 0.109745\\ &  &  &  &  & Kodak 22: 0.119926\\ &  &  &  &  & Kodak 23: 0.119268\\ &  &  &  &  & Kodak 24: 0.109576\\\hline\hline52 & MS-SSIM & 16.0 & 5x5deconv,2,10 & 5x5deconv,2,9 & Kodak 1: 0.094720\\ &  &  & 5x5deconv,2,10 & 5x5deconv,2,9 & Kodak 2: 0.100007\\ &  &  & 5x5deconv,2,320 & 5x5deconv,2,2 & Kodak 3: 0.101630\\ &  &  &  & 5x5deconv,2,3 & Kodak 4: 0.102407\\ &  &  &  &  & Kodak 5: 0.104647\\ &  &  &  &  & Kodak 6: 0.100795\\ &  &  &  &  & Kodak 7: 0.096077\\ &  &  &  &  & Kodak 8: 0.105263\\ &  &  &  &  & Kodak 9: 0.103203\\ &  &  &  &  & Kodak 10: 0.107039\\ &  &  &  &  & Kodak 11: 0.106043\\ &  &  &  &  & Kodak 12: 0.107274\\ &  &  &  &  & Kodak 13: 0.101607\\ &  &  &  &  & Kodak 14: 0.097588\\ &  &  &  &  & Kodak 15: 0.102957\\ &  &  &  &  & Kodak 16: 0.101659\\ &  &  &  &  & Kodak 17: 0.113951\\ &  &  &  &  & Kodak 18: 0.112005\\ &  &  &  &  & Kodak 19: 0.104945\\ &  &  &  &  & Kodak 20: 0.110589\\ &  &  &  &  & Kodak 21: 0.101707\\ &  &  &  &  & Kodak 22: 0.110540\\ &  &  &  &  & Kodak 23: 0.100459\\ &  &  &  &  & Kodak 24: 0.112476\\\hline\hline53 & MS-SSIM & 16.0 & 5x5deconv,2,126 & 5x5deconv,2,232 & Kodak 1: 0.238154\\ &  &  & 5x5deconv,2,186 & 5x5deconv,2,109 & Kodak 2: 0.215953\\ &  &  & 5x5deconv,2,320 & 5x5deconv,2,130 & Kodak 3: 0.203700\\ &  &  &  & 5x5deconv,2,3 & Kodak 4: 0.202846\\ &  &  &  &  & Kodak 5: 0.202394\\ &  &  &  &  & Kodak 6: 0.202295\\ &  &  &  &  & Kodak 7: 0.214188\\ &  &  &  &  & Kodak 8: 0.216370\\ &  &  &  &  & Kodak 9: 0.211758\\ &  &  &  &  & Kodak 10: 0.238991\\ &  &  &  &  & Kodak 11: 0.215912\\ &  &  &  &  & Kodak 12: 0.204758\\ &  &  &  &  & Kodak 13: 0.209270\\ &  &  &  &  & Kodak 14: 0.213734\\ &  &  &  &  & Kodak 15: 0.206845\\ &  &  &  &  & Kodak 16: 0.206379\\ &  &  &  &  & Kodak 17: 0.230254\\ &  &  &  &  & Kodak 18: 0.212157\\ &  &  &  &  & Kodak 19: 0.210962\\ &  &  &  &  & Kodak 20: 0.216503\\ &  &  &  &  & Kodak 21: 0.215664\\ &  &  &  &  & Kodak 22: 0.211320\\ &  &  &  &  & Kodak 23: 0.207184\\ &  &  &  &  & Kodak 24: 0.219555\\\hline\hline54 & MS-SSIM & 16.0 & 5x5deconv,2,130 & 5x5deconv,2,298 & Kodak 1: 0.281146\\ &  &  & 5x5deconv,2,212 & 5x5deconv,2,158 & Kodak 2: 0.258591\\ &  &  & 5x5deconv,2,320 & 5x5deconv,2,165 & Kodak 3: 0.260087\\ &  &  &  & 5x5deconv,2,3 & Kodak 4: 0.259938\\ &  &  &  &  & Kodak 5: 0.258895\\ &  &  &  &  & Kodak 6: 0.288931\\ &  &  &  &  & Kodak 7: 0.260562\\ &  &  &  &  & Kodak 8: 0.263448\\ &  &  &  &  & Kodak 9: 0.258166\\ &  &  &  &  & Kodak 10: 0.259182\\ &  &  &  &  & Kodak 11: 0.253944\\ &  &  &  &  & Kodak 12: 0.284203\\ &  &  &  &  & Kodak 13: 0.261948\\ &  &  &  &  & Kodak 14: 0.257399\\ &  &  &  &  & Kodak 15: 0.263067\\ &  &  &  &  & Kodak 16: 0.259560\\ &  &  &  &  & Kodak 17: 0.290846\\ &  &  &  &  & Kodak 18: 0.260965\\ &  &  &  &  & Kodak 19: 0.269702\\ &  &  &  &  & Kodak 20: 0.272157\\ &  &  &  &  & Kodak 21: 0.309641\\ &  &  &  &  & Kodak 22: 0.258078\\ &  &  &  &  & Kodak 23: 0.260026\\ &  &  &  &  & Kodak 24: 0.257808\\\hline\hline55 & MS-SSIM & 16.0 & 5x5deconv,2,30 & 5x5deconv,2,109 & Kodak 1: 0.139251\\ &  &  & 5x5deconv,2,51 & 5x5deconv,2,36 & Kodak 2: 0.133528\\ &  &  & 5x5deconv,2,320 & 5x5deconv,2,37 & Kodak 3: 0.140749\\ &  &  &  & 5x5deconv,2,3 & Kodak 4: 0.136051\\ &  &  &  &  & Kodak 5: 0.134860\\ &  &  &  &  & Kodak 6: 0.134172\\ &  &  &  &  & Kodak 7: 0.139721\\ &  &  &  &  & Kodak 8: 0.134780\\ &  &  &  &  & Kodak 9: 0.137690\\ &  &  &  &  & Kodak 10: 0.135880\\ &  &  &  &  & Kodak 11: 0.133254\\ &  &  &  &  & Kodak 12: 0.132106\\ &  &  &  &  & Kodak 13: 0.139968\\ &  &  &  &  & Kodak 14: 0.137579\\ &  &  &  &  & Kodak 15: 0.132463\\ &  &  &  &  & Kodak 16: 0.129214\\ &  &  &  &  & Kodak 17: 0.147135\\ &  &  &  &  & Kodak 18: 0.136931\\ &  &  &  &  & Kodak 19: 0.156046\\ &  &  &  &  & Kodak 20: 0.128119\\ &  &  &  &  & Kodak 21: 0.132729\\ &  &  &  &  & Kodak 22: 0.130668\\ &  &  &  &  & Kodak 23: 0.143981\\ &  &  &  &  & Kodak 24: 0.140562\\\hline\hline56 & MS-SSIM & 16.0 & 5x5deconv,2,96 & 5x5deconv,2,153 & Kodak 1: 0.183450\\ &  &  & 5x5deconv,2,79 & 5x5deconv,2,66 & Kodak 2: 0.165753\\ &  &  & 5x5deconv,2,320 & 5x5deconv,2,77 & Kodak 3: 0.166738\\ &  &  &  & 5x5deconv,2,3 & Kodak 4: 0.167160\\ &  &  &  &  & Kodak 5: 0.167853\\ &  &  &  &  & Kodak 6: 0.165152\\ &  &  &  &  & Kodak 7: 0.164976\\ &  &  &  &  & Kodak 8: 0.169834\\ &  &  &  &  & Kodak 9: 0.161676\\ &  &  &  &  & Kodak 10: 0.160097\\ &  &  &  &  & Kodak 11: 0.177481\\ &  &  &  &  & Kodak 12: 0.162321\\ &  &  &  &  & Kodak 13: 0.175344\\ &  &  &  &  & Kodak 14: 0.176639\\ &  &  &  &  & Kodak 15: 0.162777\\ &  &  &  &  & Kodak 16: 0.167409\\ &  &  &  &  & Kodak 17: 0.183024\\ &  &  &  &  & Kodak 18: 0.158568\\ &  &  &  &  & Kodak 19: 0.160592\\ &  &  &  &  & Kodak 20: 0.169114\\ &  &  &  &  & Kodak 21: 0.182446\\ &  &  &  &  & Kodak 22: 0.163670\\ &  &  &  &  & Kodak 23: 0.167540\\ &  &  &  &  & Kodak 24: 0.163309\\\hline\hline57 & MS-SSIM & 16.0 & 5x5deconv,2,10 & 5x5deconv,2,1 & Kodak 1: 0.090449\\ &  &  & 5x5deconv,2,10 & 5x5deconv,2,1 & Kodak 2: 0.100087\\ &  &  & 5x5deconv,2,320 & 5x5deconv,2,1 & Kodak 3: 0.104756\\ &  &  &  & 5x5deconv,2,3 & Kodak 4: 0.100550\\ &  &  &  &  & Kodak 5: 0.105024\\ &  &  &  &  & Kodak 6: 0.098192\\ &  &  &  &  & Kodak 7: 0.105486\\ &  &  &  &  & Kodak 8: 0.104733\\ &  &  &  &  & Kodak 9: 0.101347\\ &  &  &  &  & Kodak 10: 0.109711\\ &  &  &  &  & Kodak 11: 0.106180\\ &  &  &  &  & Kodak 12: 0.098015\\ &  &  &  &  & Kodak 13: 0.107539\\ &  &  &  &  & Kodak 14: 0.099377\\ &  &  &  &  & Kodak 15: 0.095486\\ &  &  &  &  & Kodak 16: 0.105926\\ &  &  &  &  & Kodak 17: 0.100554\\ &  &  &  &  & Kodak 18: 0.098241\\ &  &  &  &  & Kodak 19: 0.099004\\ &  &  &  &  & Kodak 20: 0.101968\\ &  &  &  &  & Kodak 21: 0.108133\\ &  &  &  &  & Kodak 22: 0.098346\\ &  &  &  &  & Kodak 23: 0.098716\\ &  &  &  &  & Kodak 24: 0.105353\\\hline\hline58 & MS-SSIM & 16.0 & 5x5deconv,2,130 & 5x5deconv,2,306 & Kodak 1: 0.288659\\ &  &  & 5x5deconv,2,214 & 5x5deconv,2,156 & Kodak 2: 0.259102\\ &  &  & 5x5deconv,2,320 & 5x5deconv,2,167 & Kodak 3: 0.260490\\ &  &  &  & 5x5deconv,2,3 & Kodak 4: 0.257623\\ &  &  &  &  & Kodak 5: 0.261322\\ &  &  &  &  & Kodak 6: 0.259203\\ &  &  &  &  & Kodak 7: 0.251763\\ &  &  &  &  & Kodak 8: 0.258299\\ &  &  &  &  & Kodak 9: 0.257596\\ &  &  &  &  & Kodak 10: 0.257118\\ &  &  &  &  & Kodak 11: 0.291929\\ &  &  &  &  & Kodak 12: 0.252634\\ &  &  &  &  & Kodak 13: 0.268473\\ &  &  &  &  & Kodak 14: 0.258791\\ &  &  &  &  & Kodak 15: 0.253297\\ &  &  &  &  & Kodak 16: 0.254196\\ &  &  &  &  & Kodak 17: 0.256524\\ &  &  &  &  & Kodak 18: 0.254386\\ &  &  &  &  & Kodak 19: 0.293254\\ &  &  &  &  & Kodak 20: 0.258244\\ &  &  &  &  & Kodak 21: 0.257840\\ &  &  &  &  & Kodak 22: 0.293909\\ &  &  &  &  & Kodak 23: 0.254578\\ &  &  &  &  & Kodak 24: 0.260392\\\hline\hline59 & MS-SSIM & 16.0 & 5x5deconv,2,22 & 5x5deconv,2,57 & Kodak 1: 0.125404\\ &  &  & 5x5deconv,2,35 & 5x5deconv,2,19 & Kodak 2: 0.127863\\ &  &  & 5x5deconv,2,320 & 5x5deconv,2,22 & Kodak 3: 0.121917\\ &  &  &  & 5x5deconv,2,3 & Kodak 4: 0.124976\\ &  &  &  &  & Kodak 5: 0.121839\\ &  &  &  &  & Kodak 6: 0.121986\\ &  &  &  &  & Kodak 7: 0.118249\\ &  &  &  &  & Kodak 8: 0.119982\\ &  &  &  &  & Kodak 9: 0.120682\\ &  &  &  &  & Kodak 10: 0.114607\\ &  &  &  &  & Kodak 11: 0.123187\\ &  &  &  &  & Kodak 12: 0.130364\\ &  &  &  &  & Kodak 13: 0.130266\\ &  &  &  &  & Kodak 14: 0.133495\\ &  &  &  &  & Kodak 15: 0.125459\\ &  &  &  &  & Kodak 16: 0.117762\\ &  &  &  &  & Kodak 17: 0.120776\\ &  &  &  &  & Kodak 18: 0.120149\\ &  &  &  &  & Kodak 19: 0.128455\\ &  &  &  &  & Kodak 20: 0.129218\\ &  &  &  &  & Kodak 21: 0.124082\\ &  &  &  &  & Kodak 22: 0.130486\\ &  &  &  &  & Kodak 23: 0.128145\\ &  &  &  &  & Kodak 24: 0.140525\\\hline\hline60 & MS-SSIM & 16.0 & 5x5deconv,2,10 & 5x5deconv,2,1 & Kodak 1: 0.101804\\ &  &  & 5x5deconv,2,10 & 5x5deconv,2,1 & Kodak 2: 0.098631\\ &  &  & 5x5deconv,2,320 & 5x5deconv,2,1 & Kodak 3: 0.103845\\ &  &  &  & 5x5deconv,2,3 & Kodak 4: 0.104627\\ &  &  &  &  & Kodak 5: 0.097252\\ &  &  &  &  & Kodak 6: 0.098630\\ &  &  &  &  & Kodak 7: 0.097946\\ &  &  &  &  & Kodak 8: 0.098765\\ &  &  &  &  & Kodak 9: 0.098010\\ &  &  &  &  & Kodak 10: 0.097327\\ &  &  &  &  & Kodak 11: 0.103509\\ &  &  &  &  & Kodak 12: 0.100254\\ &  &  &  &  & Kodak 13: 0.102144\\ &  &  &  &  & Kodak 14: 0.099012\\ &  &  &  &  & Kodak 15: 0.106980\\ &  &  &  &  & Kodak 16: 0.105509\\ &  &  &  &  & Kodak 17: 0.100954\\ &  &  &  &  & Kodak 18: 0.104374\\ &  &  &  &  & Kodak 19: 0.098069\\ &  &  &  &  & Kodak 20: 0.105693\\ &  &  &  &  & Kodak 21: 0.101235\\ &  &  &  &  & Kodak 22: 0.098572\\ &  &  &  &  & Kodak 23: 0.105020\\ &  &  &  &  & Kodak 24: 0.097105\\\hline\hline61 & MS-SSIM & 16.0 & 5x5deconv,2,10 & 5x5deconv,2,1 & Kodak 1: 0.091660\\ &  &  & 5x5deconv,2,10 & 5x5deconv,2,1 & Kodak 2: 0.096338\\ &  &  & 5x5deconv,2,320 & 5x5deconv,2,1 & Kodak 3: 0.095996\\ &  &  &  & 5x5deconv,2,3 & Kodak 4: 0.099211\\ &  &  &  &  & Kodak 5: 0.096682\\ &  &  &  &  & Kodak 6: 0.099324\\ &  &  &  &  & Kodak 7: 0.108493\\ &  &  &  &  & Kodak 8: 0.099608\\ &  &  &  &  & Kodak 9: 0.097639\\ &  &  &  &  & Kodak 10: 0.096301\\ &  &  &  &  & Kodak 11: 0.100298\\ &  &  &  &  & Kodak 12: 0.098497\\ &  &  &  &  & Kodak 13: 0.096368\\ &  &  &  &  & Kodak 14: 0.110839\\ &  &  &  &  & Kodak 15: 0.098789\\ &  &  &  &  & Kodak 16: 0.102690\\ &  &  &  &  & Kodak 17: 0.103154\\ &  &  &  &  & Kodak 18: 0.099768\\ &  &  &  &  & Kodak 19: 0.098993\\ &  &  &  &  & Kodak 20: 0.095909\\ &  &  &  &  & Kodak 21: 0.097948\\ &  &  &  &  & Kodak 22: 0.096138\\ &  &  &  &  & Kodak 23: 0.103601\\ &  &  &  &  & Kodak 24: 0.097320\\\hline\hline62 & MS-SSIM & 16.0 & 5x5deconv,2,10 & 5x5deconv,2,1 & Kodak 1: 0.100930\\ &  &  & 5x5deconv,2,10 & 5x5deconv,2,4 & Kodak 2: 0.102611\\ &  &  & 5x5deconv,2,320 & 5x5deconv,2,1 & Kodak 3: 0.096534\\ &  &  &  & 5x5deconv,2,3 & Kodak 4: 0.108102\\ &  &  &  &  & Kodak 5: 0.098892\\ &  &  &  &  & Kodak 6: 0.098748\\ &  &  &  &  & Kodak 7: 0.102026\\ &  &  &  &  & Kodak 8: 0.099028\\ &  &  &  &  & Kodak 9: 0.102581\\ &  &  &  &  & Kodak 10: 0.095513\\ &  &  &  &  & Kodak 11: 0.095084\\ &  &  &  &  & Kodak 12: 0.097331\\ &  &  &  &  & Kodak 13: 0.096094\\ &  &  &  &  & Kodak 14: 0.100267\\ &  &  &  &  & Kodak 15: 0.100992\\ &  &  &  &  & Kodak 16: 0.097086\\ &  &  &  &  & Kodak 17: 0.103211\\ &  &  &  &  & Kodak 18: 0.099233\\ &  &  &  &  & Kodak 19: 0.105211\\ &  &  &  &  & Kodak 20: 0.096477\\ &  &  &  &  & Kodak 21: 0.094542\\ &  &  &  &  & Kodak 22: 0.101323\\ &  &  &  &  & Kodak 23: 0.096402\\ &  &  &  &  & Kodak 24: 0.094841\\\hline\hline63 & MS-SSIM & 16.0 & 5x5deconv,2,10 & 5x5deconv,2,1 & Kodak 1: 0.093616\\ &  &  & 5x5deconv,2,10 & 5x5deconv,2,1 & Kodak 2: 0.099860\\ &  &  & 5x5deconv,2,320 & 5x5deconv,2,1 & Kodak 3: 0.098776\\ &  &  &  & 5x5deconv,2,3 & Kodak 4: 0.099355\\ &  &  &  &  & Kodak 5: 0.094526\\ &  &  &  &  & Kodak 6: 0.100718\\ &  &  &  &  & Kodak 7: 0.103188\\ &  &  &  &  & Kodak 8: 0.099156\\ &  &  &  &  & Kodak 9: 0.100436\\ &  &  &  &  & Kodak 10: 0.095387\\ &  &  &  &  & Kodak 11: 0.094490\\ &  &  &  &  & Kodak 12: 0.107202\\ &  &  &  &  & Kodak 13: 0.097424\\ &  &  &  &  & Kodak 14: 0.103278\\ &  &  &  &  & Kodak 15: 0.101626\\ &  &  &  &  & Kodak 16: 0.095700\\ &  &  &  &  & Kodak 17: 0.097334\\ &  &  &  &  & Kodak 18: 0.100427\\ &  &  &  &  & Kodak 19: 0.096982\\ &  &  &  &  & Kodak 20: 0.095711\\ &  &  &  &  & Kodak 21: 0.098819\\ &  &  &  &  & Kodak 22: 0.097459\\ &  &  &  &  & Kodak 23: 0.103756\\ &  &  &  &  & Kodak 24: 0.110673\\\hline\hline64 & MSE & 0.025 & 5x5deconv,2,113 & 5x5deconv,2,320 & Kodak 1: 0.471199\\ &  &  & 5x5deconv,2,246 & 5x5deconv,2,303 & Kodak 2: 0.450293\\ &  &  & 5x5deconv,2,320 & 5x5deconv,2,306 & Kodak 3: 0.454965\\ &  &  &  & 5x5deconv,2,3 & Kodak 4: 0.441081\\ &  &  &  &  & Kodak 5: 0.448661\\ &  &  &  &  & Kodak 6: 0.448481\\ &  &  &  &  & Kodak 7: 0.448504\\ &  &  &  &  & Kodak 8: 0.443522\\ &  &  &  &  & Kodak 9: 0.448359\\ &  &  &  &  & Kodak 10: 0.450028\\ &  &  &  &  & Kodak 11: 0.448614\\ &  &  &  &  & Kodak 12: 0.444359\\ &  &  &  &  & Kodak 13: 0.457297\\ &  &  &  &  & Kodak 14: 0.444442\\ &  &  &  &  & Kodak 15: 0.456633\\ &  &  &  &  & Kodak 16: 0.450701\\ &  &  &  &  & Kodak 17: 0.444565\\ &  &  &  &  & Kodak 18: 0.444644\\ &  &  &  &  & Kodak 19: 0.441936\\ &  &  &  &  & Kodak 20: 0.445846\\ &  &  &  &  & Kodak 21: 0.454508\\ &  &  &  &  & Kodak 22: 0.454615\\ &  &  &  &  & Kodak 23: 0.526799\\ &  &  &  &  & Kodak 24: 0.459257\\\hline\hline65 & MSE & 0.025 & 5x5deconv,2,115 & 5x5deconv,2,320 & Kodak 1: 0.493474\\ &  &  & 5x5deconv,2,346 & 5x5deconv,2,319 & Kodak 2: 0.471851\\ &  &  & 5x5deconv,2,320 & 5x5deconv,2,320 & Kodak 3: 0.474651\\ &  &  &  & 5x5deconv,2,3 & Kodak 4: 0.469305\\ &  &  &  &  & Kodak 5: 0.476248\\ &  &  &  &  & Kodak 6: 0.472390\\ &  &  &  &  & Kodak 7: 0.469519\\ &  &  &  &  & Kodak 8: 0.467567\\ &  &  &  &  & Kodak 9: 0.463412\\ &  &  &  &  & Kodak 10: 0.467363\\ &  &  &  &  & Kodak 11: 0.468762\\ &  &  &  &  & Kodak 12: 0.468293\\ &  &  &  &  & Kodak 13: 0.468512\\ &  &  &  &  & Kodak 14: 0.472320\\ &  &  &  &  & Kodak 15: 0.466259\\ &  &  &  &  & Kodak 16: 0.472126\\ &  &  &  &  & Kodak 17: 0.512347\\ &  &  &  &  & Kodak 18: 0.470400\\ &  &  &  &  & Kodak 19: 0.485009\\ &  &  &  &  & Kodak 20: 0.519214\\ &  &  &  &  & Kodak 21: 0.490701\\ &  &  &  &  & Kodak 22: 0.469064\\ &  &  &  &  & Kodak 23: 0.469196\\ &  &  &  &  & Kodak 24: 0.470258\\\hline\hline66 & MSE & 0.025 & 5x5deconv,2,28 & 5x5deconv,2,47 & Kodak 1: 0.126172\\ &  &  & 5x5deconv,2,34 & 5x5deconv,2,19 & Kodak 2: 0.128810\\ &  &  & 5x5deconv,2,320 & 5x5deconv,2,28 & Kodak 3: 0.128979\\ &  &  &  & 5x5deconv,2,3 & Kodak 4: 0.129763\\ &  &  &  &  & Kodak 5: 0.126467\\ &  &  &  &  & Kodak 6: 0.123119\\ &  &  &  &  & Kodak 7: 0.131150\\ &  &  &  &  & Kodak 8: 0.124310\\ &  &  &  &  & Kodak 9: 0.121844\\ &  &  &  &  & Kodak 10: 0.126956\\ &  &  &  &  & Kodak 11: 0.122481\\ &  &  &  &  & Kodak 12: 0.119298\\ &  &  &  &  & Kodak 13: 0.130828\\ &  &  &  &  & Kodak 14: 0.129165\\ &  &  &  &  & Kodak 15: 0.115133\\ &  &  &  &  & Kodak 16: 0.117899\\ &  &  &  &  & Kodak 17: 0.127058\\ &  &  &  &  & Kodak 18: 0.117687\\ &  &  &  &  & Kodak 19: 0.130410\\ &  &  &  &  & Kodak 20: 0.114593\\ &  &  &  &  & Kodak 21: 0.122041\\ &  &  &  &  & Kodak 22: 0.120112\\ &  &  &  &  & Kodak 23: 0.125807\\ &  &  &  &  & Kodak 24: 0.132052\\\hline\hline67 & MSE & 0.025 & 5x5deconv,2,85 & 5x5deconv,2,110 & Kodak 1: 0.144512\\ &  &  & 5x5deconv,2,66 & 5x5deconv,2,39 & Kodak 2: 0.132550\\ &  &  & 5x5deconv,2,320 & 5x5deconv,2,44 & Kodak 3: 0.131305\\ &  &  &  & 5x5deconv,2,3 & Kodak 4: 0.134787\\ &  &  &  &  & Kodak 5: 0.142403\\ &  &  &  &  & Kodak 6: 0.136041\\ &  &  &  &  & Kodak 7: 0.137662\\ &  &  &  &  & Kodak 8: 0.140479\\ &  &  &  &  & Kodak 9: 0.143081\\ &  &  &  &  & Kodak 10: 0.132586\\ &  &  &  &  & Kodak 11: 0.147049\\ &  &  &  &  & Kodak 12: 0.149739\\ &  &  &  &  & Kodak 13: 0.147196\\ &  &  &  &  & Kodak 14: 0.141666\\ &  &  &  &  & Kodak 15: 0.138064\\ &  &  &  &  & Kodak 16: 0.135568\\ &  &  &  &  & Kodak 17: 0.139408\\ &  &  &  &  & Kodak 18: 0.136008\\ &  &  &  &  & Kodak 19: 0.138843\\ &  &  &  &  & Kodak 20: 0.138041\\ &  &  &  &  & Kodak 21: 0.136502\\ &  &  &  &  & Kodak 22: 0.134934\\ &  &  &  &  & Kodak 23: 0.139923\\ &  &  &  &  & Kodak 24: 0.153896\\\hline\hline68 & MSE & 0.025 & 5x5deconv,2,4 & 5x5deconv,2,26 & Kodak 1: 0.109398\\ &  &  & 5x5deconv,2,12 & 5x5deconv,2,15 & Kodak 2: 0.119560\\ &  &  & 5x5deconv,2,320 & 5x5deconv,2,11 & Kodak 3: 0.110655\\ &  &  &  & 5x5deconv,2,3 & Kodak 4: 0.106571\\ &  &  &  &  & Kodak 5: 0.122674\\ &  &  &  &  & Kodak 6: 0.108505\\ &  &  &  &  & Kodak 7: 0.111185\\ &  &  &  &  & Kodak 8: 0.113768\\ &  &  &  &  & Kodak 9: 0.109739\\ &  &  &  &  & Kodak 10: 0.111724\\ &  &  &  &  & Kodak 11: 0.115317\\ &  &  &  &  & Kodak 12: 0.119405\\ &  &  &  &  & Kodak 13: 0.115536\\ &  &  &  &  & Kodak 14: 0.112115\\ &  &  &  &  & Kodak 15: 0.112720\\ &  &  &  &  & Kodak 16: 0.116174\\ &  &  &  &  & Kodak 17: 0.121289\\ &  &  &  &  & Kodak 18: 0.114642\\ &  &  &  &  & Kodak 19: 0.110232\\ &  &  &  &  & Kodak 20: 0.106154\\ &  &  &  &  & Kodak 21: 0.126171\\ &  &  &  &  & Kodak 22: 0.114413\\ &  &  &  &  & Kodak 23: 0.116589\\ &  &  &  &  & Kodak 24: 0.111845\\\hline\hline69 & MSE & 0.025 & 5x5deconv,2,10 & 5x5deconv,2,1 & Kodak 1: 0.090204\\ &  &  & 5x5deconv,2,10 & 5x5deconv,2,1 & Kodak 2: 0.100833\\ &  &  & 5x5deconv,2,320 & 5x5deconv,2,1 & Kodak 3: 0.096304\\ &  &  &  & 5x5deconv,2,3 & Kodak 4: 0.100764\\ &  &  &  &  & Kodak 5: 0.100862\\ &  &  &  &  & Kodak 6: 0.092029\\ &  &  &  &  & Kodak 7: 0.098764\\ &  &  &  &  & Kodak 8: 0.096118\\ &  &  &  &  & Kodak 9: 0.093777\\ &  &  &  &  & Kodak 10: 0.100469\\ &  &  &  &  & Kodak 11: 0.094719\\ &  &  &  &  & Kodak 12: 0.100989\\ &  &  &  &  & Kodak 13: 0.105269\\ &  &  &  &  & Kodak 14: 0.105896\\ &  &  &  &  & Kodak 15: 0.103095\\ &  &  &  &  & Kodak 16: 0.099579\\ &  &  &  &  & Kodak 17: 0.103033\\ &  &  &  &  & Kodak 18: 0.102586\\ &  &  &  &  & Kodak 19: 0.099869\\ &  &  &  &  & Kodak 20: 0.096570\\ &  &  &  &  & Kodak 21: 0.106639\\ &  &  &  &  & Kodak 22: 0.106849\\ &  &  &  &  & Kodak 23: 0.099467\\ &  &  &  &  & Kodak 24: 0.096739\\\hline\hline70 & MSE & 0.025 & 5x5deconv,2,142 & 5x5deconv,2,192 & Kodak 1: 0.218042\\ &  &  & 5x5deconv,2,114 & 5x5deconv,2,76 & Kodak 2: 0.186117\\ &  &  & 5x5deconv,2,320 & 5x5deconv,2,124 & Kodak 3: 0.196087\\ &  &  &  & 5x5deconv,2,3 & Kodak 4: 0.195595\\ &  &  &  &  & Kodak 5: 0.198103\\ &  &  &  &  & Kodak 6: 0.198196\\ &  &  &  &  & Kodak 7: 0.192191\\ &  &  &  &  & Kodak 8: 0.195907\\ &  &  &  &  & Kodak 9: 0.226529\\ &  &  &  &  & Kodak 10: 0.191502\\ &  &  &  &  & Kodak 11: 0.200649\\ &  &  &  &  & Kodak 12: 0.231672\\ &  &  &  &  & Kodak 13: 0.198731\\ &  &  &  &  & Kodak 14: 0.205031\\ &  &  &  &  & Kodak 15: 0.224497\\ &  &  &  &  & Kodak 16: 0.218638\\ &  &  &  &  & Kodak 17: 0.187244\\ &  &  &  &  & Kodak 18: 0.194402\\ &  &  &  &  & Kodak 19: 0.197020\\ &  &  &  &  & Kodak 20: 0.200738\\ &  &  &  &  & Kodak 21: 0.194183\\ &  &  &  &  & Kodak 22: 0.193257\\ &  &  &  &  & Kodak 23: 0.190129\\ &  &  &  &  & Kodak 24: 0.189787\\\hline\hline71 & MSE & 0.025 & 5x5deconv,2,10 & 5x5deconv,2,1 & Kodak 1: 0.099983\\ &  &  & 5x5deconv,2,10 & 5x5deconv,2,6 & Kodak 2: 0.102138\\ &  &  & 5x5deconv,2,320 & 5x5deconv,2,1 & Kodak 3: 0.106100\\ &  &  &  & 5x5deconv,2,3 & Kodak 4: 0.100605\\ &  &  &  &  & Kodak 5: 0.103042\\ &  &  &  &  & Kodak 6: 0.102361\\ &  &  &  &  & Kodak 7: 0.101216\\ &  &  &  &  & Kodak 8: 0.111181\\ &  &  &  &  & Kodak 9: 0.099277\\ &  &  &  &  & Kodak 10: 0.103119\\ &  &  &  &  & Kodak 11: 0.106275\\ &  &  &  &  & Kodak 12: 0.098726\\ &  &  &  &  & Kodak 13: 0.102677\\ &  &  &  &  & Kodak 14: 0.111621\\ &  &  &  &  & Kodak 15: 0.097879\\ &  &  &  &  & Kodak 16: 0.097780\\ &  &  &  &  & Kodak 17: 0.100116\\ &  &  &  &  & Kodak 18: 0.100887\\ &  &  &  &  & Kodak 19: 0.097322\\ &  &  &  &  & Kodak 20: 0.096679\\ &  &  &  &  & Kodak 21: 0.102031\\ &  &  &  &  & Kodak 22: 0.109935\\ &  &  &  &  & Kodak 23: 0.099062\\ &  &  &  &  & Kodak 24: 0.099268\\\hline\hline72 & MSE & 0.025 & 5x5deconv,2,10 & 5x5deconv,2,1 & Kodak 1: 0.104330\\ &  &  & 5x5deconv,2,10 & 5x5deconv,2,11 & Kodak 2: 0.104052\\ &  &  & 5x5deconv,2,320 & 5x5deconv,2,1 & Kodak 3: 0.102146\\ &  &  &  & 5x5deconv,2,3 & Kodak 4: 0.099704\\ &  &  &  &  & Kodak 5: 0.100174\\ &  &  &  &  & Kodak 6: 0.104140\\ &  &  &  &  & Kodak 7: 0.105996\\ &  &  &  &  & Kodak 8: 0.116984\\ &  &  &  &  & Kodak 9: 0.097165\\ &  &  &  &  & Kodak 10: 0.098570\\ &  &  &  &  & Kodak 11: 0.100415\\ &  &  &  &  & Kodak 12: 0.107896\\ &  &  &  &  & Kodak 13: 0.099055\\ &  &  &  &  & Kodak 14: 0.100591\\ &  &  &  &  & Kodak 15: 0.100418\\ &  &  &  &  & Kodak 16: 0.098755\\ &  &  &  &  & Kodak 17: 0.113081\\ &  &  &  &  & Kodak 18: 0.100525\\ &  &  &  &  & Kodak 19: 0.097398\\ &  &  &  &  & Kodak 20: 0.117000\\ &  &  &  &  & Kodak 21: 0.107555\\ &  &  &  &  & Kodak 22: 0.109995\\ &  &  &  &  & Kodak 23: 0.100056\\ &  &  &  &  & Kodak 24: 0.104806\\\hline\hline73 & MSE & 0.025 & 5x5deconv,2,319 & 5x5deconv,2,320 & Kodak 1: 0.476723\\ &  &  & 5x5deconv,2,180 & 5x5deconv,2,275 & Kodak 2: 0.442182\\ &  &  & 5x5deconv,2,320 & 5x5deconv,2,319 & Kodak 3: 0.475166\\ &  &  &  & 5x5deconv,2,3 & Kodak 4: 0.444103\\ &  &  &  &  & Kodak 5: 0.450079\\ &  &  &  &  & Kodak 6: 0.452229\\ &  &  &  &  & Kodak 7: 0.445693\\ &  &  &  &  & Kodak 8: 0.445370\\ &  &  &  &  & Kodak 9: 0.442961\\ &  &  &  &  & Kodak 10: 0.438327\\ &  &  &  &  & Kodak 11: 0.437572\\ &  &  &  &  & Kodak 12: 0.446282\\ &  &  &  &  & Kodak 13: 0.446698\\ &  &  &  &  & Kodak 14: 0.442369\\ &  &  &  &  & Kodak 15: 0.457727\\ &  &  &  &  & Kodak 16: 0.447951\\ &  &  &  &  & Kodak 17: 0.440340\\ &  &  &  &  & Kodak 18: 0.453139\\ &  &  &  &  & Kodak 19: 0.449370\\ &  &  &  &  & Kodak 20: 0.446584\\ &  &  &  &  & Kodak 21: 0.446308\\ &  &  &  &  & Kodak 22: 0.454053\\ &  &  &  &  & Kodak 23: 0.444977\\ &  &  &  &  & Kodak 24: 0.449817\\\hline\hline74 & MSE & 0.025 & 5x5deconv,2,199 & 5x5deconv,2,320 & Kodak 1: 0.533857\\ &  &  & 5x5deconv,2,443 & 5x5deconv,2,320 & Kodak 2: 0.491456\\ &  &  & 5x5deconv,2,320 & 5x5deconv,2,320 & Kodak 3: 0.496640\\ &  &  &  & 5x5deconv,2,3 & Kodak 4: 0.566564\\ &  &  &  &  & Kodak 5: 0.504187\\ &  &  &  &  & Kodak 6: 0.480103\\ &  &  &  &  & Kodak 7: 0.502153\\ &  &  &  &  & Kodak 8: 0.504958\\ &  &  &  &  & Kodak 9: 0.513165\\ &  &  &  &  & Kodak 10: 0.488426\\ &  &  &  &  & Kodak 11: 0.497813\\ &  &  &  &  & Kodak 12: 0.489014\\ &  &  &  &  & Kodak 13: 0.491340\\ &  &  &  &  & Kodak 14: 0.492112\\ &  &  &  &  & Kodak 15: 0.498142\\ &  &  &  &  & Kodak 16: 0.509052\\ &  &  &  &  & Kodak 17: 0.489430\\ &  &  &  &  & Kodak 18: 0.569338\\ &  &  &  &  & Kodak 19: 0.487665\\ &  &  &  &  & Kodak 20: 0.492255\\ &  &  &  &  & Kodak 21: 0.523849\\ &  &  &  &  & Kodak 22: 0.512162\\ &  &  &  &  & Kodak 23: 0.496619\\ &  &  &  &  & Kodak 24: 0.507937\\\hline\hline75 & MSE & 0.025 & 5x5deconv,2,210 & 5x5deconv,2,320 & Kodak 1: 0.481300\\ &  &  & 5x5deconv,2,256 & 5x5deconv,2,320 & Kodak 2: 0.464904\\ &  &  & 5x5deconv,2,320 & 5x5deconv,2,320 & Kodak 3: 0.467622\\ &  &  &  & 5x5deconv,2,3 & Kodak 4: 0.465374\\ &  &  &  &  & Kodak 5: 0.468599\\ &  &  &  &  & Kodak 6: 0.463313\\ &  &  &  &  & Kodak 7: 0.455455\\ &  &  &  &  & Kodak 8: 0.466972\\ &  &  &  &  & Kodak 9: 0.468299\\ &  &  &  &  & Kodak 10: 0.465804\\ &  &  &  &  & Kodak 11: 0.459112\\ &  &  &  &  & Kodak 12: 0.472172\\ &  &  &  &  & Kodak 13: 0.464121\\ &  &  &  &  & Kodak 14: 0.471428\\ &  &  &  &  & Kodak 15: 0.468556\\ &  &  &  &  & Kodak 16: 0.480610\\ &  &  &  &  & Kodak 17: 0.458480\\ &  &  &  &  & Kodak 18: 0.467159\\ &  &  &  &  & Kodak 19: 0.459812\\ &  &  &  &  & Kodak 20: 0.468978\\ &  &  &  &  & Kodak 21: 0.460424\\ &  &  &  &  & Kodak 22: 0.461937\\ &  &  &  &  & Kodak 23: 0.476625\\ &  &  &  &  & Kodak 24: 0.467505\\\hline\hline76 & MSE & 0.025 & 5x5deconv,2,4 & 5x5deconv,2,16 & Kodak 1: 0.099590\\ &  &  & 5x5deconv,2,4 & 5x5deconv,2,9 & Kodak 2: 0.100831\\ &  &  & 5x5deconv,2,320 & 5x5deconv,2,3 & Kodak 3: 0.101689\\ &  &  &  & 5x5deconv,2,3 & Kodak 4: 0.101508\\ &  &  &  &  & Kodak 5: 0.106966\\ &  &  &  &  & Kodak 6: 0.098450\\ &  &  &  &  & Kodak 7: 0.097751\\ &  &  &  &  & Kodak 8: 0.103280\\ &  &  &  &  & Kodak 9: 0.103220\\ &  &  &  &  & Kodak 10: 0.100577\\ &  &  &  &  & Kodak 11: 0.102981\\ &  &  &  &  & Kodak 12: 0.099982\\ &  &  &  &  & Kodak 13: 0.106983\\ &  &  &  &  & Kodak 14: 0.102349\\ &  &  &  &  & Kodak 15: 0.095603\\ &  &  &  &  & Kodak 16: 0.099341\\ &  &  &  &  & Kodak 17: 0.099715\\ &  &  &  &  & Kodak 18: 0.099833\\ &  &  &  &  & Kodak 19: 0.097220\\ &  &  &  &  & Kodak 20: 0.099747\\ &  &  &  &  & Kodak 21: 0.098981\\ &  &  &  &  & Kodak 22: 0.096338\\ &  &  &  &  & Kodak 23: 0.108860\\ &  &  &  &  & Kodak 24: 0.100603\\\hline\hline77 & MS-SSIM & 1.0 & 5x5deconv,2,229 & 5x5deconv,2,106 & Kodak 1: 0.149801\\ &  &  & 5x5deconv,2,203 & 5x5deconv,2,125 & Kodak 2: 0.155137\\ &  &  & 5x5deconv,2,320 & 5x5deconv,2,56 & Kodak 3: 0.151611\\ &  &  &  & 5x5deconv,2,3 & Kodak 4: 0.163796\\ &  &  &  &  & Kodak 5: 0.158872\\ &  &  &  &  & Kodak 6: 0.154118\\ &  &  &  &  & Kodak 7: 0.158567\\ &  &  &  &  & Kodak 8: 0.157644\\ &  &  &  &  & Kodak 9: 0.161582\\ &  &  &  &  & Kodak 10: 0.158951\\ &  &  &  &  & Kodak 11: 0.156279\\ &  &  &  &  & Kodak 12: 0.163706\\ &  &  &  &  & Kodak 13: 0.159181\\ &  &  &  &  & Kodak 14: 0.156990\\ &  &  &  &  & Kodak 15: 0.160291\\ &  &  &  &  & Kodak 16: 0.161380\\ &  &  &  &  & Kodak 17: 0.156793\\ &  &  &  &  & Kodak 18: 0.160366\\ &  &  &  &  & Kodak 19: 0.152899\\ &  &  &  &  & Kodak 20: 0.154157\\ &  &  &  &  & Kodak 21: 0.155683\\ &  &  &  &  & Kodak 22: 0.165125\\ &  &  &  &  & Kodak 23: 0.156974\\ &  &  &  &  & Kodak 24: 0.156774\\\hline\hline78 & MS-SSIM & 1.0 & 5x5deconv,2,98 & 5x5deconv,2,46 & Kodak 1: 0.118821\\ &  &  & 5x5deconv,2,96 & 5x5deconv,2,114 & Kodak 2: 0.136606\\ &  &  & 5x5deconv,2,320 & 5x5deconv,2,14 & Kodak 3: 0.128351\\ &  &  &  & 5x5deconv,2,3 & Kodak 4: 0.132400\\ &  &  &  &  & Kodak 5: 0.135914\\ &  &  &  &  & Kodak 6: 0.129586\\ &  &  &  &  & Kodak 7: 0.134116\\ &  &  &  &  & Kodak 8: 0.130086\\ &  &  &  &  & Kodak 9: 0.126781\\ &  &  &  &  & Kodak 10: 0.133542\\ &  &  &  &  & Kodak 11: 0.134419\\ &  &  &  &  & Kodak 12: 0.133616\\ &  &  &  &  & Kodak 13: 0.138083\\ &  &  &  &  & Kodak 14: 0.129353\\ &  &  &  &  & Kodak 15: 0.125313\\ &  &  &  &  & Kodak 16: 0.128617\\ &  &  &  &  & Kodak 17: 0.134969\\ &  &  &  &  & Kodak 18: 0.132591\\ &  &  &  &  & Kodak 19: 0.132436\\ &  &  &  &  & Kodak 20: 0.131942\\ &  &  &  &  & Kodak 21: 0.130701\\ &  &  &  &  & Kodak 22: 0.133823\\ &  &  &  &  & Kodak 23: 0.127813\\ &  &  &  &  & Kodak 24: 0.130003\\\hline\hline79 & MS-SSIM & 1.0 & 5x5deconv,2,10 & 5x5deconv,2,1 & Kodak 1: 0.090525\\ &  &  & 5x5deconv,2,10 & 5x5deconv,2,1 & Kodak 2: 0.096524\\ &  &  & 5x5deconv,2,320 & 5x5deconv,2,1 & Kodak 3: 0.095512\\ &  &  &  & 5x5deconv,2,3 & Kodak 4: 0.096298\\ &  &  &  &  & Kodak 5: 0.095812\\ &  &  &  &  & Kodak 6: 0.094332\\ &  &  &  &  & Kodak 7: 0.096759\\ &  &  &  &  & Kodak 8: 0.095831\\ &  &  &  &  & Kodak 9: 0.097705\\ &  &  &  &  & Kodak 10: 0.092775\\ &  &  &  &  & Kodak 11: 0.094016\\ &  &  &  &  & Kodak 12: 0.096345\\ &  &  &  &  & Kodak 13: 0.092695\\ &  &  &  &  & Kodak 14: 0.105628\\ &  &  &  &  & Kodak 15: 0.094925\\ &  &  &  &  & Kodak 16: 0.092806\\ &  &  &  &  & Kodak 17: 0.099364\\ &  &  &  &  & Kodak 18: 0.095906\\ &  &  &  &  & Kodak 19: 0.095588\\ &  &  &  &  & Kodak 20: 0.097143\\ &  &  &  &  & Kodak 21: 0.095678\\ &  &  &  &  & Kodak 22: 0.096565\\ &  &  &  &  & Kodak 23: 0.097550\\ &  &  &  &  & Kodak 24: 0.093400\\\hline\hline80 & MS-SSIM & 1.0 & 5x5deconv,2,10 & 5x5deconv,2,1 & Kodak 1: 0.088427\\ &  &  & 5x5deconv,2,10 & 5x5deconv,2,1 & Kodak 2: 0.094563\\ &  &  & 5x5deconv,2,320 & 5x5deconv,2,1 & Kodak 3: 0.092668\\ &  &  &  & 5x5deconv,2,3 & Kodak 4: 0.096206\\ &  &  &  &  & Kodak 5: 0.094335\\ &  &  &  &  & Kodak 6: 0.094336\\ &  &  &  &  & Kodak 7: 0.094926\\ &  &  &  &  & Kodak 8: 0.095874\\ &  &  &  &  & Kodak 9: 0.092345\\ &  &  &  &  & Kodak 10: 0.095088\\ &  &  &  &  & Kodak 11: 0.095698\\ &  &  &  &  & Kodak 12: 0.093030\\ &  &  &  &  & Kodak 13: 0.098263\\ &  &  &  &  & Kodak 14: 0.093185\\ &  &  &  &  & Kodak 15: 0.095272\\ &  &  &  &  & Kodak 16: 0.092979\\ &  &  &  &  & Kodak 17: 0.096259\\ &  &  &  &  & Kodak 18: 0.098528\\ &  &  &  &  & Kodak 19: 0.096517\\ &  &  &  &  & Kodak 20: 0.093129\\ &  &  &  &  & Kodak 21: 0.099143\\ &  &  &  &  & Kodak 22: 0.093881\\ &  &  &  &  & Kodak 23: 0.091402\\ &  &  &  &  & Kodak 24: 0.095125\\\hline\hline81 & MS-SSIM & 1.0 & 5x5deconv,2,10 & 5x5deconv,2,1 & Kodak 1: 0.089144\\ &  &  & 5x5deconv,2,10 & 5x5deconv,2,1 & Kodak 2: 0.093461\\ &  &  & 5x5deconv,2,320 & 5x5deconv,2,1 & Kodak 3: 0.098405\\ &  &  &  & 5x5deconv,2,3 & Kodak 4: 0.098283\\ &  &  &  &  & Kodak 5: 0.094969\\ &  &  &  &  & Kodak 6: 0.096370\\ &  &  &  &  & Kodak 7: 0.090559\\ &  &  &  &  & Kodak 8: 0.095831\\ &  &  &  &  & Kodak 9: 0.092194\\ &  &  &  &  & Kodak 10: 0.093678\\ &  &  &  &  & Kodak 11: 0.095456\\ &  &  &  &  & Kodak 12: 0.094078\\ &  &  &  &  & Kodak 13: 0.092918\\ &  &  &  &  & Kodak 14: 0.097994\\ &  &  &  &  & Kodak 15: 0.095197\\ &  &  &  &  & Kodak 16: 0.097426\\ &  &  &  &  & Kodak 17: 0.093913\\ &  &  &  &  & Kodak 18: 0.094592\\ &  &  &  &  & Kodak 19: 0.098320\\ &  &  &  &  & Kodak 20: 0.090853\\ &  &  &  &  & Kodak 21: 0.095273\\ &  &  &  &  & Kodak 22: 0.092657\\ &  &  &  &  & Kodak 23: 0.095467\\ &  &  &  &  & Kodak 24: 0.094699\\\hline\hline82 & MS-SSIM & 1.0 & 5x5deconv,2,37 & 5x5deconv,2,38 & Kodak 1: 0.105813\\ &  &  & 5x5deconv,2,24 & 5x5deconv,2,22 & Kodak 2: 0.109280\\ &  &  & 5x5deconv,2,320 & 5x5deconv,2,9 & Kodak 3: 0.113925\\ &  &  &  & 5x5deconv,2,3 & Kodak 4: 0.103787\\ &  &  &  &  & Kodak 5: 0.109940\\ &  &  &  &  & Kodak 6: 0.110505\\ &  &  &  &  & Kodak 7: 0.102785\\ &  &  &  &  & Kodak 8: 0.104807\\ &  &  &  &  & Kodak 9: 0.103851\\ &  &  &  &  & Kodak 10: 0.106815\\ &  &  &  &  & Kodak 11: 0.104966\\ &  &  &  &  & Kodak 12: 0.111416\\ &  &  &  &  & Kodak 13: 0.108740\\ &  &  &  &  & Kodak 14: 0.110929\\ &  &  &  &  & Kodak 15: 0.107710\\ &  &  &  &  & Kodak 16: 0.103544\\ &  &  &  &  & Kodak 17: 0.108648\\ &  &  &  &  & Kodak 18: 0.112423\\ &  &  &  &  & Kodak 19: 0.107322\\ &  &  &  &  & Kodak 20: 0.110685\\ &  &  &  &  & Kodak 21: 0.107211\\ &  &  &  &  & Kodak 22: 0.106434\\ &  &  &  &  & Kodak 23: 0.106228\\ &  &  &  &  & Kodak 24: 0.105368\\\hline\hline83 & MS-SSIM & 1.0 & 5x5deconv,2,98 & 5x5deconv,2,46 & Kodak 1: 0.134267\\ &  &  & 5x5deconv,2,96 & 5x5deconv,2,114 & Kodak 2: 0.132070\\ &  &  & 5x5deconv,2,320 & 5x5deconv,2,14 & Kodak 3: 0.139644\\ &  &  &  & 5x5deconv,2,3 & Kodak 4: 0.128537\\ &  &  &  &  & Kodak 5: 0.138736\\ &  &  &  &  & Kodak 6: 0.128855\\ &  &  &  &  & Kodak 7: 0.135693\\ &  &  &  &  & Kodak 8: 0.134837\\ &  &  &  &  & Kodak 9: 0.129103\\ &  &  &  &  & Kodak 10: 0.124742\\ &  &  &  &  & Kodak 11: 0.129064\\ &  &  &  &  & Kodak 12: 0.133395\\ &  &  &  &  & Kodak 13: 0.137553\\ &  &  &  &  & Kodak 14: 0.135685\\ &  &  &  &  & Kodak 15: 0.132546\\ &  &  &  &  & Kodak 16: 0.128388\\ &  &  &  &  & Kodak 17: 0.130209\\ &  &  &  &  & Kodak 18: 0.129813\\ &  &  &  &  & Kodak 19: 0.134251\\ &  &  &  &  & Kodak 20: 0.134002\\ &  &  &  &  & Kodak 21: 0.131188\\ &  &  &  &  & Kodak 22: 0.132911\\ &  &  &  &  & Kodak 23: 0.127468\\ &  &  &  &  & Kodak 24: 0.131464\\\hline\hline84 & MS-SSIM & 1.0 & 5x5deconv,2,10 & 5x5deconv,2,1 & Kodak 1: 0.089730\\ &  &  & 5x5deconv,2,10 & 5x5deconv,2,1 & Kodak 2: 0.096997\\ &  &  & 5x5deconv,2,320 & 5x5deconv,2,1 & Kodak 3: 0.095891\\ &  &  &  & 5x5deconv,2,3 & Kodak 4: 0.099189\\ &  &  &  &  & Kodak 5: 0.094569\\ &  &  &  &  & Kodak 6: 0.091596\\ &  &  &  &  & Kodak 7: 0.095272\\ &  &  &  &  & Kodak 8: 0.093048\\ &  &  &  &  & Kodak 9: 0.095125\\ &  &  &  &  & Kodak 10: 0.102768\\ &  &  &  &  & Kodak 11: 0.098459\\ &  &  &  &  & Kodak 12: 0.093141\\ &  &  &  &  & Kodak 13: 0.092052\\ &  &  &  &  & Kodak 14: 0.101488\\ &  &  &  &  & Kodak 15: 0.093133\\ &  &  &  &  & Kodak 16: 0.093396\\ &  &  &  &  & Kodak 17: 0.090089\\ &  &  &  &  & Kodak 18: 0.097803\\ &  &  &  &  & Kodak 19: 0.095879\\ &  &  &  &  & Kodak 20: 0.093986\\ &  &  &  &  & Kodak 21: 0.094245\\ &  &  &  &  & Kodak 22: 0.094780\\ &  &  &  &  & Kodak 23: 0.091968\\ &  &  &  &  & Kodak 24: 0.094561\\\hline\hline85 & MS-SSIM & 1.0 & 5x5deconv,2,10 & 5x5deconv,2,4 & Kodak 1: 0.096777\\ &  &  & 5x5deconv,2,10 & 5x5deconv,2,9 & Kodak 2: 0.096469\\ &  &  & 5x5deconv,2,320 & 5x5deconv,2,1 & Kodak 3: 0.095039\\ &  &  &  & 5x5deconv,2,3 & Kodak 4: 0.097063\\ &  &  &  &  & Kodak 5: 0.099434\\ &  &  &  &  & Kodak 6: 0.100631\\ &  &  &  &  & Kodak 7: 0.094776\\ &  &  &  &  & Kodak 8: 0.095272\\ &  &  &  &  & Kodak 9: 0.096256\\ &  &  &  &  & Kodak 10: 0.098695\\ &  &  &  &  & Kodak 11: 0.106370\\ &  &  &  &  & Kodak 12: 0.104930\\ &  &  &  &  & Kodak 13: 0.109110\\ &  &  &  &  & Kodak 14: 0.098773\\ &  &  &  &  & Kodak 15: 0.097639\\ &  &  &  &  & Kodak 16: 0.099007\\ &  &  &  &  & Kodak 17: 0.103006\\ &  &  &  &  & Kodak 18: 0.101320\\ &  &  &  &  & Kodak 19: 0.096077\\ &  &  &  &  & Kodak 20: 0.105637\\ &  &  &  &  & Kodak 21: 0.100139\\ &  &  &  &  & Kodak 22: 0.100934\\ &  &  &  &  & Kodak 23: 0.098253\\ &  &  &  &  & Kodak 24: 0.095669\\\hline\hline86 & MS-SSIM & 1.0 & 5x5deconv,2,4 & 5x5deconv,2,8 & Kodak 1: 0.102242\\ &  &  & 5x5deconv,2,18 & 5x5deconv,2,23 & Kodak 2: 0.104089\\ &  &  & 5x5deconv,2,320 & 5x5deconv,2,2 & Kodak 3: 0.099716\\ &  &  &  & 5x5deconv,2,3 & Kodak 4: 0.098831\\ &  &  &  &  & Kodak 5: 0.099385\\ &  &  &  &  & Kodak 6: 0.101402\\ &  &  &  &  & Kodak 7: 0.102516\\ &  &  &  &  & Kodak 8: 0.099966\\ &  &  &  &  & Kodak 9: 0.102274\\ &  &  &  &  & Kodak 10: 0.096479\\ &  &  &  &  & Kodak 11: 0.097433\\ &  &  &  &  & Kodak 12: 0.100284\\ &  &  &  &  & Kodak 13: 0.102165\\ &  &  &  &  & Kodak 14: 0.102181\\ &  &  &  &  & Kodak 15: 0.106087\\ &  &  &  &  & Kodak 16: 0.101082\\ &  &  &  &  & Kodak 17: 0.102660\\ &  &  &  &  & Kodak 18: 0.096182\\ &  &  &  &  & Kodak 19: 0.102919\\ &  &  &  &  & Kodak 20: 0.101093\\ &  &  &  &  & Kodak 21: 0.098507\\ &  &  &  &  & Kodak 22: 0.098837\\ &  &  &  &  & Kodak 23: 0.101636\\ &  &  &  &  & Kodak 24: 0.103183\\\hline\hline87 & MS-SSIM & 1.0 & 5x5deconv,2,392 & 5x5deconv,2,158 & Kodak 1: 0.219780\\ &  &  & 5x5deconv,2,215 & 5x5deconv,2,216 & Kodak 2: 0.223463\\ &  &  & 5x5deconv,2,320 & 5x5deconv,2,112 & Kodak 3: 0.216473\\ &  &  &  & 5x5deconv,2,3 & Kodak 4: 0.225869\\ &  &  &  &  & Kodak 5: 0.222247\\ &  &  &  &  & Kodak 6: 0.218940\\ &  &  &  &  & Kodak 7: 0.222522\\ &  &  &  &  & Kodak 8: 0.220914\\ &  &  &  &  & Kodak 9: 0.221806\\ &  &  &  &  & Kodak 10: 0.225328\\ &  &  &  &  & Kodak 11: 0.219423\\ &  &  &  &  & Kodak 12: 0.217090\\ &  &  &  &  & Kodak 13: 0.220486\\ &  &  &  &  & Kodak 14: 0.220883\\ &  &  &  &  & Kodak 15: 0.222794\\ &  &  &  &  & Kodak 16: 0.219317\\ &  &  &  &  & Kodak 17: 0.220656\\ &  &  &  &  & Kodak 18: 0.220295\\ &  &  &  &  & Kodak 19: 0.221644\\ &  &  &  &  & Kodak 20: 0.217086\\ &  &  &  &  & Kodak 21: 0.223427\\ &  &  &  &  & Kodak 22: 0.227723\\ &  &  &  &  & Kodak 23: 0.220944\\ &  &  &  &  & Kodak 24: 0.217942\\\hline\hline88 & MS-SSIM & 1.0 & 5x5deconv,2,10 & 5x5deconv,2,1 & Kodak 1: 0.091156\\ &  &  & 5x5deconv,2,10 & 5x5deconv,2,1 & Kodak 2: 0.098751\\ &  &  & 5x5deconv,2,320 & 5x5deconv,2,1 & Kodak 3: 0.096639\\ &  &  &  & 5x5deconv,2,3 & Kodak 4: 0.093505\\ &  &  &  &  & Kodak 5: 0.093775\\ &  &  &  &  & Kodak 6: 0.091790\\ &  &  &  &  & Kodak 7: 0.096371\\ &  &  &  &  & Kodak 8: 0.092542\\ &  &  &  &  & Kodak 9: 0.093739\\ &  &  &  &  & Kodak 10: 0.094487\\ &  &  &  &  & Kodak 11: 0.095545\\ &  &  &  &  & Kodak 12: 0.093709\\ &  &  &  &  & Kodak 13: 0.090103\\ &  &  &  &  & Kodak 14: 0.094887\\ &  &  &  &  & Kodak 15: 0.092185\\ &  &  &  &  & Kodak 16: 0.097128\\ &  &  &  &  & Kodak 17: 0.101394\\ &  &  &  &  & Kodak 18: 0.094008\\ &  &  &  &  & Kodak 19: 0.100723\\ &  &  &  &  & Kodak 20: 0.093049\\ &  &  &  &  & Kodak 21: 0.093745\\ &  &  &  &  & Kodak 22: 0.093579\\ &  &  &  &  & Kodak 23: 0.095826\\ &  &  &  &  & Kodak 24: 0.095424\\\hline\hline89 & MS-SSIM & 1.0 & 5x5deconv,2,548 & 5x5deconv,2,237 & Kodak 1: 0.285443\\ &  &  & 5x5deconv,2,260 & 5x5deconv,2,268 & Kodak 2: 0.272487\\ &  &  & 5x5deconv,2,320 & 5x5deconv,2,139 & Kodak 3: 0.272868\\ &  &  &  & 5x5deconv,2,3 & Kodak 4: 0.293440\\ &  &  &  &  & Kodak 5: 0.273089\\ &  &  &  &  & Kodak 6: 0.279287\\ &  &  &  &  & Kodak 7: 0.276006\\ &  &  &  &  & Kodak 8: 0.270715\\ &  &  &  &  & Kodak 9: 0.276796\\ &  &  &  &  & Kodak 10: 0.278134\\ &  &  &  &  & Kodak 11: 0.281851\\ &  &  &  &  & Kodak 12: 0.281436\\ &  &  &  &  & Kodak 13: 0.281114\\ &  &  &  &  & Kodak 14: 0.275840\\ &  &  &  &  & Kodak 15: 0.283114\\ &  &  &  &  & Kodak 16: 0.277540\\ &  &  &  &  & Kodak 17: 0.273394\\ &  &  &  &  & Kodak 18: 0.279330\\ &  &  &  &  & Kodak 19: 0.279665\\ &  &  &  &  & Kodak 20: 0.280737\\ &  &  &  &  & Kodak 21: 0.279188\\ &  &  &  &  & Kodak 22: 0.285004\\ &  &  &  &  & Kodak 23: 0.276343\\ &  &  &  &  & Kodak 24: 0.284039\\\hline\hline90 & MSE & 0.00625 & 5x5deconv,2,5 & 5x5deconv,2,7 & Kodak 1: 0.091279\\ &  &  & 5x5deconv,2,9 & 5x5deconv,2,7 & Kodak 2: 0.099905\\ &  &  & 5x5deconv,2,320 & 5x5deconv,2,4 & Kodak 3: 0.101902\\ &  &  &  & 5x5deconv,2,3 & Kodak 4: 0.100399\\ &  &  &  &  & Kodak 5: 0.097322\\ &  &  &  &  & Kodak 6: 0.094234\\ &  &  &  &  & Kodak 7: 0.097161\\ &  &  &  &  & Kodak 8: 0.101344\\ &  &  &  &  & Kodak 9: 0.092152\\ &  &  &  &  & Kodak 10: 0.098494\\ &  &  &  &  & Kodak 11: 0.096702\\ &  &  &  &  & Kodak 12: 0.095236\\ &  &  &  &  & Kodak 13: 0.097348\\ &  &  &  &  & Kodak 14: 0.101402\\ &  &  &  &  & Kodak 15: 0.099451\\ &  &  &  &  & Kodak 16: 0.098890\\ &  &  &  &  & Kodak 17: 0.095123\\ &  &  &  &  & Kodak 18: 0.100196\\ &  &  &  &  & Kodak 19: 0.096645\\ &  &  &  &  & Kodak 20: 0.099210\\ &  &  &  &  & Kodak 21: 0.098294\\ &  &  &  &  & Kodak 22: 0.100967\\ &  &  &  &  & Kodak 23: 0.098254\\ &  &  &  &  & Kodak 24: 0.096405\\\hline\hline91 & MSE & 0.00625 & 5x5deconv,2,86 & 5x5deconv,2,127 & Kodak 1: 0.167708\\ &  &  & 5x5deconv,2,127 & 5x5deconv,2,65 & Kodak 2: 0.168359\\ &  &  & 5x5deconv,2,320 & 5x5deconv,2,98 & Kodak 3: 0.163842\\ &  &  &  & 5x5deconv,2,3 & Kodak 4: 0.160105\\ &  &  &  &  & Kodak 5: 0.168813\\ &  &  &  &  & Kodak 6: 0.175810\\ &  &  &  &  & Kodak 7: 0.168072\\ &  &  &  &  & Kodak 8: 0.166378\\ &  &  &  &  & Kodak 9: 0.171732\\ &  &  &  &  & Kodak 10: 0.167522\\ &  &  &  &  & Kodak 11: 0.165876\\ &  &  &  &  & Kodak 12: 0.168901\\ &  &  &  &  & Kodak 13: 0.168178\\ &  &  &  &  & Kodak 14: 0.161383\\ &  &  &  &  & Kodak 15: 0.164875\\ &  &  &  &  & Kodak 16: 0.167065\\ &  &  &  &  & Kodak 17: 0.171907\\ &  &  &  &  & Kodak 18: 0.166804\\ &  &  &  &  & Kodak 19: 0.160792\\ &  &  &  &  & Kodak 20: 0.167327\\ &  &  &  &  & Kodak 21: 0.171215\\ &  &  &  &  & Kodak 22: 0.173977\\ &  &  &  &  & Kodak 23: 0.165860\\ &  &  &  &  & Kodak 24: 0.168601\\\hline\hline92 & MSE & 0.00625 & 5x5deconv,2,10 & 5x5deconv,2,1 & Kodak 1: 0.090154\\ &  &  & 5x5deconv,2,10 & 5x5deconv,2,3 & Kodak 2: 0.094896\\ &  &  & 5x5deconv,2,320 & 5x5deconv,2,1 & Kodak 3: 0.094720\\ &  &  &  & 5x5deconv,2,3 & Kodak 4: 0.098545\\ &  &  &  &  & Kodak 5: 0.096098\\ &  &  &  &  & Kodak 6: 0.094433\\ &  &  &  &  & Kodak 7: 0.096432\\ &  &  &  &  & Kodak 8: 0.098041\\ &  &  &  &  & Kodak 9: 0.095109\\ &  &  &  &  & Kodak 10: 0.096138\\ &  &  &  &  & Kodak 11: 0.092773\\ &  &  &  &  & Kodak 12: 0.096935\\ &  &  &  &  & Kodak 13: 0.094188\\ &  &  &  &  & Kodak 14: 0.097670\\ &  &  &  &  & Kodak 15: 0.101815\\ &  &  &  &  & Kodak 16: 0.093623\\ &  &  &  &  & Kodak 17: 0.097134\\ &  &  &  &  & Kodak 18: 0.096462\\ &  &  &  &  & Kodak 19: 0.096825\\ &  &  &  &  & Kodak 20: 0.097313\\ &  &  &  &  & Kodak 21: 0.096147\\ &  &  &  &  & Kodak 22: 0.098282\\ &  &  &  &  & Kodak 23: 0.100980\\ &  &  &  &  & Kodak 24: 0.096372\\\hline\hline93 & MSE & 0.00625 & 5x5deconv,2,69 & 5x5deconv,2,320 & Kodak 1: 0.469171\\ &  &  & 5x5deconv,2,272 & 5x5deconv,2,320 & Kodak 2: 0.457613\\ &  &  & 5x5deconv,2,320 & 5x5deconv,2,320 & Kodak 3: 0.451504\\ &  &  &  & 5x5deconv,2,3 & Kodak 4: 0.459258\\ &  &  &  &  & Kodak 5: 0.455389\\ &  &  &  &  & Kodak 6: 0.474212\\ &  &  &  &  & Kodak 7: 0.472278\\ &  &  &  &  & Kodak 8: 0.479848\\ &  &  &  &  & Kodak 9: 0.459147\\ &  &  &  &  & Kodak 10: 0.461161\\ &  &  &  &  & Kodak 11: 0.458348\\ &  &  &  &  & Kodak 12: 0.456942\\ &  &  &  &  & Kodak 13: 0.464158\\ &  &  &  &  & Kodak 14: 0.457513\\ &  &  &  &  & Kodak 15: 0.462915\\ &  &  &  &  & Kodak 16: 0.477508\\ &  &  &  &  & Kodak 17: 0.464681\\ &  &  &  &  & Kodak 18: 0.466813\\ &  &  &  &  & Kodak 19: 0.456621\\ &  &  &  &  & Kodak 20: 0.459765\\ &  &  &  &  & Kodak 21: 0.484829\\ &  &  &  &  & Kodak 22: 0.462098\\ &  &  &  &  & Kodak 23: 0.457839\\ &  &  &  &  & Kodak 24: 0.457438\\\hline\hline94 & MSE & 0.00625 & 5x5deconv,2,321 & 5x5deconv,2,248 & Kodak 1: 0.293774\\ &  &  & 5x5deconv,2,194 & 5x5deconv,2,124 & Kodak 2: 0.286762\\ &  &  & 5x5deconv,2,320 & 5x5deconv,2,251 & Kodak 3: 0.283007\\ &  &  &  & 5x5deconv,2,3 & Kodak 4: 0.284478\\ &  &  &  &  & Kodak 5: 0.287500\\ &  &  &  &  & Kodak 6: 0.281504\\ &  &  &  &  & Kodak 7: 0.284773\\ &  &  &  &  & Kodak 8: 0.284351\\ &  &  &  &  & Kodak 9: 0.283759\\ &  &  &  &  & Kodak 10: 0.282859\\ &  &  &  &  & Kodak 11: 0.280224\\ &  &  &  &  & Kodak 12: 0.283613\\ &  &  &  &  & Kodak 13: 0.288776\\ &  &  &  &  & Kodak 14: 0.280596\\ &  &  &  &  & Kodak 15: 0.277580\\ &  &  &  &  & Kodak 16: 0.286193\\ &  &  &  &  & Kodak 17: 0.283446\\ &  &  &  &  & Kodak 18: 0.296230\\ &  &  &  &  & Kodak 19: 0.283190\\ &  &  &  &  & Kodak 20: 0.286955\\ &  &  &  &  & Kodak 21: 0.285349\\ &  &  &  &  & Kodak 22: 0.284321\\ &  &  &  &  & Kodak 23: 0.280665\\ &  &  &  &  & Kodak 24: 0.285309\\\hline\hline95 & MSE & 0.00625 & 5x5deconv,2,9 & 5x5deconv,2,10 & Kodak 1: 0.098289\\ &  &  & 5x5deconv,2,11 & 5x5deconv,2,11 & Kodak 2: 0.106955\\ &  &  & 5x5deconv,2,320 & 5x5deconv,2,10 & Kodak 3: 0.103761\\ &  &  &  & 5x5deconv,2,3 & Kodak 4: 0.105213\\ &  &  &  &  & Kodak 5: 0.101070\\ &  &  &  &  & Kodak 6: 0.111941\\ &  &  &  &  & Kodak 7: 0.107037\\ &  &  &  &  & Kodak 8: 0.101674\\ &  &  &  &  & Kodak 9: 0.104069\\ &  &  &  &  & Kodak 10: 0.098036\\ &  &  &  &  & Kodak 11: 0.101552\\ &  &  &  &  & Kodak 12: 0.103246\\ &  &  &  &  & Kodak 13: 0.103598\\ &  &  &  &  & Kodak 14: 0.098729\\ &  &  &  &  & Kodak 15: 0.105547\\ &  &  &  &  & Kodak 16: 0.105503\\ &  &  &  &  & Kodak 17: 0.107250\\ &  &  &  &  & Kodak 18: 0.102964\\ &  &  &  &  & Kodak 19: 0.104738\\ &  &  &  &  & Kodak 20: 0.102863\\ &  &  &  &  & Kodak 21: 0.102875\\ &  &  &  &  & Kodak 22: 0.102647\\ &  &  &  &  & Kodak 23: 0.103313\\ &  &  &  &  & Kodak 24: 0.111539\\\hline\hline96 & MSE & 0.00625 & 5x5deconv,2,33 & 5x5deconv,2,27 & Kodak 1: 0.113869\\ &  &  & 5x5deconv,2,27 & 5x5deconv,2,24 & Kodak 2: 0.112267\\ &  &  & 5x5deconv,2,320 & 5x5deconv,2,24 & Kodak 3: 0.119182\\ &  &  &  & 5x5deconv,2,3 & Kodak 4: 0.116199\\ &  &  &  &  & Kodak 5: 0.117410\\ &  &  &  &  & Kodak 6: 0.116891\\ &  &  &  &  & Kodak 7: 0.115519\\ &  &  &  &  & Kodak 8: 0.125990\\ &  &  &  &  & Kodak 9: 0.111071\\ &  &  &  &  & Kodak 10: 0.113015\\ &  &  &  &  & Kodak 11: 0.108013\\ &  &  &  &  & Kodak 12: 0.119387\\ &  &  &  &  & Kodak 13: 0.113281\\ &  &  &  &  & Kodak 14: 0.115581\\ &  &  &  &  & Kodak 15: 0.112837\\ &  &  &  &  & Kodak 16: 0.118988\\ &  &  &  &  & Kodak 17: 0.115726\\ &  &  &  &  & Kodak 18: 0.120853\\ &  &  &  &  & Kodak 19: 0.112788\\ &  &  &  &  & Kodak 20: 0.119167\\ &  &  &  &  & Kodak 21: 0.115860\\ &  &  &  &  & Kodak 22: 0.116596\\ &  &  &  &  & Kodak 23: 0.111770\\ &  &  &  &  & Kodak 24: 0.120979\\\hline\hline97 & MSE & 0.00625 & 5x5deconv,2,10 & 5x5deconv,2,1 & Kodak 1: 0.088365\\ &  &  & 5x5deconv,2,10 & 5x5deconv,2,4 & Kodak 2: 0.095348\\ &  &  & 5x5deconv,2,320 & 5x5deconv,2,1 & Kodak 3: 0.102350\\ &  &  &  & 5x5deconv,2,3 & Kodak 4: 0.098357\\ &  &  &  &  & Kodak 5: 0.115447\\ &  &  &  &  & Kodak 6: 0.093545\\ &  &  &  &  & Kodak 7: 0.096448\\ &  &  &  &  & Kodak 8: 0.092679\\ &  &  &  &  & Kodak 9: 0.092130\\ &  &  &  &  & Kodak 10: 0.096271\\ &  &  &  &  & Kodak 11: 0.096687\\ &  &  &  &  & Kodak 12: 0.093352\\ &  &  &  &  & Kodak 13: 0.103985\\ &  &  &  &  & Kodak 14: 0.094847\\ &  &  &  &  & Kodak 15: 0.094612\\ &  &  &  &  & Kodak 16: 0.098751\\ &  &  &  &  & Kodak 17: 0.094593\\ &  &  &  &  & Kodak 18: 0.096921\\ &  &  &  &  & Kodak 19: 0.097478\\ &  &  &  &  & Kodak 20: 0.096122\\ &  &  &  &  & Kodak 21: 0.096395\\ &  &  &  &  & Kodak 22: 0.098730\\ &  &  &  &  & Kodak 23: 0.093176\\ &  &  &  &  & Kodak 24: 0.097272\\\hline\hline98 & MSE & 0.00625 & 5x5deconv,2,195 & 5x5deconv,2,320 & Kodak 1: 0.444449\\ &  &  & 5x5deconv,2,247 & 5x5deconv,2,276 & Kodak 2: 0.429200\\ &  &  & 5x5deconv,2,320 & 5x5deconv,2,319 & Kodak 3: 0.431259\\ &  &  &  & 5x5deconv,2,3 & Kodak 4: 0.446040\\ &  &  &  &  & Kodak 5: 0.428383\\ &  &  &  &  & Kodak 6: 0.431587\\ &  &  &  &  & Kodak 7: 0.428353\\ &  &  &  &  & Kodak 8: 0.429060\\ &  &  &  &  & Kodak 9: 0.428905\\ &  &  &  &  & Kodak 10: 0.434910\\ &  &  &  &  & Kodak 11: 0.442609\\ &  &  &  &  & Kodak 12: 0.431109\\ &  &  &  &  & Kodak 13: 0.435253\\ &  &  &  &  & Kodak 14: 0.430797\\ &  &  &  &  & Kodak 15: 0.433208\\ &  &  &  &  & Kodak 16: 0.429315\\ &  &  &  &  & Kodak 17: 0.437388\\ &  &  &  &  & Kodak 18: 0.453618\\ &  &  &  &  & Kodak 19: 0.433650\\ &  &  &  &  & Kodak 20: 0.434790\\ &  &  &  &  & Kodak 21: 0.434229\\ &  &  &  &  & Kodak 22: 0.435367\\ &  &  &  &  & Kodak 23: 0.428646\\ &  &  &  &  & Kodak 24: 0.430835\\\hline\hline99 & MSE & 0.00625 & 5x5deconv,2,67 & 5x5deconv,2,74 & Kodak 1: 0.132833\\ &  &  & 5x5deconv,2,78 & 5x5deconv,2,34 & Kodak 2: 0.130773\\ &  &  & 5x5deconv,2,320 & 5x5deconv,2,42 & Kodak 3: 0.125924\\ &  &  &  & 5x5deconv,2,3 & Kodak 4: 0.124230\\ &  &  &  &  & Kodak 5: 0.140724\\ &  &  &  &  & Kodak 6: 0.125026\\ &  &  &  &  & Kodak 7: 0.133712\\ &  &  &  &  & Kodak 8: 0.136889\\ &  &  &  &  & Kodak 9: 0.131233\\ &  &  &  &  & Kodak 10: 0.127386\\ &  &  &  &  & Kodak 11: 0.131825\\ &  &  &  &  & Kodak 12: 0.132510\\ &  &  &  &  & Kodak 13: 0.136288\\ &  &  &  &  & Kodak 14: 0.134666\\ &  &  &  &  & Kodak 15: 0.128942\\ &  &  &  &  & Kodak 16: 0.122728\\ &  &  &  &  & Kodak 17: 0.124976\\ &  &  &  &  & Kodak 18: 0.131202\\ &  &  &  &  & Kodak 19: 0.133144\\ &  &  &  &  & Kodak 20: 0.129193\\ &  &  &  &  & Kodak 21: 0.132811\\ &  &  &  &  & Kodak 22: 0.125590\\ &  &  &  &  & Kodak 23: 0.127695\\ &  &  &  &  & Kodak 24: 0.136559\\\hline\hline100 & MSE & 0.00625 & 5x5deconv,2,10 & 5x5deconv,2,1 & Kodak 1: 0.093637\\ &  &  & 5x5deconv,2,10 & 5x5deconv,2,5 & Kodak 2: 0.102904\\ &  &  & 5x5deconv,2,320 & 5x5deconv,2,1 & Kodak 3: 0.101212\\ &  &  &  & 5x5deconv,2,3 & Kodak 4: 0.104803\\ &  &  &  &  & Kodak 5: 0.098383\\ &  &  &  &  & Kodak 6: 0.099826\\ &  &  &  &  & Kodak 7: 0.104390\\ &  &  &  &  & Kodak 8: 0.095282\\ &  &  &  &  & Kodak 9: 0.100180\\ &  &  &  &  & Kodak 10: 0.104843\\ &  &  &  &  & Kodak 11: 0.103557\\ &  &  &  &  & Kodak 12: 0.101010\\ &  &  &  &  & Kodak 13: 0.104189\\ &  &  &  &  & Kodak 14: 0.097168\\ &  &  &  &  & Kodak 15: 0.102984\\ &  &  &  &  & Kodak 16: 0.110058\\ &  &  &  &  & Kodak 17: 0.100320\\ &  &  &  &  & Kodak 18: 0.102334\\ &  &  &  &  & Kodak 19: 0.098099\\ &  &  &  &  & Kodak 20: 0.102844\\ &  &  &  &  & Kodak 21: 0.100157\\ &  &  &  &  & Kodak 22: 0.097695\\ &  &  &  &  & Kodak 23: 0.102039\\ &  &  &  &  & Kodak 24: 0.100096\\\hline\hline101 & MSE & 0.00625 & 5x5deconv,2,98 & 5x5deconv,2,320 & Kodak 1: 0.499599\\ &  &  & 5x5deconv,2,301 & 5x5deconv,2,319 & Kodak 2: 0.471103\\ &  &  & 5x5deconv,2,320 & 5x5deconv,2,320 & Kodak 3: 0.482218\\ &  &  &  & 5x5deconv,2,3 & Kodak 4: 0.474611\\ &  &  &  &  & Kodak 5: 0.474334\\ &  &  &  &  & Kodak 6: 0.493934\\ &  &  &  &  & Kodak 7: 0.480521\\ &  &  &  &  & Kodak 8: 0.474176\\ &  &  &  &  & Kodak 9: 0.469563\\ &  &  &  &  & Kodak 10: 0.468386\\ &  &  &  &  & Kodak 11: 0.475829\\ &  &  &  &  & Kodak 12: 0.523411\\ &  &  &  &  & Kodak 13: 0.469697\\ &  &  &  &  & Kodak 14: 0.470446\\ &  &  &  &  & Kodak 15: 0.477881\\ &  &  &  &  & Kodak 16: 0.482084\\ &  &  &  &  & Kodak 17: 0.469746\\ &  &  &  &  & Kodak 18: 0.486263\\ &  &  &  &  & Kodak 19: 0.471147\\ &  &  &  &  & Kodak 20: 0.525680\\ &  &  &  &  & Kodak 21: 0.475704\\ &  &  &  &  & Kodak 22: 0.472035\\ &  &  &  &  & Kodak 23: 0.474129\\ &  &  &  &  & Kodak 24: 0.469961\\\hline\hline102 & MS-SSIM & 0.5 & 5x5deconv,2,10 & 5x5deconv,2,1 & Kodak 1: 0.098219\\ &  &  & 5x5deconv,2,10 & 5x5deconv,2,1 & Kodak 2: 0.099931\\ &  &  & 5x5deconv,2,320 & 5x5deconv,2,1 & Kodak 3: 0.099856\\ &  &  &  & 5x5deconv,2,3 & Kodak 4: 0.100465\\ &  &  &  &  & Kodak 5: 0.105798\\ &  &  &  &  & Kodak 6: 0.100759\\ &  &  &  &  & Kodak 7: 0.100932\\ &  &  &  &  & Kodak 8: 0.099745\\ &  &  &  &  & Kodak 9: 0.102379\\ &  &  &  &  & Kodak 10: 0.099805\\ &  &  &  &  & Kodak 11: 0.107330\\ &  &  &  &  & Kodak 12: 0.097527\\ &  &  &  &  & Kodak 13: 0.095664\\ &  &  &  &  & Kodak 14: 0.102278\\ &  &  &  &  & Kodak 15: 0.101984\\ &  &  &  &  & Kodak 16: 0.102760\\ &  &  &  &  & Kodak 17: 0.099597\\ &  &  &  &  & Kodak 18: 0.098948\\ &  &  &  &  & Kodak 19: 0.098945\\ &  &  &  &  & Kodak 20: 0.096947\\ &  &  &  &  & Kodak 21: 0.099885\\ &  &  &  &  & Kodak 22: 0.097324\\ &  &  &  &  & Kodak 23: 0.095344\\ &  &  &  &  & Kodak 24: 0.101131\\\hline\hline103 & MS-SSIM & 0.5 & 5x5deconv,2,395 & 5x5deconv,2,181 & Kodak 1: 0.217327\\ &  &  & 5x5deconv,2,138 & 5x5deconv,2,192 & Kodak 2: 0.220578\\ &  &  & 5x5deconv,2,320 & 5x5deconv,2,117 & Kodak 3: 0.248516\\ &  &  &  & 5x5deconv,2,3 & Kodak 4: 0.219423\\ &  &  &  &  & Kodak 5: 0.220858\\ &  &  &  &  & Kodak 6: 0.226007\\ &  &  &  &  & Kodak 7: 0.226147\\ &  &  &  &  & Kodak 8: 0.230303\\ &  &  &  &  & Kodak 9: 0.219276\\ &  &  &  &  & Kodak 10: 0.221397\\ &  &  &  &  & Kodak 11: 0.223229\\ &  &  &  &  & Kodak 12: 0.244699\\ &  &  &  &  & Kodak 13: 0.230366\\ &  &  &  &  & Kodak 14: 0.251322\\ &  &  &  &  & Kodak 15: 0.225948\\ &  &  &  &  & Kodak 16: 0.227646\\ &  &  &  &  & Kodak 17: 0.220220\\ &  &  &  &  & Kodak 18: 0.221163\\ &  &  &  &  & Kodak 19: 0.225448\\ &  &  &  &  & Kodak 20: 0.214402\\ &  &  &  &  & Kodak 21: 0.221144\\ &  &  &  &  & Kodak 22: 0.247117\\ &  &  &  &  & Kodak 23: 0.220775\\ &  &  &  &  & Kodak 24: 0.222309\\\hline\hline104 & MS-SSIM & 0.5 & 5x5deconv,2,43 & 5x5deconv,2,34 & Kodak 1: 0.108619\\ &  &  & 5x5deconv,2,24 & 5x5deconv,2,25 & Kodak 2: 0.102130\\ &  &  & 5x5deconv,2,320 & 5x5deconv,2,8 & Kodak 3: 0.111988\\ &  &  &  & 5x5deconv,2,3 & Kodak 4: 0.112993\\ &  &  &  &  & Kodak 5: 0.113921\\ &  &  &  &  & Kodak 6: 0.107526\\ &  &  &  &  & Kodak 7: 0.109068\\ &  &  &  &  & Kodak 8: 0.112754\\ &  &  &  &  & Kodak 9: 0.112410\\ &  &  &  &  & Kodak 10: 0.109243\\ &  &  &  &  & Kodak 11: 0.112882\\ &  &  &  &  & Kodak 12: 0.107393\\ &  &  &  &  & Kodak 13: 0.119732\\ &  &  &  &  & Kodak 14: 0.117176\\ &  &  &  &  & Kodak 15: 0.113388\\ &  &  &  &  & Kodak 16: 0.120404\\ &  &  &  &  & Kodak 17: 0.112151\\ &  &  &  &  & Kodak 18: 0.110483\\ &  &  &  &  & Kodak 19: 0.112721\\ &  &  &  &  & Kodak 20: 0.112681\\ &  &  &  &  & Kodak 21: 0.106701\\ &  &  &  &  & Kodak 22: 0.110445\\ &  &  &  &  & Kodak 23: 0.109081\\ &  &  &  &  & Kodak 24: 0.110950\\\hline\hline105 & MS-SSIM & 0.5 & 5x5deconv,2,10 & 5x5deconv,2,1 & Kodak 1: 0.091596\\ &  &  & 5x5deconv,2,10 & 5x5deconv,2,1 & Kodak 2: 0.098569\\ &  &  & 5x5deconv,2,320 & 5x5deconv,2,1 & Kodak 3: 0.098692\\ &  &  &  & 5x5deconv,2,3 & Kodak 4: 0.095558\\ &  &  &  &  & Kodak 5: 0.102314\\ &  &  &  &  & Kodak 6: 0.097285\\ &  &  &  &  & Kodak 7: 0.099091\\ &  &  &  &  & Kodak 8: 0.096359\\ &  &  &  &  & Kodak 9: 0.099712\\ &  &  &  &  & Kodak 10: 0.101521\\ &  &  &  &  & Kodak 11: 0.100785\\ &  &  &  &  & Kodak 12: 0.098667\\ &  &  &  &  & Kodak 13: 0.104456\\ &  &  &  &  & Kodak 14: 0.096524\\ &  &  &  &  & Kodak 15: 0.097040\\ &  &  &  &  & Kodak 16: 0.102865\\ &  &  &  &  & Kodak 17: 0.097715\\ &  &  &  &  & Kodak 18: 0.098563\\ &  &  &  &  & Kodak 19: 0.100539\\ &  &  &  &  & Kodak 20: 0.095690\\ &  &  &  &  & Kodak 21: 0.099879\\ &  &  &  &  & Kodak 22: 0.097718\\ &  &  &  &  & Kodak 23: 0.103547\\ &  &  &  &  & Kodak 24: 0.104714\\\hline\hline106 & MS-SSIM & 0.5 & 5x5deconv,2,10 & 5x5deconv,2,1 & Kodak 1: 0.096959\\ &  &  & 5x5deconv,2,10 & 5x5deconv,2,1 & Kodak 2: 0.092966\\ &  &  & 5x5deconv,2,320 & 5x5deconv,2,1 & Kodak 3: 0.091932\\ &  &  &  & 5x5deconv,2,3 & Kodak 4: 0.089257\\ &  &  &  &  & Kodak 5: 0.088777\\ &  &  &  &  & Kodak 6: 0.092514\\ &  &  &  &  & Kodak 7: 0.095655\\ &  &  &  &  & Kodak 8: 0.098771\\ &  &  &  &  & Kodak 9: 0.098182\\ &  &  &  &  & Kodak 10: 0.087943\\ &  &  &  &  & Kodak 11: 0.091484\\ &  &  &  &  & Kodak 12: 0.097905\\ &  &  &  &  & Kodak 13: 0.099237\\ &  &  &  &  & Kodak 14: 0.096300\\ &  &  &  &  & Kodak 15: 0.089730\\ &  &  &  &  & Kodak 16: 0.098736\\ &  &  &  &  & Kodak 17: 0.097543\\ &  &  &  &  & Kodak 18: 0.094906\\ &  &  &  &  & Kodak 19: 0.090817\\ &  &  &  &  & Kodak 20: 0.090778\\ &  &  &  &  & Kodak 21: 0.089384\\ &  &  &  &  & Kodak 22: 0.087384\\ &  &  &  &  & Kodak 23: 0.090647\\ &  &  &  &  & Kodak 24: 0.091509\\\hline\hline107 & MS-SSIM & 0.5 & 5x5deconv,2,4 & 5x5deconv,2,9 & Kodak 1: 0.099958\\ &  &  & 5x5deconv,2,23 & 5x5deconv,2,23 & Kodak 2: 0.108528\\ &  &  & 5x5deconv,2,320 & 5x5deconv,2,2 & Kodak 3: 0.109055\\ &  &  &  & 5x5deconv,2,3 & Kodak 4: 0.127100\\ &  &  &  &  & Kodak 5: 0.105417\\ &  &  &  &  & Kodak 6: 0.104613\\ &  &  &  &  & Kodak 7: 0.105390\\ &  &  &  &  & Kodak 8: 0.104694\\ &  &  &  &  & Kodak 9: 0.106905\\ &  &  &  &  & Kodak 10: 0.099672\\ &  &  &  &  & Kodak 11: 0.101833\\ &  &  &  &  & Kodak 12: 0.105325\\ &  &  &  &  & Kodak 13: 0.104409\\ &  &  &  &  & Kodak 14: 0.114169\\ &  &  &  &  & Kodak 15: 0.102936\\ &  &  &  &  & Kodak 16: 0.100379\\ &  &  &  &  & Kodak 17: 0.105503\\ &  &  &  &  & Kodak 18: 0.100196\\ &  &  &  &  & Kodak 19: 0.113998\\ &  &  &  &  & Kodak 20: 0.102180\\ &  &  &  &  & Kodak 21: 0.103980\\ &  &  &  &  & Kodak 22: 0.106723\\ &  &  &  &  & Kodak 23: 0.103786\\ &  &  &  &  & Kodak 24: 0.107403\\\hline\hline108 & MS-SSIM & 0.5 & 5x5deconv,2,309 & 5x5deconv,2,233 & Kodak 1: 0.276674\\ &  &  & 5x5deconv,2,446 & 5x5deconv,2,290 & Kodak 2: 0.287468\\ &  &  & 5x5deconv,2,320 & 5x5deconv,2,136 & Kodak 3: 0.281028\\ &  &  &  & 5x5deconv,2,3 & Kodak 4: 0.286832\\ &  &  &  &  & Kodak 5: 0.288965\\ &  &  &  &  & Kodak 6: 0.294165\\ &  &  &  &  & Kodak 7: 0.288932\\ &  &  &  &  & Kodak 8: 0.293573\\ &  &  &  &  & Kodak 9: 0.288337\\ &  &  &  &  & Kodak 10: 0.290015\\ &  &  &  &  & Kodak 11: 0.290918\\ &  &  &  &  & Kodak 12: 0.289881\\ &  &  &  &  & Kodak 13: 0.291269\\ &  &  &  &  & Kodak 14: 0.291320\\ &  &  &  &  & Kodak 15: 0.288411\\ &  &  &  &  & Kodak 16: 0.288857\\ &  &  &  &  & Kodak 17: 0.292744\\ &  &  &  &  & Kodak 18: 0.291106\\ &  &  &  &  & Kodak 19: 0.284964\\ &  &  &  &  & Kodak 20: 0.288313\\ &  &  &  &  & Kodak 21: 0.285804\\ &  &  &  &  & Kodak 22: 0.291516\\ &  &  &  &  & Kodak 23: 0.291235\\ &  &  &  &  & Kodak 24: 0.318699\\\hline\hline109 & MS-SSIM & 0.5 & 5x5deconv,2,10 & 5x5deconv,2,1 & Kodak 1: 0.092120\\ &  &  & 5x5deconv,2,10 & 5x5deconv,2,1 & Kodak 2: 0.097861\\ &  &  & 5x5deconv,2,320 & 5x5deconv,2,1 & Kodak 3: 0.100374\\ &  &  &  & 5x5deconv,2,3 & Kodak 4: 0.098479\\ &  &  &  &  & Kodak 5: 0.102455\\ &  &  &  &  & Kodak 6: 0.096442\\ &  &  &  &  & Kodak 7: 0.096128\\ &  &  &  &  & Kodak 8: 0.099579\\ &  &  &  &  & Kodak 9: 0.097558\\ &  &  &  &  & Kodak 10: 0.097794\\ &  &  &  &  & Kodak 11: 0.097080\\ &  &  &  &  & Kodak 12: 0.097695\\ &  &  &  &  & Kodak 13: 0.096417\\ &  &  &  &  & Kodak 14: 0.096861\\ &  &  &  &  & Kodak 15: 0.106105\\ &  &  &  &  & Kodak 16: 0.096902\\ &  &  &  &  & Kodak 17: 0.099617\\ &  &  &  &  & Kodak 18: 0.102581\\ &  &  &  &  & Kodak 19: 0.104544\\ &  &  &  &  & Kodak 20: 0.101492\\ &  &  &  &  & Kodak 21: 0.097974\\ &  &  &  &  & Kodak 22: 0.104564\\ &  &  &  &  & Kodak 23: 0.102830\\ &  &  &  &  & Kodak 24: 0.103363\\\hline\hline110 & MS-SSIM & 0.5 & 5x5deconv,2,10 & 5x5deconv,2,5 & Kodak 1: 0.093957\\ &  &  & 5x5deconv,2,10 & 5x5deconv,2,10 & Kodak 2: 0.098009\\ &  &  & 5x5deconv,2,320 & 5x5deconv,2,1 & Kodak 3: 0.100520\\ &  &  &  & 5x5deconv,2,3 & Kodak 4: 0.098481\\ &  &  &  &  & Kodak 5: 0.106950\\ &  &  &  &  & Kodak 6: 0.101882\\ &  &  &  &  & Kodak 7: 0.098758\\ &  &  &  &  & Kodak 8: 0.097488\\ &  &  &  &  & Kodak 9: 0.100360\\ &  &  &  &  & Kodak 10: 0.107288\\ &  &  &  &  & Kodak 11: 0.104039\\ &  &  &  &  & Kodak 12: 0.098643\\ &  &  &  &  & Kodak 13: 0.106284\\ &  &  &  &  & Kodak 14: 0.110934\\ &  &  &  &  & Kodak 15: 0.105039\\ &  &  &  &  & Kodak 16: 0.099111\\ &  &  &  &  & Kodak 17: 0.115744\\ &  &  &  &  & Kodak 18: 0.101286\\ &  &  &  &  & Kodak 19: 0.100911\\ &  &  &  &  & Kodak 20: 0.103411\\ &  &  &  &  & Kodak 21: 0.104892\\ &  &  &  &  & Kodak 22: 0.111660\\ &  &  &  &  & Kodak 23: 0.103528\\ &  &  &  &  & Kodak 24: 0.098483\\\hline\hline111 & MS-SSIM & 0.5 & 5x5deconv,2,222 & 5x5deconv,2,107 & Kodak 1: 0.156406\\ &  &  & 5x5deconv,2,189 & 5x5deconv,2,119 & Kodak 2: 0.167934\\ &  &  & 5x5deconv,2,320 & 5x5deconv,2,56 & Kodak 3: 0.154224\\ &  &  &  & 5x5deconv,2,3 & Kodak 4: 0.165705\\ &  &  &  &  & Kodak 5: 0.161841\\ &  &  &  &  & Kodak 6: 0.160028\\ &  &  &  &  & Kodak 7: 0.160054\\ &  &  &  &  & Kodak 8: 0.165247\\ &  &  &  &  & Kodak 9: 0.156862\\ &  &  &  &  & Kodak 10: 0.160146\\ &  &  &  &  & Kodak 11: 0.160881\\ &  &  &  &  & Kodak 12: 0.164831\\ &  &  &  &  & Kodak 13: 0.163908\\ &  &  &  &  & Kodak 14: 0.165707\\ &  &  &  &  & Kodak 15: 0.155874\\ &  &  &  &  & Kodak 16: 0.152089\\ &  &  &  &  & Kodak 17: 0.158518\\ &  &  &  &  & Kodak 18: 0.161456\\ &  &  &  &  & Kodak 19: 0.163361\\ &  &  &  &  & Kodak 20: 0.162271\\ &  &  &  &  & Kodak 21: 0.168679\\ &  &  &  &  & Kodak 22: 0.159999\\ &  &  &  &  & Kodak 23: 0.166304\\ &  &  &  &  & Kodak 24: 0.152289\\\hline\hline112 & MS-SSIM & 0.5 & 5x5deconv,2,10 & 5x5deconv,2,1 & Kodak 1: 0.092305\\ &  &  & 5x5deconv,2,10 & 5x5deconv,2,1 & Kodak 2: 0.102060\\ &  &  & 5x5deconv,2,320 & 5x5deconv,2,1 & Kodak 3: 0.100578\\ &  &  &  & 5x5deconv,2,3 & Kodak 4: 0.096956\\ &  &  &  &  & Kodak 5: 0.104737\\ &  &  &  &  & Kodak 6: 0.093452\\ &  &  &  &  & Kodak 7: 0.105634\\ &  &  &  &  & Kodak 8: 0.099266\\ &  &  &  &  & Kodak 9: 0.099015\\ &  &  &  &  & Kodak 10: 0.099468\\ &  &  &  &  & Kodak 11: 0.103890\\ &  &  &  &  & Kodak 12: 0.096093\\ &  &  &  &  & Kodak 13: 0.097772\\ &  &  &  &  & Kodak 14: 0.102426\\ &  &  &  &  & Kodak 15: 0.102847\\ &  &  &  &  & Kodak 16: 0.103936\\ &  &  &  &  & Kodak 17: 0.103582\\ &  &  &  &  & Kodak 18: 0.106298\\ &  &  &  &  & Kodak 19: 0.097358\\ &  &  &  &  & Kodak 20: 0.106728\\ &  &  &  &  & Kodak 21: 0.103074\\ &  &  &  &  & Kodak 22: 0.105907\\ &  &  &  &  & Kodak 23: 0.109309\\ &  &  &  &  & Kodak 24: 0.098862\\\hline\hline113 & MS-SSIM & 0.5 & 5x5deconv,2,93 & 5x5deconv,2,48 & Kodak 1: 0.126707\\ &  &  & 5x5deconv,2,106 & 5x5deconv,2,112 & Kodak 2: 0.125048\\ &  &  & 5x5deconv,2,320 & 5x5deconv,2,11 & Kodak 3: 0.126230\\ &  &  &  & 5x5deconv,2,3 & Kodak 4: 0.118951\\ &  &  &  &  & Kodak 5: 0.129245\\ &  &  &  &  & Kodak 6: 0.135875\\ &  &  &  &  & Kodak 7: 0.132757\\ &  &  &  &  & Kodak 8: 0.134154\\ &  &  &  &  & Kodak 9: 0.133891\\ &  &  &  &  & Kodak 10: 0.130507\\ &  &  &  &  & Kodak 11: 0.127175\\ &  &  &  &  & Kodak 12: 0.127556\\ &  &  &  &  & Kodak 13: 0.128535\\ &  &  &  &  & Kodak 14: 0.132849\\ &  &  &  &  & Kodak 15: 0.134776\\ &  &  &  &  & Kodak 16: 0.128750\\ &  &  &  &  & Kodak 17: 0.138258\\ &  &  &  &  & Kodak 18: 0.124576\\ &  &  &  &  & Kodak 19: 0.135281\\ &  &  &  &  & Kodak 20: 0.137527\\ &  &  &  &  & Kodak 21: 0.147222\\ &  &  &  &  & Kodak 22: 0.127913\\ &  &  &  &  & Kodak 23: 0.129541\\ &  &  &  &  & Kodak 24: 0.149770\\\hline\hline114 & MS-SSIM & 8.0 & 5x5deconv,2,150 & 5x5deconv,2,260 & Kodak 1: 0.281719\\ &  &  & 5x5deconv,2,180 & 5x5deconv,2,181 & Kodak 2: 0.264412\\ &  &  & 5x5deconv,2,320 & 5x5deconv,2,160 & Kodak 3: 0.253847\\ &  &  &  & 5x5deconv,2,3 & Kodak 4: 0.264033\\ &  &  &  &  & Kodak 5: 0.262993\\ &  &  &  &  & Kodak 6: 0.263467\\ &  &  &  &  & Kodak 7: 0.257007\\ &  &  &  &  & Kodak 8: 0.255881\\ &  &  &  &  & Kodak 9: 0.257742\\ &  &  &  &  & Kodak 10: 0.285450\\ &  &  &  &  & Kodak 11: 0.258197\\ &  &  &  &  & Kodak 12: 0.255870\\ &  &  &  &  & Kodak 13: 0.304513\\ &  &  &  &  & Kodak 14: 0.268514\\ &  &  &  &  & Kodak 15: 0.254067\\ &  &  &  &  & Kodak 16: 0.299586\\ &  &  &  &  & Kodak 17: 0.291026\\ &  &  &  &  & Kodak 18: 0.268419\\ &  &  &  &  & Kodak 19: 0.295159\\ &  &  &  &  & Kodak 20: 0.258106\\ &  &  &  &  & Kodak 21: 0.261986\\ &  &  &  &  & Kodak 22: 0.258827\\ &  &  &  &  & Kodak 23: 0.263632\\ &  &  &  &  & Kodak 24: 0.261888\\\hline\hline115 & MS-SSIM & 8.0 & 5x5deconv,2,6 & 5x5deconv,2,14 & Kodak 1: 0.110130\\ &  &  & 5x5deconv,2,14 & 5x5deconv,2,20 & Kodak 2: 0.115959\\ &  &  & 5x5deconv,2,320 & 5x5deconv,2,6 & Kodak 3: 0.103825\\ &  &  &  & 5x5deconv,2,3 & Kodak 4: 0.111053\\ &  &  &  &  & Kodak 5: 0.114286\\ &  &  &  &  & Kodak 6: 0.107325\\ &  &  &  &  & Kodak 7: 0.103519\\ &  &  &  &  & Kodak 8: 0.106784\\ &  &  &  &  & Kodak 9: 0.119484\\ &  &  &  &  & Kodak 10: 0.104175\\ &  &  &  &  & Kodak 11: 0.102585\\ &  &  &  &  & Kodak 12: 0.115139\\ &  &  &  &  & Kodak 13: 0.109845\\ &  &  &  &  & Kodak 14: 0.111068\\ &  &  &  &  & Kodak 15: 0.108164\\ &  &  &  &  & Kodak 16: 0.114860\\ &  &  &  &  & Kodak 17: 0.112070\\ &  &  &  &  & Kodak 18: 0.109329\\ &  &  &  &  & Kodak 19: 0.108686\\ &  &  &  &  & Kodak 20: 0.111539\\ &  &  &  &  & Kodak 21: 0.110538\\ &  &  &  &  & Kodak 22: 0.106278\\ &  &  &  &  & Kodak 23: 0.104613\\ &  &  &  &  & Kodak 24: 0.112123\\\hline\hline116 & MS-SSIM & 8.0 & 5x5deconv,2,10 & 5x5deconv,2,1 & Kodak 1: 0.095971\\ &  &  & 5x5deconv,2,10 & 5x5deconv,2,6 & Kodak 2: 0.104412\\ &  &  & 5x5deconv,2,320 & 5x5deconv,2,1 & Kodak 3: 0.098535\\ &  &  &  & 5x5deconv,2,3 & Kodak 4: 0.101694\\ &  &  &  &  & Kodak 5: 0.099018\\ &  &  &  &  & Kodak 6: 0.110770\\ &  &  &  &  & Kodak 7: 0.103186\\ &  &  &  &  & Kodak 8: 0.096886\\ &  &  &  &  & Kodak 9: 0.100820\\ &  &  &  &  & Kodak 10: 0.095259\\ &  &  &  &  & Kodak 11: 0.113202\\ &  &  &  &  & Kodak 12: 0.108632\\ &  &  &  &  & Kodak 13: 0.100514\\ &  &  &  &  & Kodak 14: 0.098073\\ &  &  &  &  & Kodak 15: 0.105589\\ &  &  &  &  & Kodak 16: 0.099448\\ &  &  &  &  & Kodak 17: 0.098434\\ &  &  &  &  & Kodak 18: 0.105247\\ &  &  &  &  & Kodak 19: 0.104778\\ &  &  &  &  & Kodak 20: 0.108030\\ &  &  &  &  & Kodak 21: 0.100427\\ &  &  &  &  & Kodak 22: 0.100259\\ &  &  &  &  & Kodak 23: 0.108623\\ &  &  &  &  & Kodak 24: 0.109427\\\hline\hline117 & MS-SSIM & 8.0 & 5x5deconv,2,249 & 5x5deconv,2,218 & Kodak 1: 0.202842\\ &  &  & 5x5deconv,2,147 & 5x5deconv,2,112 & Kodak 2: 0.217406\\ &  &  & 5x5deconv,2,320 & 5x5deconv,2,121 & Kodak 3: 0.205609\\ &  &  &  & 5x5deconv,2,3 & Kodak 4: 0.211451\\ &  &  &  &  & Kodak 5: 0.203045\\ &  &  &  &  & Kodak 6: 0.238921\\ &  &  &  &  & Kodak 7: 0.212911\\ &  &  &  &  & Kodak 8: 0.207102\\ &  &  &  &  & Kodak 9: 0.209465\\ &  &  &  &  & Kodak 10: 0.214373\\ &  &  &  &  & Kodak 11: 0.205199\\ &  &  &  &  & Kodak 12: 0.210432\\ &  &  &  &  & Kodak 13: 0.206860\\ &  &  &  &  & Kodak 14: 0.238813\\ &  &  &  &  & Kodak 15: 0.210873\\ &  &  &  &  & Kodak 16: 0.213135\\ &  &  &  &  & Kodak 17: 0.205823\\ &  &  &  &  & Kodak 18: 0.231187\\ &  &  &  &  & Kodak 19: 0.214554\\ &  &  &  &  & Kodak 20: 0.215605\\ &  &  &  &  & Kodak 21: 0.213762\\ &  &  &  &  & Kodak 22: 0.239792\\ &  &  &  &  & Kodak 23: 0.204109\\ &  &  &  &  & Kodak 24: 0.208833\\\hline\hline118 & MS-SSIM & 8.0 & 5x5deconv,2,49 & 5x5deconv,2,96 & Kodak 1: 0.138990\\ &  &  & 5x5deconv,2,62 & 5x5deconv,2,37 & Kodak 2: 0.145092\\ &  &  & 5x5deconv,2,320 & 5x5deconv,2,45 & Kodak 3: 0.129620\\ &  &  &  & 5x5deconv,2,3 & Kodak 4: 0.136966\\ &  &  &  &  & Kodak 5: 0.135976\\ &  &  &  &  & Kodak 6: 0.140166\\ &  &  &  &  & Kodak 7: 0.136217\\ &  &  &  &  & Kodak 8: 0.144711\\ &  &  &  &  & Kodak 9: 0.147020\\ &  &  &  &  & Kodak 10: 0.133757\\ &  &  &  &  & Kodak 11: 0.138187\\ &  &  &  &  & Kodak 12: 0.139690\\ &  &  &  &  & Kodak 13: 0.134551\\ &  &  &  &  & Kodak 14: 0.138912\\ &  &  &  &  & Kodak 15: 0.138832\\ &  &  &  &  & Kodak 16: 0.137120\\ &  &  &  &  & Kodak 17: 0.139633\\ &  &  &  &  & Kodak 18: 0.140854\\ &  &  &  &  & Kodak 19: 0.139804\\ &  &  &  &  & Kodak 20: 0.132762\\ &  &  &  &  & Kodak 21: 0.144971\\ &  &  &  &  & Kodak 22: 0.137973\\ &  &  &  &  & Kodak 23: 0.153518\\ &  &  &  &  & Kodak 24: 0.138809\\\hline\hline119 & MS-SSIM & 8.0 & 5x5deconv,2,10 & 5x5deconv,2,1 & Kodak 1: 0.094787\\ &  &  & 5x5deconv,2,10 & 5x5deconv,2,1 & Kodak 2: 0.100170\\ &  &  & 5x5deconv,2,320 & 5x5deconv,2,1 & Kodak 3: 0.101838\\ &  &  &  & 5x5deconv,2,3 & Kodak 4: 0.100501\\ &  &  &  &  & Kodak 5: 0.098477\\ &  &  &  &  & Kodak 6: 0.102280\\ &  &  &  &  & Kodak 7: 0.099734\\ &  &  &  &  & Kodak 8: 0.098042\\ &  &  &  &  & Kodak 9: 0.098003\\ &  &  &  &  & Kodak 10: 0.095278\\ &  &  &  &  & Kodak 11: 0.100857\\ &  &  &  &  & Kodak 12: 0.097385\\ &  &  &  &  & Kodak 13: 0.096943\\ &  &  &  &  & Kodak 14: 0.098407\\ &  &  &  &  & Kodak 15: 0.097299\\ &  &  &  &  & Kodak 16: 0.098141\\ &  &  &  &  & Kodak 17: 0.097923\\ &  &  &  &  & Kodak 18: 0.096515\\ &  &  &  &  & Kodak 19: 0.095600\\ &  &  &  &  & Kodak 20: 0.099790\\ &  &  &  &  & Kodak 21: 0.097795\\ &  &  &  &  & Kodak 22: 0.101406\\ &  &  &  &  & Kodak 23: 0.101437\\ &  &  &  &  & Kodak 24: 0.103390\\\hline\hline120 & MS-SSIM & 8.0 & 5x5deconv,2,10 & 5x5deconv,2,5 & Kodak 1: 0.104829\\ &  &  & 5x5deconv,2,10 & 5x5deconv,2,12 & Kodak 2: 0.100597\\ &  &  & 5x5deconv,2,320 & 5x5deconv,2,3 & Kodak 3: 0.099614\\ &  &  &  & 5x5deconv,2,3 & Kodak 4: 0.105048\\ &  &  &  &  & Kodak 5: 0.115354\\ &  &  &  &  & Kodak 6: 0.102562\\ &  &  &  &  & Kodak 7: 0.103125\\ &  &  &  &  & Kodak 8: 0.104111\\ &  &  &  &  & Kodak 9: 0.102253\\ &  &  &  &  & Kodak 10: 0.107209\\ &  &  &  &  & Kodak 11: 0.105078\\ &  &  &  &  & Kodak 12: 0.104298\\ &  &  &  &  & Kodak 13: 0.100027\\ &  &  &  &  & Kodak 14: 0.103818\\ &  &  &  &  & Kodak 15: 0.098801\\ &  &  &  &  & Kodak 16: 0.100646\\ &  &  &  &  & Kodak 17: 0.113706\\ &  &  &  &  & Kodak 18: 0.105628\\ &  &  &  &  & Kodak 19: 0.102009\\ &  &  &  &  & Kodak 20: 0.097074\\ &  &  &  &  & Kodak 21: 0.099720\\ &  &  &  &  & Kodak 22: 0.107270\\ &  &  &  &  & Kodak 23: 0.098218\\ &  &  &  &  & Kodak 24: 0.103264\\\hline\hline121 & MS-SSIM & 8.0 & 5x5deconv,2,104 & 5x5deconv,2,153 & Kodak 1: 0.160916\\ &  &  & 5x5deconv,2,90 & 5x5deconv,2,65 & Kodak 2: 0.163355\\ &  &  & 5x5deconv,2,320 & 5x5deconv,2,79 & Kodak 3: 0.164418\\ &  &  &  & 5x5deconv,2,3 & Kodak 4: 0.165571\\ &  &  &  &  & Kodak 5: 0.156477\\ &  &  &  &  & Kodak 6: 0.166202\\ &  &  &  &  & Kodak 7: 0.185474\\ &  &  &  &  & Kodak 8: 0.155135\\ &  &  &  &  & Kodak 9: 0.162974\\ &  &  &  &  & Kodak 10: 0.162827\\ &  &  &  &  & Kodak 11: 0.161115\\ &  &  &  &  & Kodak 12: 0.159137\\ &  &  &  &  & Kodak 13: 0.170570\\ &  &  &  &  & Kodak 14: 0.166179\\ &  &  &  &  & Kodak 15: 0.174125\\ &  &  &  &  & Kodak 16: 0.164690\\ &  &  &  &  & Kodak 17: 0.154549\\ &  &  &  &  & Kodak 18: 0.163537\\ &  &  &  &  & Kodak 19: 0.159968\\ &  &  &  &  & Kodak 20: 0.168827\\ &  &  &  &  & Kodak 21: 0.156196\\ &  &  &  &  & Kodak 22: 0.171386\\ &  &  &  &  & Kodak 23: 0.184430\\ &  &  &  &  & Kodak 24: 0.187173\\\hline\hline122 & MS-SSIM & 8.0 & 5x5deconv,2,10 & 5x5deconv,2,1 & Kodak 1: 0.093223\\ &  &  & 5x5deconv,2,10 & 5x5deconv,2,1 & Kodak 2: 0.101900\\ &  &  & 5x5deconv,2,320 & 5x5deconv,2,1 & Kodak 3: 0.098201\\ &  &  &  & 5x5deconv,2,3 & Kodak 4: 0.101484\\ &  &  &  &  & Kodak 5: 0.098036\\ &  &  &  &  & Kodak 6: 0.098977\\ &  &  &  &  & Kodak 7: 0.101355\\ &  &  &  &  & Kodak 8: 0.098815\\ &  &  &  &  & Kodak 9: 0.111111\\ &  &  &  &  & Kodak 10: 0.099097\\ &  &  &  &  & Kodak 11: 0.099603\\ &  &  &  &  & Kodak 12: 0.097287\\ &  &  &  &  & Kodak 13: 0.097203\\ &  &  &  &  & Kodak 14: 0.108905\\ &  &  &  &  & Kodak 15: 0.097462\\ &  &  &  &  & Kodak 16: 0.102683\\ &  &  &  &  & Kodak 17: 0.093793\\ &  &  &  &  & Kodak 18: 0.097697\\ &  &  &  &  & Kodak 19: 0.099278\\ &  &  &  &  & Kodak 20: 0.095024\\ &  &  &  &  & Kodak 21: 0.099861\\ &  &  &  &  & Kodak 22: 0.096950\\ &  &  &  &  & Kodak 23: 0.111553\\ &  &  &  &  & Kodak 24: 0.098963\\\hline\hline123 & MS-SSIM & 8.0 & 5x5deconv,2,6 & 5x5deconv,2,14 & Kodak 1: 0.108465\\ &  &  & 5x5deconv,2,14 & 5x5deconv,2,20 & Kodak 2: 0.112835\\ &  &  & 5x5deconv,2,320 & 5x5deconv,2,7 & Kodak 3: 0.102311\\ &  &  &  & 5x5deconv,2,3 & Kodak 4: 0.117711\\ &  &  &  &  & Kodak 5: 0.120406\\ &  &  &  &  & Kodak 6: 0.119241\\ &  &  &  &  & Kodak 7: 0.106413\\ &  &  &  &  & Kodak 8: 0.108401\\ &  &  &  &  & Kodak 9: 0.109727\\ &  &  &  &  & Kodak 10: 0.110268\\ &  &  &  &  & Kodak 11: 0.114715\\ &  &  &  &  & Kodak 12: 0.114643\\ &  &  &  &  & Kodak 13: 0.113129\\ &  &  &  &  & Kodak 14: 0.111303\\ &  &  &  &  & Kodak 15: 0.110581\\ &  &  &  &  & Kodak 16: 0.119344\\ &  &  &  &  & Kodak 17: 0.113204\\ &  &  &  &  & Kodak 18: 0.114282\\ &  &  &  &  & Kodak 19: 0.116643\\ &  &  &  &  & Kodak 20: 0.111988\\ &  &  &  &  & Kodak 21: 0.109104\\ &  &  &  &  & Kodak 22: 0.108409\\ &  &  &  &  & Kodak 23: 0.116546\\ &  &  &  &  & Kodak 24: 0.121679\\\hline\hline124 & MS-SSIM & 8.0 & 5x5deconv,2,10 & 5x5deconv,2,1 & Kodak 1: 0.090816\\ &  &  & 5x5deconv,2,10 & 5x5deconv,2,1 & Kodak 2: 0.096069\\ &  &  & 5x5deconv,2,320 & 5x5deconv,2,1 & Kodak 3: 0.099676\\ &  &  &  & 5x5deconv,2,3 & Kodak 4: 0.096410\\ &  &  &  &  & Kodak 5: 0.107615\\ &  &  &  &  & Kodak 6: 0.093928\\ &  &  &  &  & Kodak 7: 0.100785\\ &  &  &  &  & Kodak 8: 0.094832\\ &  &  &  &  & Kodak 9: 0.093807\\ &  &  &  &  & Kodak 10: 0.094529\\ &  &  &  &  & Kodak 11: 0.102641\\ &  &  &  &  & Kodak 12: 0.094292\\ &  &  &  &  & Kodak 13: 0.100835\\ &  &  &  &  & Kodak 14: 0.098764\\ &  &  &  &  & Kodak 15: 0.095786\\ &  &  &  &  & Kodak 16: 0.094760\\ &  &  &  &  & Kodak 17: 0.096186\\ &  &  &  &  & Kodak 18: 0.096750\\ &  &  &  &  & Kodak 19: 0.102512\\ &  &  &  &  & Kodak 20: 0.094453\\ &  &  &  &  & Kodak 21: 0.093890\\ &  &  &  &  & Kodak 22: 0.102659\\ &  &  &  &  & Kodak 23: 0.092862\\ &  &  &  &  & Kodak 24: 0.094941\\\hline\hline125 & MS-SSIM & 8.0 & 5x5deconv,2,10 & 5x5deconv,2,1 & Kodak 1: 0.099332\\ &  &  & 5x5deconv,2,10 & 5x5deconv,2,1 & Kodak 2: 0.095398\\ &  &  & 5x5deconv,2,320 & 5x5deconv,2,1 & Kodak 3: 0.095682\\ &  &  &  & 5x5deconv,2,3 & Kodak 4: 0.095641\\ &  &  &  &  & Kodak 5: 0.094915\\ &  &  &  &  & Kodak 6: 0.096150\\ &  &  &  &  & Kodak 7: 0.109551\\ &  &  &  &  & Kodak 8: 0.096224\\ &  &  &  &  & Kodak 9: 0.098993\\ &  &  &  &  & Kodak 10: 0.096190\\ &  &  &  &  & Kodak 11: 0.104167\\ &  &  &  &  & Kodak 12: 0.098927\\ &  &  &  &  & Kodak 13: 0.099872\\ &  &  &  &  & Kodak 14: 0.098283\\ &  &  &  &  & Kodak 15: 0.099330\\ &  &  &  &  & Kodak 16: 0.095996\\ &  &  &  &  & Kodak 17: 0.097298\\ &  &  &  &  & Kodak 18: 0.096642\\ &  &  &  &  & Kodak 19: 0.098590\\ &  &  &  &  & Kodak 20: 0.100411\\ &  &  &  &  & Kodak 21: 0.098178\\ &  &  &  &  & Kodak 22: 0.094602\\ &  &  &  &  & Kodak 23: 0.093866\\ &  &  &  &  & Kodak 24: 0.094619\\\hline\hline126 & MS-SSIM & 8.0 & 5x5deconv,2,10 & 5x5deconv,2,1 & Kodak 1: 0.096213\\ &  &  & 5x5deconv,2,10 & 5x5deconv,2,6 & Kodak 2: 0.101260\\ &  &  & 5x5deconv,2,320 & 5x5deconv,2,1 & Kodak 3: 0.096541\\ &  &  &  & 5x5deconv,2,3 & Kodak 4: 0.095421\\ &  &  &  &  & Kodak 5: 0.098241\\ &  &  &  &  & Kodak 6: 0.094703\\ &  &  &  &  & Kodak 7: 0.099120\\ &  &  &  &  & Kodak 8: 0.111118\\ &  &  &  &  & Kodak 9: 0.103598\\ &  &  &  &  & Kodak 10: 0.098047\\ &  &  &  &  & Kodak 11: 0.103634\\ &  &  &  &  & Kodak 12: 0.101910\\ &  &  &  &  & Kodak 13: 0.097769\\ &  &  &  &  & Kodak 14: 0.095701\\ &  &  &  &  & Kodak 15: 0.095421\\ &  &  &  &  & Kodak 16: 0.098352\\ &  &  &  &  & Kodak 17: 0.093238\\ &  &  &  &  & Kodak 18: 0.094530\\ &  &  &  &  & Kodak 19: 0.096709\\ &  &  &  &  & Kodak 20: 0.099939\\ &  &  &  &  & Kodak 21: 0.093040\\ &  &  &  &  & Kodak 22: 0.096550\\ &  &  &  &  & Kodak 23: 0.095337\\ &  &  &  &  & Kodak 24: 0.106908\\\hline\hline127 & MS-SSIM & 8.0 & 5x5deconv,2,21 & 5x5deconv,2,45 & Kodak 1: 0.122247\\ &  &  & 5x5deconv,2,32 & 5x5deconv,2,32 & Kodak 2: 0.121652\\ &  &  & 5x5deconv,2,320 & 5x5deconv,2,12 & Kodak 3: 0.111481\\ &  &  &  & 5x5deconv,2,3 & Kodak 4: 0.114946\\ &  &  &  &  & Kodak 5: 0.119622\\ &  &  &  &  & Kodak 6: 0.117467\\ &  &  &  &  & Kodak 7: 0.117495\\ &  &  &  &  & Kodak 8: 0.120984\\ &  &  &  &  & Kodak 9: 0.108773\\ &  &  &  &  & Kodak 10: 0.120018\\ &  &  &  &  & Kodak 11: 0.118537\\ &  &  &  &  & Kodak 12: 0.116371\\ &  &  &  &  & Kodak 13: 0.113775\\ &  &  &  &  & Kodak 14: 0.120392\\ &  &  &  &  & Kodak 15: 0.114809\\ &  &  &  &  & Kodak 16: 0.113567\\ &  &  &  &  & Kodak 17: 0.117508\\ &  &  &  &  & Kodak 18: 0.121690\\ &  &  &  &  & Kodak 19: 0.111937\\ &  &  &  &  & Kodak 20: 0.119967\\ &  &  &  &  & Kodak 21: 0.112400\\ &  &  &  &  & Kodak 22: 0.127661\\ &  &  &  &  & Kodak 23: 0.116331\\ &  &  &  &  & Kodak 24: 0.117562\\\hline\hline128 & MS-SSIM & 8.0 & 5x5deconv,2,10 & 5x5deconv,2,1 & Kodak 1: 0.097209\\ &  &  & 5x5deconv,2,10 & 5x5deconv,2,1 & Kodak 2: 0.093602\\ &  &  & 5x5deconv,2,320 & 5x5deconv,2,1 & Kodak 3: 0.099510\\ &  &  &  & 5x5deconv,2,3 & Kodak 4: 0.095567\\ &  &  &  &  & Kodak 5: 0.095302\\ &  &  &  &  & Kodak 6: 0.098875\\ &  &  &  &  & Kodak 7: 0.096205\\ &  &  &  &  & Kodak 8: 0.095630\\ &  &  &  &  & Kodak 9: 0.097337\\ &  &  &  &  & Kodak 10: 0.094469\\ &  &  &  &  & Kodak 11: 0.096736\\ &  &  &  &  & Kodak 12: 0.102180\\ &  &  &  &  & Kodak 13: 0.094882\\ &  &  &  &  & Kodak 14: 0.094325\\ &  &  &  &  & Kodak 15: 0.095428\\ &  &  &  &  & Kodak 16: 0.096963\\ &  &  &  &  & Kodak 17: 0.103464\\ &  &  &  &  & Kodak 18: 0.094748\\ &  &  &  &  & Kodak 19: 0.094963\\ &  &  &  &  & Kodak 20: 0.104983\\ &  &  &  &  & Kodak 21: 0.099904\\ &  &  &  &  & Kodak 22: 0.094663\\ &  &  &  &  & Kodak 23: 0.094345\\ &  &  &  &  & Kodak 24: 0.098879\\\hline\hline129 & MS-SSIM & 8.0 & 5x5deconv,2,150 & 5x5deconv,2,252 & Kodak 1: 0.262211\\ &  &  & 5x5deconv,2,183 & 5x5deconv,2,179 & Kodak 2: 0.249235\\ &  &  & 5x5deconv,2,320 & 5x5deconv,2,160 & Kodak 3: 0.252041\\ &  &  &  & 5x5deconv,2,3 & Kodak 4: 0.257887\\ &  &  &  &  & Kodak 5: 0.252972\\ &  &  &  &  & Kodak 6: 0.254682\\ &  &  &  &  & Kodak 7: 0.248569\\ &  &  &  &  & Kodak 8: 0.254664\\ &  &  &  &  & Kodak 9: 0.249629\\ &  &  &  &  & Kodak 10: 0.253500\\ &  &  &  &  & Kodak 11: 0.251628\\ &  &  &  &  & Kodak 12: 0.265711\\ &  &  &  &  & Kodak 13: 0.254219\\ &  &  &  &  & Kodak 14: 0.262398\\ &  &  &  &  & Kodak 15: 0.252378\\ &  &  &  &  & Kodak 16: 0.251702\\ &  &  &  &  & Kodak 17: 0.253058\\ &  &  &  &  & Kodak 18: 0.257231\\ &  &  &  &  & Kodak 19: 0.252141\\ &  &  &  &  & Kodak 20: 0.250581\\ &  &  &  &  & Kodak 21: 0.247138\\ &  &  &  &  & Kodak 22: 0.253130\\ &  &  &  &  & Kodak 23: 0.259897\\ &  &  &  &  & Kodak 24: 0.252696\\\hline\hline130 & MSE & 0.1 & 5x5deconv,2,10 & 5x5deconv,2,1 & Kodak 1: 0.090429\\ &  &  & 5x5deconv,2,10 & 5x5deconv,2,10 & Kodak 2: 0.099224\\ &  &  & 5x5deconv,2,320 & 5x5deconv,2,1 & Kodak 3: 0.094465\\ &  &  &  & 5x5deconv,2,3 & Kodak 4: 0.097336\\ &  &  &  &  & Kodak 5: 0.096487\\ &  &  &  &  & Kodak 6: 0.095787\\ &  &  &  &  & Kodak 7: 0.095523\\ &  &  &  &  & Kodak 8: 0.098076\\ &  &  &  &  & Kodak 9: 0.102374\\ &  &  &  &  & Kodak 10: 0.097467\\ &  &  &  &  & Kodak 11: 0.100785\\ &  &  &  &  & Kodak 12: 0.097448\\ &  &  &  &  & Kodak 13: 0.100138\\ &  &  &  &  & Kodak 14: 0.097043\\ &  &  &  &  & Kodak 15: 0.097858\\ &  &  &  &  & Kodak 16: 0.097672\\ &  &  &  &  & Kodak 17: 0.096753\\ &  &  &  &  & Kodak 18: 0.095807\\ &  &  &  &  & Kodak 19: 0.101102\\ &  &  &  &  & Kodak 20: 0.095769\\ &  &  &  &  & Kodak 21: 0.100900\\ &  &  &  &  & Kodak 22: 0.100592\\ &  &  &  &  & Kodak 23: 0.098168\\ &  &  &  &  & Kodak 24: 0.093999\\\hline\hline131 & MSE & 0.1 & 5x5deconv,2,26 & 5x5deconv,2,317 & Kodak 1: 0.253992\\ &  &  & 5x5deconv,2,26 & 5x5deconv,2,318 & Kodak 2: 0.252061\\ &  &  & 5x5deconv,2,320 & 5x5deconv,2,62 & Kodak 3: 0.246699\\ &  &  &  & 5x5deconv,2,3 & Kodak 4: 0.243999\\ &  &  &  &  & Kodak 5: 0.244742\\ &  &  &  &  & Kodak 6: 0.252538\\ &  &  &  &  & Kodak 7: 0.241884\\ &  &  &  &  & Kodak 8: 0.253047\\ &  &  &  &  & Kodak 9: 0.241561\\ &  &  &  &  & Kodak 10: 0.257844\\ &  &  &  &  & Kodak 11: 0.244629\\ &  &  &  &  & Kodak 12: 0.249970\\ &  &  &  &  & Kodak 13: 0.254374\\ &  &  &  &  & Kodak 14: 0.246358\\ &  &  &  &  & Kodak 15: 0.251292\\ &  &  &  &  & Kodak 16: 0.249967\\ &  &  &  &  & Kodak 17: 0.247014\\ &  &  &  &  & Kodak 18: 0.248629\\ &  &  &  &  & Kodak 19: 0.248225\\ &  &  &  &  & Kodak 20: 0.251812\\ &  &  &  &  & Kodak 21: 0.243724\\ &  &  &  &  & Kodak 22: 0.249720\\ &  &  &  &  & Kodak 23: 0.246120\\ &  &  &  &  & Kodak 24: 0.248593\\\hline\hline132 & MSE & 0.1 & 5x5deconv,2,10 & 5x5deconv,2,1 & Kodak 1: 0.089036\\ &  &  & 5x5deconv,2,10 & 5x5deconv,2,9 & Kodak 2: 0.097550\\ &  &  & 5x5deconv,2,320 & 5x5deconv,2,1 & Kodak 3: 0.100783\\ &  &  &  & 5x5deconv,2,3 & Kodak 4: 0.094312\\ &  &  &  &  & Kodak 5: 0.098428\\ &  &  &  &  & Kodak 6: 0.099175\\ &  &  &  &  & Kodak 7: 0.094759\\ &  &  &  &  & Kodak 8: 0.098884\\ &  &  &  &  & Kodak 9: 0.101784\\ &  &  &  &  & Kodak 10: 0.098242\\ &  &  &  &  & Kodak 11: 0.100850\\ &  &  &  &  & Kodak 12: 0.098983\\ &  &  &  &  & Kodak 13: 0.093770\\ &  &  &  &  & Kodak 14: 0.095750\\ &  &  &  &  & Kodak 15: 0.093982\\ &  &  &  &  & Kodak 16: 0.097815\\ &  &  &  &  & Kodak 17: 0.100647\\ &  &  &  &  & Kodak 18: 0.099836\\ &  &  &  &  & Kodak 19: 0.098002\\ &  &  &  &  & Kodak 20: 0.100289\\ &  &  &  &  & Kodak 21: 0.099873\\ &  &  &  &  & Kodak 22: 0.096005\\ &  &  &  &  & Kodak 23: 0.094975\\ &  &  &  &  & Kodak 24: 0.095375\\\hline\hline133 & MSE & 0.1 & 5x5deconv,2,121 & 5x5deconv,2,320 & Kodak 1: 0.481659\\ &  &  & 5x5deconv,2,344 & 5x5deconv,2,320 & Kodak 2: 0.468366\\ &  &  & 5x5deconv,2,320 & 5x5deconv,2,320 & Kodak 3: 0.468255\\ &  &  &  & 5x5deconv,2,3 & Kodak 4: 0.469708\\ &  &  &  &  & Kodak 5: 0.475139\\ &  &  &  &  & Kodak 6: 0.460072\\ &  &  &  &  & Kodak 7: 0.469157\\ &  &  &  &  & Kodak 8: 0.470979\\ &  &  &  &  & Kodak 9: 0.467544\\ &  &  &  &  & Kodak 10: 0.467709\\ &  &  &  &  & Kodak 11: 0.474068\\ &  &  &  &  & Kodak 12: 0.479579\\ &  &  &  &  & Kodak 13: 0.476754\\ &  &  &  &  & Kodak 14: 0.472240\\ &  &  &  &  & Kodak 15: 0.471871\\ &  &  &  &  & Kodak 16: 0.466201\\ &  &  &  &  & Kodak 17: 0.468905\\ &  &  &  &  & Kodak 18: 0.477990\\ &  &  &  &  & Kodak 19: 0.469902\\ &  &  &  &  & Kodak 20: 0.461492\\ &  &  &  &  & Kodak 21: 0.468919\\ &  &  &  &  & Kodak 22: 0.469018\\ &  &  &  &  & Kodak 23: 0.463560\\ &  &  &  &  & Kodak 24: 0.484876\\\hline\hline134 & MSE & 0.1 & 5x5deconv,2,7 & 5x5deconv,2,130 & Kodak 1: 0.142532\\ &  &  & 5x5deconv,2,13 & 5x5deconv,2,35 & Kodak 2: 0.125605\\ &  &  & 5x5deconv,2,320 & 5x5deconv,2,15 & Kodak 3: 0.119145\\ &  &  &  & 5x5deconv,2,3 & Kodak 4: 0.129092\\ &  &  &  &  & Kodak 5: 0.139332\\ &  &  &  &  & Kodak 6: 0.126292\\ &  &  &  &  & Kodak 7: 0.120804\\ &  &  &  &  & Kodak 8: 0.132543\\ &  &  &  &  & Kodak 9: 0.121592\\ &  &  &  &  & Kodak 10: 0.115401\\ &  &  &  &  & Kodak 11: 0.130864\\ &  &  &  &  & Kodak 12: 0.124881\\ &  &  &  &  & Kodak 13: 0.134268\\ &  &  &  &  & Kodak 14: 0.126354\\ &  &  &  &  & Kodak 15: 0.118809\\ &  &  &  &  & Kodak 16: 0.125791\\ &  &  &  &  & Kodak 17: 0.125338\\ &  &  &  &  & Kodak 18: 0.130828\\ &  &  &  &  & Kodak 19: 0.131055\\ &  &  &  &  & Kodak 20: 0.126076\\ &  &  &  &  & Kodak 21: 0.130086\\ &  &  &  &  & Kodak 22: 0.123319\\ &  &  &  &  & Kodak 23: 0.124586\\ &  &  &  &  & Kodak 24: 0.126732\\\hline\hline135 & MSE & 0.1 & 5x5deconv,2,10 & 5x5deconv,2,1 & Kodak 1: 0.092333\\ &  &  & 5x5deconv,2,10 & 5x5deconv,2,5 & Kodak 2: 0.101986\\ &  &  & 5x5deconv,2,320 & 5x5deconv,2,1 & Kodak 3: 0.098592\\ &  &  &  & 5x5deconv,2,3 & Kodak 4: 0.100899\\ &  &  &  &  & Kodak 5: 0.094209\\ &  &  &  &  & Kodak 6: 0.100880\\ &  &  &  &  & Kodak 7: 0.096998\\ &  &  &  &  & Kodak 8: 0.099688\\ &  &  &  &  & Kodak 9: 0.095160\\ &  &  &  &  & Kodak 10: 0.094753\\ &  &  &  &  & Kodak 11: 0.097111\\ &  &  &  &  & Kodak 12: 0.110651\\ &  &  &  &  & Kodak 13: 0.100626\\ &  &  &  &  & Kodak 14: 0.101754\\ &  &  &  &  & Kodak 15: 0.097753\\ &  &  &  &  & Kodak 16: 0.100781\\ &  &  &  &  & Kodak 17: 0.096788\\ &  &  &  &  & Kodak 18: 0.098507\\ &  &  &  &  & Kodak 19: 0.098709\\ &  &  &  &  & Kodak 20: 0.095960\\ &  &  &  &  & Kodak 21: 0.099527\\ &  &  &  &  & Kodak 22: 0.098687\\ &  &  &  &  & Kodak 23: 0.106527\\ &  &  &  &  & Kodak 24: 0.099025\\\hline\hline136 & MSE & 0.1 & 5x5deconv,2,4 & 5x5deconv,2,15 & Kodak 1: 0.106560\\ &  &  & 5x5deconv,2,3 & 5x5deconv,2,13 & Kodak 2: 0.106990\\ &  &  & 5x5deconv,2,320 & 5x5deconv,2,6 & Kodak 3: 0.103098\\ &  &  &  & 5x5deconv,2,3 & Kodak 4: 0.108392\\ &  &  &  &  & Kodak 5: 0.116674\\ &  &  &  &  & Kodak 6: 0.107274\\ &  &  &  &  & Kodak 7: 0.116851\\ &  &  &  &  & Kodak 8: 0.112565\\ &  &  &  &  & Kodak 9: 0.113003\\ &  &  &  &  & Kodak 10: 0.101842\\ &  &  &  &  & Kodak 11: 0.102050\\ &  &  &  &  & Kodak 12: 0.105474\\ &  &  &  &  & Kodak 13: 0.107104\\ &  &  &  &  & Kodak 14: 0.104093\\ &  &  &  &  & Kodak 15: 0.137977\\ &  &  &  &  & Kodak 16: 0.118926\\ &  &  &  &  & Kodak 17: 0.123728\\ &  &  &  &  & Kodak 18: 0.124440\\ &  &  &  &  & Kodak 19: 0.128604\\ &  &  &  &  & Kodak 20: 0.117889\\ &  &  &  &  & Kodak 21: 0.116582\\ &  &  &  &  & Kodak 22: 0.105249\\ &  &  &  &  & Kodak 23: 0.107015\\ &  &  &  &  & Kodak 24: 0.117414\\\hline\hline137 & MSE & 0.1 & 5x5deconv,2,97 & 5x5deconv,2,304 & Kodak 1: 0.219113\\ &  &  & 5x5deconv,2,116 & 5x5deconv,2,92 & Kodak 2: 0.216052\\ &  &  & 5x5deconv,2,320 & 5x5deconv,2,140 & Kodak 3: 0.211310\\ &  &  &  & 5x5deconv,2,3 & Kodak 4: 0.214075\\ &  &  &  &  & Kodak 5: 0.220980\\ &  &  &  &  & Kodak 6: 0.212966\\ &  &  &  &  & Kodak 7: 0.213109\\ &  &  &  &  & Kodak 8: 0.214546\\ &  &  &  &  & Kodak 9: 0.223940\\ &  &  &  &  & Kodak 10: 0.214416\\ &  &  &  &  & Kodak 11: 0.217510\\ &  &  &  &  & Kodak 12: 0.221753\\ &  &  &  &  & Kodak 13: 0.216600\\ &  &  &  &  & Kodak 14: 0.212461\\ &  &  &  &  & Kodak 15: 0.225300\\ &  &  &  &  & Kodak 16: 0.210901\\ &  &  &  &  & Kodak 17: 0.218437\\ &  &  &  &  & Kodak 18: 0.218093\\ &  &  &  &  & Kodak 19: 0.224472\\ &  &  &  &  & Kodak 20: 0.217115\\ &  &  &  &  & Kodak 21: 0.223558\\ &  &  &  &  & Kodak 22: 0.212603\\ &  &  &  &  & Kodak 23: 0.225525\\ &  &  &  &  & Kodak 24: 0.216879\\\hline\hline138 & MSE & 0.1 & 5x5deconv,2,17 & 5x5deconv,2,41 & Kodak 1: 0.121429\\ &  &  & 5x5deconv,2,29 & 5x5deconv,2,23 & Kodak 2: 0.112793\\ &  &  & 5x5deconv,2,320 & 5x5deconv,2,10 & Kodak 3: 0.116799\\ &  &  &  & 5x5deconv,2,3 & Kodak 4: 0.116365\\ &  &  &  &  & Kodak 5: 0.125837\\ &  &  &  &  & Kodak 6: 0.129252\\ &  &  &  &  & Kodak 7: 0.116164\\ &  &  &  &  & Kodak 8: 0.119049\\ &  &  &  &  & Kodak 9: 0.120701\\ &  &  &  &  & Kodak 10: 0.107731\\ &  &  &  &  & Kodak 11: 0.110532\\ &  &  &  &  & Kodak 12: 0.113739\\ &  &  &  &  & Kodak 13: 0.118284\\ &  &  &  &  & Kodak 14: 0.121054\\ &  &  &  &  & Kodak 15: 0.113387\\ &  &  &  &  & Kodak 16: 0.120243\\ &  &  &  &  & Kodak 17: 0.116478\\ &  &  &  &  & Kodak 18: 0.119829\\ &  &  &  &  & Kodak 19: 0.121194\\ &  &  &  &  & Kodak 20: 0.115347\\ &  &  &  &  & Kodak 21: 0.117505\\ &  &  &  &  & Kodak 22: 0.107815\\ &  &  &  &  & Kodak 23: 0.113049\\ &  &  &  &  & Kodak 24: 0.117995\\\hline\hline139 & MSE & 0.1 & 5x5deconv,2,97 & 5x5deconv,2,320 & Kodak 1: 0.479663\\ &  &  & 5x5deconv,2,63 & 5x5deconv,2,320 & Kodak 2: 0.456830\\ &  &  & 5x5deconv,2,320 & 5x5deconv,2,320 & Kodak 3: 0.462371\\ &  &  &  & 5x5deconv,2,3 & Kodak 4: 0.469212\\ &  &  &  &  & Kodak 5: 0.471877\\ &  &  &  &  & Kodak 6: 0.462212\\ &  &  &  &  & Kodak 7: 0.500694\\ &  &  &  &  & Kodak 8: 0.470778\\ &  &  &  &  & Kodak 9: 0.461106\\ &  &  &  &  & Kodak 10: 0.460153\\ &  &  &  &  & Kodak 11: 0.471040\\ &  &  &  &  & Kodak 12: 0.467536\\ &  &  &  &  & Kodak 13: 0.467321\\ &  &  &  &  & Kodak 14: 0.471187\\ &  &  &  &  & Kodak 15: 0.464505\\ &  &  &  &  & Kodak 16: 0.465739\\ &  &  &  &  & Kodak 17: 0.469104\\ &  &  &  &  & Kodak 18: 0.468796\\ &  &  &  &  & Kodak 19: 0.468807\\ &  &  &  &  & Kodak 20: 0.468936\\ &  &  &  &  & Kodak 21: 0.466779\\ &  &  &  &  & Kodak 22: 0.481170\\ &  &  &  &  & Kodak 23: 0.473404\\ &  &  &  &  & Kodak 24: 0.466344\\\hline\hline140 & MSE & 0.1 & 5x5deconv,2,142 & 5x5deconv,2,320 & Kodak 1: 0.479931\\ &  &  & 5x5deconv,2,405 & 5x5deconv,2,320 & Kodak 2: 0.467517\\ &  &  & 5x5deconv,2,320 & 5x5deconv,2,320 & Kodak 3: 0.467453\\ &  &  &  & 5x5deconv,2,3 & Kodak 4: 0.478378\\ &  &  &  &  & Kodak 5: 0.464479\\ &  &  &  &  & Kodak 6: 0.465645\\ &  &  &  &  & Kodak 7: 0.459733\\ &  &  &  &  & Kodak 8: 0.470914\\ &  &  &  &  & Kodak 9: 0.459690\\ &  &  &  &  & Kodak 10: 0.459046\\ &  &  &  &  & Kodak 11: 0.461381\\ &  &  &  &  & Kodak 12: 0.466622\\ &  &  &  &  & Kodak 13: 0.467599\\ &  &  &  &  & Kodak 14: 0.471110\\ &  &  &  &  & Kodak 15: 0.460103\\ &  &  &  &  & Kodak 16: 0.467493\\ &  &  &  &  & Kodak 17: 0.461306\\ &  &  &  &  & Kodak 18: 0.468145\\ &  &  &  &  & Kodak 19: 0.468512\\ &  &  &  &  & Kodak 20: 0.460920\\ &  &  &  &  & Kodak 21: 0.467536\\ &  &  &  &  & Kodak 22: 0.471034\\ &  &  &  &  & Kodak 23: 0.469735\\ &  &  &  &  & Kodak 24: 0.464966\\\hline\hline141 & MSE & 0.1 & 5x5deconv,2,110 & 5x5deconv,2,320 & Kodak 1: 0.372799\\ &  &  & 5x5deconv,2,310 & 5x5deconv,2,176 & Kodak 2: 0.362586\\ &  &  & 5x5deconv,2,320 & 5x5deconv,2,304 & Kodak 3: 0.358868\\ &  &  &  & 5x5deconv,2,3 & Kodak 4: 0.390599\\ &  &  &  &  & Kodak 5: 0.366360\\ &  &  &  &  & Kodak 6: 0.358812\\ &  &  &  &  & Kodak 7: 0.361179\\ &  &  &  &  & Kodak 8: 0.366796\\ &  &  &  &  & Kodak 9: 0.359760\\ &  &  &  &  & Kodak 10: 0.356888\\ &  &  &  &  & Kodak 11: 0.389857\\ &  &  &  &  & Kodak 12: 0.362880\\ &  &  &  &  & Kodak 13: 0.374729\\ &  &  &  &  & Kodak 14: 0.367973\\ &  &  &  &  & Kodak 15: 0.362475\\ &  &  &  &  & Kodak 16: 0.365911\\ &  &  &  &  & Kodak 17: 0.360376\\ &  &  &  &  & Kodak 18: 0.359489\\ &  &  &  &  & Kodak 19: 0.357965\\ &  &  &  &  & Kodak 20: 0.365797\\ &  &  &  &  & Kodak 21: 0.364752\\ &  &  &  &  & Kodak 22: 0.362062\\ &  &  &  &  & Kodak 23: 0.392338\\ &  &  &  &  & Kodak 24: 0.361389\\\hline\hline142 & MSE & 0.1 & 5x5deconv,2,137 & 5x5deconv,2,320 & Kodak 1: 0.480384\\ &  &  & 5x5deconv,2,168 & 5x5deconv,2,320 & Kodak 2: 0.469157\\ &  &  & 5x5deconv,2,320 & 5x5deconv,2,320 & Kodak 3: 0.468652\\ &  &  &  & 5x5deconv,2,3 & Kodak 4: 0.484393\\ &  &  &  &  & Kodak 5: 0.470108\\ &  &  &  &  & Kodak 6: 0.477917\\ &  &  &  &  & Kodak 7: 0.475554\\ &  &  &  &  & Kodak 8: 0.466667\\ &  &  &  &  & Kodak 9: 0.463783\\ &  &  &  &  & Kodak 10: 0.465310\\ &  &  &  &  & Kodak 11: 0.460835\\ &  &  &  &  & Kodak 12: 0.466972\\ &  &  &  &  & Kodak 13: 0.473992\\ &  &  &  &  & Kodak 14: 0.465868\\ &  &  &  &  & Kodak 15: 0.462942\\ &  &  &  &  & Kodak 16: 0.469657\\ &  &  &  &  & Kodak 17: 0.466100\\ &  &  &  &  & Kodak 18: 0.468792\\ &  &  &  &  & Kodak 19: 0.466899\\ &  &  &  &  & Kodak 20: 0.485336\\ &  &  &  &  & Kodak 21: 0.468973\\ &  &  &  &  & Kodak 22: 0.464597\\ &  &  &  &  & Kodak 23: 0.464765\\ &  &  &  &  & Kodak 24: 0.466055\\\hline\hline143 & MSE & 0.1 & 5x5deconv,2,10 & 5x5deconv,2,1 & Kodak 1: 0.101335\\ &  &  & 5x5deconv,2,10 & 5x5deconv,2,9 & Kodak 2: 0.100469\\ &  &  & 5x5deconv,2,320 & 5x5deconv,2,1 & Kodak 3: 0.099128\\ &  &  &  & 5x5deconv,2,3 & Kodak 4: 0.095875\\ &  &  &  &  & Kodak 5: 0.096948\\ &  &  &  &  & Kodak 6: 0.095268\\ &  &  &  &  & Kodak 7: 0.104205\\ &  &  &  &  & Kodak 8: 0.104376\\ &  &  &  &  & Kodak 9: 0.093939\\ &  &  &  &  & Kodak 10: 0.100787\\ &  &  &  &  & Kodak 11: 0.100907\\ &  &  &  &  & Kodak 12: 0.102626\\ &  &  &  &  & Kodak 13: 0.095098\\ &  &  &  &  & Kodak 14: 0.098307\\ &  &  &  &  & Kodak 15: 0.102045\\ &  &  &  &  & Kodak 16: 0.096350\\ &  &  &  &  & Kodak 17: 0.100804\\ &  &  &  &  & Kodak 18: 0.097760\\ &  &  &  &  & Kodak 19: 0.099925\\ &  &  &  &  & Kodak 20: 0.095979\\ &  &  &  &  & Kodak 21: 0.099067\\ &  &  &  &  & Kodak 22: 0.097847\\ &  &  &  &  & Kodak 23: 0.096015\\ &  &  &  &  & Kodak 24: 0.093131\\\hline\hline144 & MSE & 0.1 & 5x5deconv,2,162 & 5x5deconv,2,320 & Kodak 1: 0.310731\\ &  &  & 5x5deconv,2,238 & 5x5deconv,2,178 & Kodak 2: 0.303398\\ &  &  & 5x5deconv,2,320 & 5x5deconv,2,223 & Kodak 3: 0.299126\\ &  &  &  & 5x5deconv,2,3 & Kodak 4: 0.317278\\ &  &  &  &  & Kodak 5: 0.308188\\ &  &  &  &  & Kodak 6: 0.301917\\ &  &  &  &  & Kodak 7: 0.303779\\ &  &  &  &  & Kodak 8: 0.301094\\ &  &  &  &  & Kodak 9: 0.304472\\ &  &  &  &  & Kodak 10: 0.297055\\ &  &  &  &  & Kodak 11: 0.299686\\ &  &  &  &  & Kodak 12: 0.297032\\ &  &  &  &  & Kodak 13: 0.314949\\ &  &  &  &  & Kodak 14: 0.302654\\ &  &  &  &  & Kodak 15: 0.299089\\ &  &  &  &  & Kodak 16: 0.306094\\ &  &  &  &  & Kodak 17: 0.307862\\ &  &  &  &  & Kodak 18: 0.299928\\ &  &  &  &  & Kodak 19: 0.311035\\ &  &  &  &  & Kodak 20: 0.304814\\ &  &  &  &  & Kodak 21: 0.303327\\ &  &  &  &  & Kodak 22: 0.306639\\ &  &  &  &  & Kodak 23: 0.298914\\ &  &  &  &  & Kodak 24: 0.300823\\\hline\hline145 & MSE & 0.2 & 5x5deconv,2,166 & 5x5deconv,2,320 & Kodak 1: 0.303118\\ &  &  & 5x5deconv,2,197 & 5x5deconv,2,140 & Kodak 2: 0.294212\\ &  &  & 5x5deconv,2,320 & 5x5deconv,2,233 & Kodak 3: 0.294831\\ &  &  &  & 5x5deconv,2,3 & Kodak 4: 0.295587\\ &  &  &  &  & Kodak 5: 0.292993\\ &  &  &  &  & Kodak 6: 0.295411\\ &  &  &  &  & Kodak 7: 0.294374\\ &  &  &  &  & Kodak 8: 0.306506\\ &  &  &  &  & Kodak 9: 0.313997\\ &  &  &  &  & Kodak 10: 0.294935\\ &  &  &  &  & Kodak 11: 0.302208\\ &  &  &  &  & Kodak 12: 0.293460\\ &  &  &  &  & Kodak 13: 0.312676\\ &  &  &  &  & Kodak 14: 0.300582\\ &  &  &  &  & Kodak 15: 0.291714\\ &  &  &  &  & Kodak 16: 0.295152\\ &  &  &  &  & Kodak 17: 0.313638\\ &  &  &  &  & Kodak 18: 0.299121\\ &  &  &  &  & Kodak 19: 0.293951\\ &  &  &  &  & Kodak 20: 0.293809\\ &  &  &  &  & Kodak 21: 0.297381\\ &  &  &  &  & Kodak 22: 0.300699\\ &  &  &  &  & Kodak 23: 0.291845\\ &  &  &  &  & Kodak 24: 0.294100\\\hline\hline146 & MSE & 0.2 & 5x5deconv,2,160 & 5x5deconv,2,320 & Kodak 1: 0.301528\\ &  &  & 5x5deconv,2,253 & 5x5deconv,2,155 & Kodak 2: 0.295704\\ &  &  & 5x5deconv,2,320 & 5x5deconv,2,227 & Kodak 3: 0.293139\\ &  &  &  & 5x5deconv,2,3 & Kodak 4: 0.289731\\ &  &  &  &  & Kodak 5: 0.295430\\ &  &  &  &  & Kodak 6: 0.297240\\ &  &  &  &  & Kodak 7: 0.295715\\ &  &  &  &  & Kodak 8: 0.298541\\ &  &  &  &  & Kodak 9: 0.290056\\ &  &  &  &  & Kodak 10: 0.294261\\ &  &  &  &  & Kodak 11: 0.295399\\ &  &  &  &  & Kodak 12: 0.309540\\ &  &  &  &  & Kodak 13: 0.299799\\ &  &  &  &  & Kodak 14: 0.295456\\ &  &  &  &  & Kodak 15: 0.294643\\ &  &  &  &  & Kodak 16: 0.298482\\ &  &  &  &  & Kodak 17: 0.290810\\ &  &  &  &  & Kodak 18: 0.296871\\ &  &  &  &  & Kodak 19: 0.311163\\ &  &  &  &  & Kodak 20: 0.293156\\ &  &  &  &  & Kodak 21: 0.296664\\ &  &  &  &  & Kodak 22: 0.297960\\ &  &  &  &  & Kodak 23: 0.293464\\ &  &  &  &  & Kodak 24: 0.298733\\\hline\hline147 & MSE & 0.2 & 5x5deconv,2,4 & 5x5deconv,2,21 & Kodak 1: 0.105709\\ &  &  & 5x5deconv,2,4 & 5x5deconv,2,12 & Kodak 2: 0.103841\\ &  &  & 5x5deconv,2,320 & 5x5deconv,2,6 & Kodak 3: 0.105526\\ &  &  &  & 5x5deconv,2,3 & Kodak 4: 0.108750\\ &  &  &  &  & Kodak 5: 0.109773\\ &  &  &  &  & Kodak 6: 0.106055\\ &  &  &  &  & Kodak 7: 0.111679\\ &  &  &  &  & Kodak 8: 0.113288\\ &  &  &  &  & Kodak 9: 0.102821\\ &  &  &  &  & Kodak 10: 0.111710\\ &  &  &  &  & Kodak 11: 0.113187\\ &  &  &  &  & Kodak 12: 0.107489\\ &  &  &  &  & Kodak 13: 0.110753\\ &  &  &  &  & Kodak 14: 0.117701\\ &  &  &  &  & Kodak 15: 0.111358\\ &  &  &  &  & Kodak 16: 0.107164\\ &  &  &  &  & Kodak 17: 0.101179\\ &  &  &  &  & Kodak 18: 0.105911\\ &  &  &  &  & Kodak 19: 0.107640\\ &  &  &  &  & Kodak 20: 0.102002\\ &  &  &  &  & Kodak 21: 0.109949\\ &  &  &  &  & Kodak 22: 0.109005\\ &  &  &  &  & Kodak 23: 0.098350\\ &  &  &  &  & Kodak 24: 0.107793\\\hline\hline148 & MSE & 0.2 & 5x5deconv,2,10 & 5x5deconv,2,4 & Kodak 1: 0.090605\\ &  &  & 5x5deconv,2,10 & 5x5deconv,2,9 & Kodak 2: 0.102694\\ &  &  & 5x5deconv,2,320 & 5x5deconv,2,1 & Kodak 3: 0.102146\\ &  &  &  & 5x5deconv,2,3 & Kodak 4: 0.099528\\ &  &  &  &  & Kodak 5: 0.105779\\ &  &  &  &  & Kodak 6: 0.098887\\ &  &  &  &  & Kodak 7: 0.098631\\ &  &  &  &  & Kodak 8: 0.096184\\ &  &  &  &  & Kodak 9: 0.102200\\ &  &  &  &  & Kodak 10: 0.101487\\ &  &  &  &  & Kodak 11: 0.101246\\ &  &  &  &  & Kodak 12: 0.101873\\ &  &  &  &  & Kodak 13: 0.101027\\ &  &  &  &  & Kodak 14: 0.098653\\ &  &  &  &  & Kodak 15: 0.095091\\ &  &  &  &  & Kodak 16: 0.105483\\ &  &  &  &  & Kodak 17: 0.105454\\ &  &  &  &  & Kodak 18: 0.105141\\ &  &  &  &  & Kodak 19: 0.097336\\ &  &  &  &  & Kodak 20: 0.104404\\ &  &  &  &  & Kodak 21: 0.103096\\ &  &  &  &  & Kodak 22: 0.127719\\ &  &  &  &  & Kodak 23: 0.110119\\ &  &  &  &  & Kodak 24: 0.103548\\\hline\hline149 & MSE & 0.2 & 5x5deconv,2,162 & 5x5deconv,2,320 & Kodak 1: 0.481202\\ &  &  & 5x5deconv,2,149 & 5x5deconv,2,320 & Kodak 2: 0.463770\\ &  &  & 5x5deconv,2,320 & 5x5deconv,2,320 & Kodak 3: 0.481928\\ &  &  &  & 5x5deconv,2,3 & Kodak 4: 0.487866\\ &  &  &  &  & Kodak 5: 0.471976\\ &  &  &  &  & Kodak 6: 0.479604\\ &  &  &  &  & Kodak 7: 0.465093\\ &  &  &  &  & Kodak 8: 0.474560\\ &  &  &  &  & Kodak 9: 0.465092\\ &  &  &  &  & Kodak 10: 0.469526\\ &  &  &  &  & Kodak 11: 0.469809\\ &  &  &  &  & Kodak 12: 0.466042\\ &  &  &  &  & Kodak 13: 0.479955\\ &  &  &  &  & Kodak 14: 0.473695\\ &  &  &  &  & Kodak 15: 0.500995\\ &  &  &  &  & Kodak 16: 0.468231\\ &  &  &  &  & Kodak 17: 0.474178\\ &  &  &  &  & Kodak 18: 0.475303\\ &  &  &  &  & Kodak 19: 0.470313\\ &  &  &  &  & Kodak 20: 0.470276\\ &  &  &  &  & Kodak 21: 0.477627\\ &  &  &  &  & Kodak 22: 0.474138\\ &  &  &  &  & Kodak 23: 0.465759\\ &  &  &  &  & Kodak 24: 0.474751\\\hline\hline150 & MSE & 0.2 & 5x5deconv,2,10 & 5x5deconv,2,1 & Kodak 1: 0.092079\\ &  &  & 5x5deconv,2,10 & 5x5deconv,2,11 & Kodak 2: 0.099110\\ &  &  & 5x5deconv,2,320 & 5x5deconv,2,1 & Kodak 3: 0.097571\\ &  &  &  & 5x5deconv,2,3 & Kodak 4: 0.100326\\ &  &  &  &  & Kodak 5: 0.097477\\ &  &  &  &  & Kodak 6: 0.101978\\ &  &  &  &  & Kodak 7: 0.096702\\ &  &  &  &  & Kodak 8: 0.098425\\ &  &  &  &  & Kodak 9: 0.099220\\ &  &  &  &  & Kodak 10: 0.097570\\ &  &  &  &  & Kodak 11: 0.100229\\ &  &  &  &  & Kodak 12: 0.097656\\ &  &  &  &  & Kodak 13: 0.098198\\ &  &  &  &  & Kodak 14: 0.099117\\ &  &  &  &  & Kodak 15: 0.101997\\ &  &  &  &  & Kodak 16: 0.096896\\ &  &  &  &  & Kodak 17: 0.098294\\ &  &  &  &  & Kodak 18: 0.102178\\ &  &  &  &  & Kodak 19: 0.100865\\ &  &  &  &  & Kodak 20: 0.101818\\ &  &  &  &  & Kodak 21: 0.095364\\ &  &  &  &  & Kodak 22: 0.097354\\ &  &  &  &  & Kodak 23: 0.097263\\ &  &  &  &  & Kodak 24: 0.102214\\\hline\hline151 & MSE & 0.2 & 5x5deconv,2,10 & 5x5deconv,2,1 & Kodak 1: 0.098289\\ &  &  & 5x5deconv,2,10 & 5x5deconv,2,7 & Kodak 2: 0.099639\\ &  &  & 5x5deconv,2,320 & 5x5deconv,2,1 & Kodak 3: 0.097120\\ &  &  &  & 5x5deconv,2,3 & Kodak 4: 0.097980\\ &  &  &  &  & Kodak 5: 0.098229\\ &  &  &  &  & Kodak 6: 0.097569\\ &  &  &  &  & Kodak 7: 0.099217\\ &  &  &  &  & Kodak 8: 0.094511\\ &  &  &  &  & Kodak 9: 0.096500\\ &  &  &  &  & Kodak 10: 0.100274\\ &  &  &  &  & Kodak 11: 0.097966\\ &  &  &  &  & Kodak 12: 0.096745\\ &  &  &  &  & Kodak 13: 0.094998\\ &  &  &  &  & Kodak 14: 0.099842\\ &  &  &  &  & Kodak 15: 0.094576\\ &  &  &  &  & Kodak 16: 0.097489\\ &  &  &  &  & Kodak 17: 0.093672\\ &  &  &  &  & Kodak 18: 0.102305\\ &  &  &  &  & Kodak 19: 0.090897\\ &  &  &  &  & Kodak 20: 0.095420\\ &  &  &  &  & Kodak 21: 0.102069\\ &  &  &  &  & Kodak 22: 0.095531\\ &  &  &  &  & Kodak 23: 0.097753\\ &  &  &  &  & Kodak 24: 0.098305\\\hline\hline152 & MSE & 0.2 & 5x5deconv,2,155 & 5x5deconv,2,320 & Kodak 1: 0.489186\\ &  &  & 5x5deconv,2,419 & 5x5deconv,2,297 & Kodak 2: 0.470168\\ &  &  & 5x5deconv,2,320 & 5x5deconv,2,320 & Kodak 3: 0.464226\\ &  &  &  & 5x5deconv,2,3 & Kodak 4: 0.459460\\ &  &  &  &  & Kodak 5: 0.464071\\ &  &  &  &  & Kodak 6: 0.459052\\ &  &  &  &  & Kodak 7: 0.456941\\ &  &  &  &  & Kodak 8: 0.472730\\ &  &  &  &  & Kodak 9: 0.468377\\ &  &  &  &  & Kodak 10: 0.461921\\ &  &  &  &  & Kodak 11: 0.458854\\ &  &  &  &  & Kodak 12: 0.458204\\ &  &  &  &  & Kodak 13: 0.471632\\ &  &  &  &  & Kodak 14: 0.456648\\ &  &  &  &  & Kodak 15: 0.459306\\ &  &  &  &  & Kodak 16: 0.459673\\ &  &  &  &  & Kodak 17: 0.459775\\ &  &  &  &  & Kodak 18: 0.458965\\ &  &  &  &  & Kodak 19: 0.464847\\ &  &  &  &  & Kodak 20: 0.456721\\ &  &  &  &  & Kodak 21: 0.508660\\ &  &  &  &  & Kodak 22: 0.466040\\ &  &  &  &  & Kodak 23: 0.451750\\ &  &  &  &  & Kodak 24: 0.459128\\\hline\hline153 & MSE & 0.2 & 5x5deconv,2,60 & 5x5deconv,2,174 & Kodak 1: 0.160207\\ &  &  & 5x5deconv,2,54 & 5x5deconv,2,50 & Kodak 2: 0.160663\\ &  &  & 5x5deconv,2,320 & 5x5deconv,2,68 & Kodak 3: 0.164878\\ &  &  &  & 5x5deconv,2,3 & Kodak 4: 0.158647\\ &  &  &  &  & Kodak 5: 0.156206\\ &  &  &  &  & Kodak 6: 0.163826\\ &  &  &  &  & Kodak 7: 0.156649\\ &  &  &  &  & Kodak 8: 0.173277\\ &  &  &  &  & Kodak 9: 0.157669\\ &  &  &  &  & Kodak 10: 0.161512\\ &  &  &  &  & Kodak 11: 0.151613\\ &  &  &  &  & Kodak 12: 0.158649\\ &  &  &  &  & Kodak 13: 0.151820\\ &  &  &  &  & Kodak 14: 0.163956\\ &  &  &  &  & Kodak 15: 0.150117\\ &  &  &  &  & Kodak 16: 0.158120\\ &  &  &  &  & Kodak 17: 0.152917\\ &  &  &  &  & Kodak 18: 0.148388\\ &  &  &  &  & Kodak 19: 0.155658\\ &  &  &  &  & Kodak 20: 0.164731\\ &  &  &  &  & Kodak 21: 0.157921\\ &  &  &  &  & Kodak 22: 0.160211\\ &  &  &  &  & Kodak 23: 0.154411\\ &  &  &  &  & Kodak 24: 0.157945\\\hline\hline154 & MSE & 0.2 & 5x5deconv,2,7 & 5x5deconv,2,43 & Kodak 1: 0.132144\\ &  &  & 5x5deconv,2,9 & 5x5deconv,2,20 & Kodak 2: 0.117656\\ &  &  & 5x5deconv,2,320 & 5x5deconv,2,11 & Kodak 3: 0.111721\\ &  &  &  & 5x5deconv,2,3 & Kodak 4: 0.119142\\ &  &  &  &  & Kodak 5: 0.123009\\ &  &  &  &  & Kodak 6: 0.120729\\ &  &  &  &  & Kodak 7: 0.109796\\ &  &  &  &  & Kodak 8: 0.115665\\ &  &  &  &  & Kodak 9: 0.115240\\ &  &  &  &  & Kodak 10: 0.111905\\ &  &  &  &  & Kodak 11: 0.122182\\ &  &  &  &  & Kodak 12: 0.123619\\ &  &  &  &  & Kodak 13: 0.124812\\ &  &  &  &  & Kodak 14: 0.120890\\ &  &  &  &  & Kodak 15: 0.112994\\ &  &  &  &  & Kodak 16: 0.121618\\ &  &  &  &  & Kodak 17: 0.112041\\ &  &  &  &  & Kodak 18: 0.119907\\ &  &  &  &  & Kodak 19: 0.113241\\ &  &  &  &  & Kodak 20: 0.112277\\ &  &  &  &  & Kodak 21: 0.117651\\ &  &  &  &  & Kodak 22: 0.123493\\ &  &  &  &  & Kodak 23: 0.111771\\ &  &  &  &  & Kodak 24: 0.115911\\\hline\hline155 & MSE & 0.2 & 5x5deconv,2,408 & 5x5deconv,2,320 & Kodak 1: 0.507472\\ &  &  & 5x5deconv,2,287 & 5x5deconv,2,319 & Kodak 2: 0.489833\\ &  &  & 5x5deconv,2,320 & 5x5deconv,2,314 & Kodak 3: 0.484900\\ &  &  &  & 5x5deconv,2,3 & Kodak 4: 0.479071\\ &  &  &  &  & Kodak 5: 0.483050\\ &  &  &  &  & Kodak 6: 0.478079\\ &  &  &  &  & Kodak 7: 0.477650\\ &  &  &  &  & Kodak 8: 0.489758\\ &  &  &  &  & Kodak 9: 0.530026\\ &  &  &  &  & Kodak 10: 0.476621\\ &  &  &  &  & Kodak 11: 0.530632\\ &  &  &  &  & Kodak 12: 0.483006\\ &  &  &  &  & Kodak 13: 0.477010\\ &  &  &  &  & Kodak 14: 0.481191\\ &  &  &  &  & Kodak 15: 0.488068\\ &  &  &  &  & Kodak 16: 0.531639\\ &  &  &  &  & Kodak 17: 0.476623\\ &  &  &  &  & Kodak 18: 0.477350\\ &  &  &  &  & Kodak 19: 0.523751\\ &  &  &  &  & Kodak 20: 0.478802\\ &  &  &  &  & Kodak 21: 0.478432\\ &  &  &  &  & Kodak 22: 0.490986\\ &  &  &  &  & Kodak 23: 0.479552\\ &  &  &  &  & Kodak 24: 0.480689\\\hline\hline156 & MSE & 0.2 & 5x5deconv,2,175 & 5x5deconv,2,320 & Kodak 1: 0.495158\\ &  &  & 5x5deconv,2,297 & 5x5deconv,2,320 & Kodak 2: 0.474038\\ &  &  & 5x5deconv,2,320 & 5x5deconv,2,320 & Kodak 3: 0.475004\\ &  &  &  & 5x5deconv,2,3 & Kodak 4: 0.483538\\ &  &  &  &  & Kodak 5: 0.482387\\ &  &  &  &  & Kodak 6: 0.470134\\ &  &  &  &  & Kodak 7: 0.468093\\ &  &  &  &  & Kodak 8: 0.532650\\ &  &  &  &  & Kodak 9: 0.473692\\ &  &  &  &  & Kodak 10: 0.478169\\ &  &  &  &  & Kodak 11: 0.475534\\ &  &  &  &  & Kodak 12: 0.473051\\ &  &  &  &  & Kodak 13: 0.488297\\ &  &  &  &  & Kodak 14: 0.479340\\ &  &  &  &  & Kodak 15: 0.476187\\ &  &  &  &  & Kodak 16: 0.470799\\ &  &  &  &  & Kodak 17: 0.470509\\ &  &  &  &  & Kodak 18: 0.475570\\ &  &  &  &  & Kodak 19: 0.480157\\ &  &  &  &  & Kodak 20: 0.472443\\ &  &  &  &  & Kodak 21: 0.520774\\ &  &  &  &  & Kodak 22: 0.484067\\ &  &  &  &  & Kodak 23: 0.471795\\ &  &  &  &  & Kodak 24: 0.480558\\\hline\hline157 & MSE & 0.2 & 5x5deconv,2,22 & 5x5deconv,2,320 & Kodak 1: 0.480551\\ &  &  & 5x5deconv,2,17 & 5x5deconv,2,320 & Kodak 2: 0.460371\\ &  &  & 5x5deconv,2,320 & 5x5deconv,2,301 & Kodak 3: 0.454990\\ &  &  &  & 5x5deconv,2,3 & Kodak 4: 0.455996\\ &  &  &  &  & Kodak 5: 0.460384\\ &  &  &  &  & Kodak 6: 0.458334\\ &  &  &  &  & Kodak 7: 0.516327\\ &  &  &  &  & Kodak 8: 0.500230\\ &  &  &  &  & Kodak 9: 0.452583\\ &  &  &  &  & Kodak 10: 0.461612\\ &  &  &  &  & Kodak 11: 0.461253\\ &  &  &  &  & Kodak 12: 0.459937\\ &  &  &  &  & Kodak 13: 0.513088\\ &  &  &  &  & Kodak 14: 0.463863\\ &  &  &  &  & Kodak 15: 0.455560\\ &  &  &  &  & Kodak 16: 0.457069\\ &  &  &  &  & Kodak 17: 0.488597\\ &  &  &  &  & Kodak 18: 0.458163\\ &  &  &  &  & Kodak 19: 0.493887\\ &  &  &  &  & Kodak 20: 0.457921\\ &  &  &  &  & Kodak 21: 0.464995\\ &  &  &  &  & Kodak 22: 0.463697\\ &  &  &  &  & Kodak 23: 0.455648\\ &  &  &  &  & Kodak 24: 0.461126\\\hline\hline158 & MSE & 0.2 & 5x5deconv,2,410 & 5x5deconv,2,320 & Kodak 1: 0.464282\\ &  &  & 5x5deconv,2,291 & 5x5deconv,2,274 & Kodak 2: 0.430423\\ &  &  & 5x5deconv,2,320 & 5x5deconv,2,299 & Kodak 3: 0.432318\\ &  &  &  & 5x5deconv,2,3 & Kodak 4: 0.426595\\ &  &  &  &  & Kodak 5: 0.440550\\ &  &  &  &  & Kodak 6: 0.432459\\ &  &  &  &  & Kodak 7: 0.427310\\ &  &  &  &  & Kodak 8: 0.431967\\ &  &  &  &  & Kodak 9: 0.428695\\ &  &  &  &  & Kodak 10: 0.434085\\ &  &  &  &  & Kodak 11: 0.428018\\ &  &  &  &  & Kodak 12: 0.425410\\ &  &  &  &  & Kodak 13: 0.440183\\ &  &  &  &  & Kodak 14: 0.438110\\ &  &  &  &  & Kodak 15: 0.429132\\ &  &  &  &  & Kodak 16: 0.427356\\ &  &  &  &  & Kodak 17: 0.430538\\ &  &  &  &  & Kodak 18: 0.438744\\ &  &  &  &  & Kodak 19: 0.425408\\ &  &  &  &  & Kodak 20: 0.431574\\ &  &  &  &  & Kodak 21: 0.433571\\ &  &  &  &  & Kodak 22: 0.473522\\ &  &  &  &  & Kodak 23: 0.427955\\ &  &  &  &  & Kodak 24: 0.434413\\\hline\hline159 & MSE & 0.2 & 5x5deconv,2,159 & 5x5deconv,2,320 & Kodak 1: 0.502085\\ &  &  & 5x5deconv,2,482 & 5x5deconv,2,320 & Kodak 2: 0.475873\\ &  &  & 5x5deconv,2,320 & 5x5deconv,2,320 & Kodak 3: 0.475347\\ &  &  &  & 5x5deconv,2,3 & Kodak 4: 0.470848\\ &  &  &  &  & Kodak 5: 0.477581\\ &  &  &  &  & Kodak 6: 0.479789\\ &  &  &  &  & Kodak 7: 0.468709\\ &  &  &  &  & Kodak 8: 0.478816\\ &  &  &  &  & Kodak 9: 0.477878\\ &  &  &  &  & Kodak 10: 0.476848\\ &  &  &  &  & Kodak 11: 0.476653\\ &  &  &  &  & Kodak 12: 0.473594\\ &  &  &  &  & Kodak 13: 0.494087\\ &  &  &  &  & Kodak 14: 0.492657\\ &  &  &  &  & Kodak 15: 0.533477\\ &  &  &  &  & Kodak 16: 0.486097\\ &  &  &  &  & Kodak 17: 0.472496\\ &  &  &  &  & Kodak 18: 0.476066\\ &  &  &  &  & Kodak 19: 0.476433\\ &  &  &  &  & Kodak 20: 0.470531\\ &  &  &  &  & Kodak 21: 0.497577\\ &  &  &  &  & Kodak 22: 0.482138\\ &  &  &  &  & Kodak 23: 0.475282\\ &  &  &  &  & Kodak 24: 0.474423\\\hline\hline160 & MS-SSIM & 32.0 & 5x5deconv,2,10 & 5x5deconv,2,25 & Kodak 1: 0.120456\\ &  &  & 5x5deconv,2,10 & 5x5deconv,2,21 & Kodak 2: 0.109877\\ &  &  & 5x5deconv,2,320 & 5x5deconv,2,9 & Kodak 3: 0.108121\\ &  &  &  & 5x5deconv,2,3 & Kodak 4: 0.114504\\ &  &  &  &  & Kodak 5: 0.119040\\ &  &  &  &  & Kodak 6: 0.113946\\ &  &  &  &  & Kodak 7: 0.112832\\ &  &  &  &  & Kodak 8: 0.115880\\ &  &  &  &  & Kodak 9: 0.108133\\ &  &  &  &  & Kodak 10: 0.109028\\ &  &  &  &  & Kodak 11: 0.115051\\ &  &  &  &  & Kodak 12: 0.116684\\ &  &  &  &  & Kodak 13: 0.116418\\ &  &  &  &  & Kodak 14: 0.124150\\ &  &  &  &  & Kodak 15: 0.110820\\ &  &  &  &  & Kodak 16: 0.112882\\ &  &  &  &  & Kodak 17: 0.113405\\ &  &  &  &  & Kodak 18: 0.113422\\ &  &  &  &  & Kodak 19: 0.106244\\ &  &  &  &  & Kodak 20: 0.114730\\ &  &  &  &  & Kodak 21: 0.116578\\ &  &  &  &  & Kodak 22: 0.113423\\ &  &  &  &  & Kodak 23: 0.115912\\ &  &  &  &  & Kodak 24: 0.111655\\\hline\hline161 & MS-SSIM & 32.0 & 5x5deconv,2,38 & 5x5deconv,2,125 & Kodak 1: 0.133678\\ &  &  & 5x5deconv,2,47 & 5x5deconv,2,35 & Kodak 2: 0.142491\\ &  &  & 5x5deconv,2,320 & 5x5deconv,2,36 & Kodak 3: 0.129006\\ &  &  &  & 5x5deconv,2,3 & Kodak 4: 0.135270\\ &  &  &  &  & Kodak 5: 0.133333\\ &  &  &  &  & Kodak 6: 0.133344\\ &  &  &  &  & Kodak 7: 0.138022\\ &  &  &  &  & Kodak 8: 0.136866\\ &  &  &  &  & Kodak 9: 0.128668\\ &  &  &  &  & Kodak 10: 0.144826\\ &  &  &  &  & Kodak 11: 0.139559\\ &  &  &  &  & Kodak 12: 0.140850\\ &  &  &  &  & Kodak 13: 0.134354\\ &  &  &  &  & Kodak 14: 0.126590\\ &  &  &  &  & Kodak 15: 0.142494\\ &  &  &  &  & Kodak 16: 0.140908\\ &  &  &  &  & Kodak 17: 0.136242\\ &  &  &  &  & Kodak 18: 0.145618\\ &  &  &  &  & Kodak 19: 0.127129\\ &  &  &  &  & Kodak 20: 0.137428\\ &  &  &  &  & Kodak 21: 0.136000\\ &  &  &  &  & Kodak 22: 0.136022\\ &  &  &  &  & Kodak 23: 0.136413\\ &  &  &  &  & Kodak 24: 0.135622\\\hline\hline162 & MS-SSIM & 32.0 & 5x5deconv,2,133 & 5x5deconv,2,299 & Kodak 1: 0.301811\\ &  &  & 5x5deconv,2,222 & 5x5deconv,2,171 & Kodak 2: 0.273392\\ &  &  & 5x5deconv,2,320 & 5x5deconv,2,182 & Kodak 3: 0.274760\\ &  &  &  & 5x5deconv,2,3 & Kodak 4: 0.279317\\ &  &  &  &  & Kodak 5: 0.279362\\ &  &  &  &  & Kodak 6: 0.278695\\ &  &  &  &  & Kodak 7: 0.272504\\ &  &  &  &  & Kodak 8: 0.279676\\ &  &  &  &  & Kodak 9: 0.274956\\ &  &  &  &  & Kodak 10: 0.271814\\ &  &  &  &  & Kodak 11: 0.271409\\ &  &  &  &  & Kodak 12: 0.272288\\ &  &  &  &  & Kodak 13: 0.276345\\ &  &  &  &  & Kodak 14: 0.283040\\ &  &  &  &  & Kodak 15: 0.274637\\ &  &  &  &  & Kodak 16: 0.281584\\ &  &  &  &  & Kodak 17: 0.278567\\ &  &  &  &  & Kodak 18: 0.278755\\ &  &  &  &  & Kodak 19: 0.293521\\ &  &  &  &  & Kodak 20: 0.275036\\ &  &  &  &  & Kodak 21: 0.294390\\ &  &  &  &  & Kodak 22: 0.278761\\ &  &  &  &  & Kodak 23: 0.278052\\ &  &  &  &  & Kodak 24: 0.272422\\\hline\hline163 & MS-SSIM & 32.0 & 5x5deconv,2,10 & 5x5deconv,2,25 & Kodak 1: 0.112235\\ &  &  & 5x5deconv,2,10 & 5x5deconv,2,21 & Kodak 2: 0.112820\\ &  &  & 5x5deconv,2,320 & 5x5deconv,2,9 & Kodak 3: 0.107536\\ &  &  &  & 5x5deconv,2,3 & Kodak 4: 0.110974\\ &  &  &  &  & Kodak 5: 0.117255\\ &  &  &  &  & Kodak 6: 0.110562\\ &  &  &  &  & Kodak 7: 0.114314\\ &  &  &  &  & Kodak 8: 0.111256\\ &  &  &  &  & Kodak 9: 0.114524\\ &  &  &  &  & Kodak 10: 0.124340\\ &  &  &  &  & Kodak 11: 0.119958\\ &  &  &  &  & Kodak 12: 0.109064\\ &  &  &  &  & Kodak 13: 0.113346\\ &  &  &  &  & Kodak 14: 0.116168\\ &  &  &  &  & Kodak 15: 0.112970\\ &  &  &  &  & Kodak 16: 0.113147\\ &  &  &  &  & Kodak 17: 0.111269\\ &  &  &  &  & Kodak 18: 0.116185\\ &  &  &  &  & Kodak 19: 0.120691\\ &  &  &  &  & Kodak 20: 0.107421\\ &  &  &  &  & Kodak 21: 0.114532\\ &  &  &  &  & Kodak 22: 0.123120\\ &  &  &  &  & Kodak 23: 0.120367\\ &  &  &  &  & Kodak 24: 0.113240\\\hline\hline164 & MS-SSIM & 32.0 & 5x5deconv,2,127 & 5x5deconv,2,257 & Kodak 1: 0.220361\\ &  &  & 5x5deconv,2,203 & 5x5deconv,2,110 & Kodak 2: 0.204460\\ &  &  & 5x5deconv,2,320 & 5x5deconv,2,117 & Kodak 3: 0.209394\\ &  &  &  & 5x5deconv,2,3 & Kodak 4: 0.205221\\ &  &  &  &  & Kodak 5: 0.208783\\ &  &  &  &  & Kodak 6: 0.207168\\ &  &  &  &  & Kodak 7: 0.232608\\ &  &  &  &  & Kodak 8: 0.208855\\ &  &  &  &  & Kodak 9: 0.211122\\ &  &  &  &  & Kodak 10: 0.204620\\ &  &  &  &  & Kodak 11: 0.226304\\ &  &  &  &  & Kodak 12: 0.211376\\ &  &  &  &  & Kodak 13: 0.208787\\ &  &  &  &  & Kodak 14: 0.207753\\ &  &  &  &  & Kodak 15: 0.208689\\ &  &  &  &  & Kodak 16: 0.208175\\ &  &  &  &  & Kodak 17: 0.216856\\ &  &  &  &  & Kodak 18: 0.232696\\ &  &  &  &  & Kodak 19: 0.210485\\ &  &  &  &  & Kodak 20: 0.209171\\ &  &  &  &  & Kodak 21: 0.220761\\ &  &  &  &  & Kodak 22: 0.206973\\ &  &  &  &  & Kodak 23: 0.203510\\ &  &  &  &  & Kodak 24: 0.205593\\\hline\hline165 & MS-SSIM & 32.0 & 5x5deconv,2,10 & 5x5deconv,2,1 & Kodak 1: 0.088686\\ &  &  & 5x5deconv,2,10 & 5x5deconv,2,1 & Kodak 2: 0.096726\\ &  &  & 5x5deconv,2,320 & 5x5deconv,2,1 & Kodak 3: 0.103325\\ &  &  &  & 5x5deconv,2,3 & Kodak 4: 0.096599\\ &  &  &  &  & Kodak 5: 0.097434\\ &  &  &  &  & Kodak 6: 0.097508\\ &  &  &  &  & Kodak 7: 0.097465\\ &  &  &  &  & Kodak 8: 0.097931\\ &  &  &  &  & Kodak 9: 0.097946\\ &  &  &  &  & Kodak 10: 0.095971\\ &  &  &  &  & Kodak 11: 0.099215\\ &  &  &  &  & Kodak 12: 0.099715\\ &  &  &  &  & Kodak 13: 0.095095\\ &  &  &  &  & Kodak 14: 0.100629\\ &  &  &  &  & Kodak 15: 0.094883\\ &  &  &  &  & Kodak 16: 0.095307\\ &  &  &  &  & Kodak 17: 0.097414\\ &  &  &  &  & Kodak 18: 0.101731\\ &  &  &  &  & Kodak 19: 0.097508\\ &  &  &  &  & Kodak 20: 0.095628\\ &  &  &  &  & Kodak 21: 0.094184\\ &  &  &  &  & Kodak 22: 0.094835\\ &  &  &  &  & Kodak 23: 0.096347\\ &  &  &  &  & Kodak 24: 0.093664\\\hline\hline166 & MS-SSIM & 32.0 & 5x5deconv,2,10 & 5x5deconv,2,1 & Kodak 1: 0.089014\\ &  &  & 5x5deconv,2,10 & 5x5deconv,2,1 & Kodak 2: 0.095749\\ &  &  & 5x5deconv,2,320 & 5x5deconv,2,1 & Kodak 3: 0.095666\\ &  &  &  & 5x5deconv,2,3 & Kodak 4: 0.095597\\ &  &  &  &  & Kodak 5: 0.098292\\ &  &  &  &  & Kodak 6: 0.096038\\ &  &  &  &  & Kodak 7: 0.093437\\ &  &  &  &  & Kodak 8: 0.094970\\ &  &  &  &  & Kodak 9: 0.093913\\ &  &  &  &  & Kodak 10: 0.100258\\ &  &  &  &  & Kodak 11: 0.098430\\ &  &  &  &  & Kodak 12: 0.095071\\ &  &  &  &  & Kodak 13: 0.101716\\ &  &  &  &  & Kodak 14: 0.108751\\ &  &  &  &  & Kodak 15: 0.092836\\ &  &  &  &  & Kodak 16: 0.095178\\ &  &  &  &  & Kodak 17: 0.097871\\ &  &  &  &  & Kodak 18: 0.098371\\ &  &  &  &  & Kodak 19: 0.096416\\ &  &  &  &  & Kodak 20: 0.098957\\ &  &  &  &  & Kodak 21: 0.097700\\ &  &  &  &  & Kodak 22: 0.096797\\ &  &  &  &  & Kodak 23: 0.099113\\ &  &  &  &  & Kodak 24: 0.096234\\\hline\hline167 & MS-SSIM & 32.0 & 5x5deconv,2,10 & 5x5deconv,2,1 & Kodak 1: 0.087427\\ &  &  & 5x5deconv,2,10 & 5x5deconv,2,1 & Kodak 2: 0.095901\\ &  &  & 5x5deconv,2,320 & 5x5deconv,2,1 & Kodak 3: 0.095449\\ &  &  &  & 5x5deconv,2,3 & Kodak 4: 0.097404\\ &  &  &  &  & Kodak 5: 0.095418\\ &  &  &  &  & Kodak 6: 0.095644\\ &  &  &  &  & Kodak 7: 0.094300\\ &  &  &  &  & Kodak 8: 0.097656\\ &  &  &  &  & Kodak 9: 0.103691\\ &  &  &  &  & Kodak 10: 0.103610\\ &  &  &  &  & Kodak 11: 0.091504\\ &  &  &  &  & Kodak 12: 0.094639\\ &  &  &  &  & Kodak 13: 0.096512\\ &  &  &  &  & Kodak 14: 0.093880\\ &  &  &  &  & Kodak 15: 0.096588\\ &  &  &  &  & Kodak 16: 0.092834\\ &  &  &  &  & Kodak 17: 0.095476\\ &  &  &  &  & Kodak 18: 0.096027\\ &  &  &  &  & Kodak 19: 0.099179\\ &  &  &  &  & Kodak 20: 0.093008\\ &  &  &  &  & Kodak 21: 0.096652\\ &  &  &  &  & Kodak 22: 0.094547\\ &  &  &  &  & Kodak 23: 0.096325\\ &  &  &  &  & Kodak 24: 0.093908\\\hline\hline\hline\hline169 & MS-SSIM & 32.0 & 5x5deconv,2,10 & 5x5deconv,2,1 & Kodak 1: 0.091560\\ &  &  & 5x5deconv,2,10 & 5x5deconv,2,1 & Kodak 2: 0.094823\\ &  &  & 5x5deconv,2,320 & 5x5deconv,2,1 & Kodak 3: 0.097641\\ &  &  &  & 5x5deconv,2,3 & Kodak 4: 0.097963\\ &  &  &  &  & Kodak 5: 0.097186\\ &  &  &  &  & Kodak 6: 0.094511\\ &  &  &  &  & Kodak 7: 0.098501\\ &  &  &  &  & Kodak 8: 0.097258\\ &  &  &  &  & Kodak 9: 0.095097\\ &  &  &  &  & Kodak 10: 0.096929\\ &  &  &  &  & Kodak 11: 0.098962\\ &  &  &  &  & Kodak 12: 0.095068\\ &  &  &  &  & Kodak 13: 0.094094\\ &  &  &  &  & Kodak 14: 0.093390\\ &  &  &  &  & Kodak 15: 0.095743\\ &  &  &  &  & Kodak 16: 0.094178\\ &  &  &  &  & Kodak 17: 0.095623\\ &  &  &  &  & Kodak 18: 0.096115\\ &  &  &  &  & Kodak 19: 0.091458\\ &  &  &  &  & Kodak 20: 0.097820\\ &  &  &  &  & Kodak 21: 0.097795\\ &  &  &  &  & Kodak 22: 0.097298\\ &  &  &  &  & Kodak 23: 0.093556\\ &  &  &  &  & Kodak 24: 0.093437\\\hline\hline170 & MS-SSIM & 32.0 & 5x5deconv,2,10 & 5x5deconv,2,2 & Kodak 1: 0.090844\\ &  &  & 5x5deconv,2,10 & 5x5deconv,2,7 & Kodak 2: 0.096305\\ &  &  & 5x5deconv,2,320 & 5x5deconv,2,1 & Kodak 3: 0.096400\\ &  &  &  & 5x5deconv,2,3 & Kodak 4: 0.098336\\ &  &  &  &  & Kodak 5: 0.103209\\ &  &  &  &  & Kodak 6: 0.099771\\ &  &  &  &  & Kodak 7: 0.102734\\ &  &  &  &  & Kodak 8: 0.094370\\ &  &  &  &  & Kodak 9: 0.098792\\ &  &  &  &  & Kodak 10: 0.097566\\ &  &  &  &  & Kodak 11: 0.099586\\ &  &  &  &  & Kodak 12: 0.097956\\ &  &  &  &  & Kodak 13: 0.098540\\ &  &  &  &  & Kodak 14: 0.096653\\ &  &  &  &  & Kodak 15: 0.096759\\ &  &  &  &  & Kodak 16: 0.092348\\ &  &  &  &  & Kodak 17: 0.100029\\ &  &  &  &  & Kodak 18: 0.100912\\ &  &  &  &  & Kodak 19: 0.097965\\ &  &  &  &  & Kodak 20: 0.099143\\ &  &  &  &  & Kodak 21: 0.096681\\ &  &  &  &  & Kodak 22: 0.095744\\ &  &  &  &  & Kodak 23: 0.104663\\ &  &  &  &  & Kodak 24: 0.097521\\\hline\hline171 & MS-SSIM & 32.0 & 5x5deconv,2,10 & 5x5deconv,2,10 & Kodak 1: 0.094066\\ &  &  & 5x5deconv,2,10 & 5x5deconv,2,12 & Kodak 2: 0.104317\\ &  &  & 5x5deconv,2,320 & 5x5deconv,2,2 & Kodak 3: 0.102328\\ &  &  &  & 5x5deconv,2,3 & Kodak 4: 0.104336\\ &  &  &  &  & Kodak 5: 0.103654\\ &  &  &  &  & Kodak 6: 0.099808\\ &  &  &  &  & Kodak 7: 0.100822\\ &  &  &  &  & Kodak 8: 0.098455\\ &  &  &  &  & Kodak 9: 0.099632\\ &  &  &  &  & Kodak 10: 0.100200\\ &  &  &  &  & Kodak 11: 0.097265\\ &  &  &  &  & Kodak 12: 0.100869\\ &  &  &  &  & Kodak 13: 0.100485\\ &  &  &  &  & Kodak 14: 0.106404\\ &  &  &  &  & Kodak 15: 0.101837\\ &  &  &  &  & Kodak 16: 0.101688\\ &  &  &  &  & Kodak 17: 0.104071\\ &  &  &  &  & Kodak 18: 0.106429\\ &  &  &  &  & Kodak 19: 0.100989\\ &  &  &  &  & Kodak 20: 0.100092\\ &  &  &  &  & Kodak 21: 0.102381\\ &  &  &  &  & Kodak 22: 0.108313\\ &  &  &  &  & Kodak 23: 0.101330\\ &  &  &  &  & Kodak 24: 0.102200\\\hline\hline172 & MS-SSIM & 32.0 & 5x5deconv,2,18 & 5x5deconv,2,65 & Kodak 1: 0.124459\\ &  &  & 5x5deconv,2,46 & 5x5deconv,2,20 & Kodak 2: 0.129198\\ &  &  & 5x5deconv,2,320 & 5x5deconv,2,21 & Kodak 3: 0.142913\\ &  &  &  & 5x5deconv,2,3 & Kodak 4: 0.139121\\ &  &  &  &  & Kodak 5: 0.133520\\ &  &  &  &  & Kodak 6: 0.124983\\ &  &  &  &  & Kodak 7: 0.121064\\ &  &  &  &  & Kodak 8: 0.125611\\ &  &  &  &  & Kodak 9: 0.119424\\ &  &  &  &  & Kodak 10: 0.124876\\ &  &  &  &  & Kodak 11: 0.126727\\ &  &  &  &  & Kodak 12: 0.125575\\ &  &  &  &  & Kodak 13: 0.120437\\ &  &  &  &  & Kodak 14: 0.125041\\ &  &  &  &  & Kodak 15: 0.130199\\ &  &  &  &  & Kodak 16: 0.116382\\ &  &  &  &  & Kodak 17: 0.116743\\ &  &  &  &  & Kodak 18: 0.133121\\ &  &  &  &  & Kodak 19: 0.125902\\ &  &  &  &  & Kodak 20: 0.120788\\ &  &  &  &  & Kodak 21: 0.131217\\ &  &  &  &  & Kodak 22: 0.128599\\ &  &  &  &  & Kodak 23: 0.119483\\ &  &  &  &  & Kodak 24: 0.121689\\\hline\hline173 & MSE & 0.0125 & 5x5deconv,2,54 & 5x5deconv,2,83 & Kodak 1: 0.129891\\ &  &  & 5x5deconv,2,76 & 5x5deconv,2,34 & Kodak 2: 0.136549\\ &  &  & 5x5deconv,2,320 & 5x5deconv,2,50 & Kodak 3: 0.134352\\ &  &  &  & 5x5deconv,2,3 & Kodak 4: 0.137699\\ &  &  &  &  & Kodak 5: 0.134173\\ &  &  &  &  & Kodak 6: 0.137700\\ &  &  &  &  & Kodak 7: 0.140566\\ &  &  &  &  & Kodak 8: 0.138710\\ &  &  &  &  & Kodak 9: 0.132510\\ &  &  &  &  & Kodak 10: 0.141136\\ &  &  &  &  & Kodak 11: 0.130179\\ &  &  &  &  & Kodak 12: 0.138949\\ &  &  &  &  & Kodak 13: 0.139509\\ &  &  &  &  & Kodak 14: 0.140781\\ &  &  &  &  & Kodak 15: 0.138058\\ &  &  &  &  & Kodak 16: 0.131278\\ &  &  &  &  & Kodak 17: 0.126063\\ &  &  &  &  & Kodak 18: 0.142900\\ &  &  &  &  & Kodak 19: 0.130284\\ &  &  &  &  & Kodak 20: 0.127855\\ &  &  &  &  & Kodak 21: 0.139130\\ &  &  &  &  & Kodak 22: 0.133985\\ &  &  &  &  & Kodak 23: 0.128615\\ &  &  &  &  & Kodak 24: 0.133263\\\hline\hline174 & MSE & 0.0125 & 5x5deconv,2,7 & 5x5deconv,2,16 & Kodak 1: 0.100964\\ &  &  & 5x5deconv,2,14 & 5x5deconv,2,16 & Kodak 2: 0.104259\\ &  &  & 5x5deconv,2,320 & 5x5deconv,2,9 & Kodak 3: 0.102735\\ &  &  &  & 5x5deconv,2,3 & Kodak 4: 0.103291\\ &  &  &  &  & Kodak 5: 0.112951\\ &  &  &  &  & Kodak 6: 0.112303\\ &  &  &  &  & Kodak 7: 0.106736\\ &  &  &  &  & Kodak 8: 0.103830\\ &  &  &  &  & Kodak 9: 0.104688\\ &  &  &  &  & Kodak 10: 0.103222\\ &  &  &  &  & Kodak 11: 0.109775\\ &  &  &  &  & Kodak 12: 0.100568\\ &  &  &  &  & Kodak 13: 0.105245\\ &  &  &  &  & Kodak 14: 0.107531\\ &  &  &  &  & Kodak 15: 0.108309\\ &  &  &  &  & Kodak 16: 0.106410\\ &  &  &  &  & Kodak 17: 0.114047\\ &  &  &  &  & Kodak 18: 0.107317\\ &  &  &  &  & Kodak 19: 0.101910\\ &  &  &  &  & Kodak 20: 0.109379\\ &  &  &  &  & Kodak 21: 0.102524\\ &  &  &  &  & Kodak 22: 0.104049\\ &  &  &  &  & Kodak 23: 0.108357\\ &  &  &  &  & Kodak 24: 0.104893\\\hline\hline175 & MSE & 0.0125 & 5x5deconv,2,10 & 5x5deconv,2,1 & Kodak 1: 0.089998\\ &  &  & 5x5deconv,2,10 & 5x5deconv,2,8 & Kodak 2: 0.097005\\ &  &  & 5x5deconv,2,320 & 5x5deconv,2,1 & Kodak 3: 0.101774\\ &  &  &  & 5x5deconv,2,3 & Kodak 4: 0.105974\\ &  &  &  &  & Kodak 5: 0.100516\\ &  &  &  &  & Kodak 6: 0.100017\\ &  &  &  &  & Kodak 7: 0.097400\\ &  &  &  &  & Kodak 8: 0.097931\\ &  &  &  &  & Kodak 9: 0.096009\\ &  &  &  &  & Kodak 10: 0.097202\\ &  &  &  &  & Kodak 11: 0.099132\\ &  &  &  &  & Kodak 12: 0.098206\\ &  &  &  &  & Kodak 13: 0.102643\\ &  &  &  &  & Kodak 14: 0.097349\\ &  &  &  &  & Kodak 15: 0.096104\\ &  &  &  &  & Kodak 16: 0.096373\\ &  &  &  &  & Kodak 17: 0.095639\\ &  &  &  &  & Kodak 18: 0.094805\\ &  &  &  &  & Kodak 19: 0.098807\\ &  &  &  &  & Kodak 20: 0.098251\\ &  &  &  &  & Kodak 21: 0.098585\\ &  &  &  &  & Kodak 22: 0.100711\\ &  &  &  &  & Kodak 23: 0.097782\\ &  &  &  &  & Kodak 24: 0.099303\\\hline\hline176 & MSE & 0.0125 & 5x5deconv,2,156 & 5x5deconv,2,238 & Kodak 1: 0.231516\\ &  &  & 5x5deconv,2,116 & 5x5deconv,2,86 & Kodak 2: 0.218838\\ &  &  & 5x5deconv,2,320 & 5x5deconv,2,154 & Kodak 3: 0.236907\\ &  &  &  & 5x5deconv,2,3 & Kodak 4: 0.224717\\ &  &  &  &  & Kodak 5: 0.222304\\ &  &  &  &  & Kodak 6: 0.217144\\ &  &  &  &  & Kodak 7: 0.218522\\ &  &  &  &  & Kodak 8: 0.226248\\ &  &  &  &  & Kodak 9: 0.210893\\ &  &  &  &  & Kodak 10: 0.213372\\ &  &  &  &  & Kodak 11: 0.210674\\ &  &  &  &  & Kodak 12: 0.235466\\ &  &  &  &  & Kodak 13: 0.212789\\ &  &  &  &  & Kodak 14: 0.217908\\ &  &  &  &  & Kodak 15: 0.221124\\ &  &  &  &  & Kodak 16: 0.217276\\ &  &  &  &  & Kodak 17: 0.212905\\ &  &  &  &  & Kodak 18: 0.223217\\ &  &  &  &  & Kodak 19: 0.215336\\ &  &  &  &  & Kodak 20: 0.220740\\ &  &  &  &  & Kodak 21: 0.216770\\ &  &  &  &  & Kodak 22: 0.219545\\ &  &  &  &  & Kodak 23: 0.233540\\ &  &  &  &  & Kodak 24: 0.219837\\\hline\hline177 & MSE & 0.0125 & 5x5deconv,2,10 & 5x5deconv,2,1 & Kodak 1: 0.091936\\ &  &  & 5x5deconv,2,10 & 5x5deconv,2,2 & Kodak 2: 0.100810\\ &  &  & 5x5deconv,2,320 & 5x5deconv,2,1 & Kodak 3: 0.098719\\ &  &  &  & 5x5deconv,2,3 & Kodak 4: 0.101710\\ &  &  &  &  & Kodak 5: 0.100749\\ &  &  &  &  & Kodak 6: 0.098669\\ &  &  &  &  & Kodak 7: 0.095218\\ &  &  &  &  & Kodak 8: 0.097391\\ &  &  &  &  & Kodak 9: 0.098561\\ &  &  &  &  & Kodak 10: 0.096406\\ &  &  &  &  & Kodak 11: 0.103915\\ &  &  &  &  & Kodak 12: 0.102879\\ &  &  &  &  & Kodak 13: 0.098727\\ &  &  &  &  & Kodak 14: 0.096098\\ &  &  &  &  & Kodak 15: 0.105441\\ &  &  &  &  & Kodak 16: 0.100678\\ &  &  &  &  & Kodak 17: 0.099358\\ &  &  &  &  & Kodak 18: 0.103814\\ &  &  &  &  & Kodak 19: 0.098594\\ &  &  &  &  & Kodak 20: 0.101408\\ &  &  &  &  & Kodak 21: 0.097724\\ &  &  &  &  & Kodak 22: 0.096027\\ &  &  &  &  & Kodak 23: 0.102995\\ &  &  &  &  & Kodak 24: 0.098334\\\hline\hline178 & MSE & 0.0125 & 5x5deconv,2,27 & 5x5deconv,2,38 & Kodak 1: 0.125642\\ &  &  & 5x5deconv,2,31 & 5x5deconv,2,17 & Kodak 2: 0.118532\\ &  &  & 5x5deconv,2,320 & 5x5deconv,2,33 & Kodak 3: 0.113311\\ &  &  &  & 5x5deconv,2,3 & Kodak 4: 0.112836\\ &  &  &  &  & Kodak 5: 0.112552\\ &  &  &  &  & Kodak 6: 0.115625\\ &  &  &  &  & Kodak 7: 0.119033\\ &  &  &  &  & Kodak 8: 0.125961\\ &  &  &  &  & Kodak 9: 0.118549\\ &  &  &  &  & Kodak 10: 0.120070\\ &  &  &  &  & Kodak 11: 0.117989\\ &  &  &  &  & Kodak 12: 0.126276\\ &  &  &  &  & Kodak 13: 0.118745\\ &  &  &  &  & Kodak 14: 0.118206\\ &  &  &  &  & Kodak 15: 0.113539\\ &  &  &  &  & Kodak 16: 0.121114\\ &  &  &  &  & Kodak 17: 0.121345\\ &  &  &  &  & Kodak 18: 0.120813\\ &  &  &  &  & Kodak 19: 0.118158\\ &  &  &  &  & Kodak 20: 0.121360\\ &  &  &  &  & Kodak 21: 0.126581\\ &  &  &  &  & Kodak 22: 0.124281\\ &  &  &  &  & Kodak 23: 0.124278\\ &  &  &  &  & Kodak 24: 0.123591\\\hline\hline179 & MSE & 0.0125 & 5x5deconv,2,108 & 5x5deconv,2,285 & Kodak 1: 0.367908\\ &  &  & 5x5deconv,2,262 & 5x5deconv,2,166 & Kodak 2: 0.356719\\ &  &  & 5x5deconv,2,320 & 5x5deconv,2,290 & Kodak 3: 0.346682\\ &  &  &  & 5x5deconv,2,3 & Kodak 4: 0.343113\\ &  &  &  &  & Kodak 5: 0.352760\\ &  &  &  &  & Kodak 6: 0.344664\\ &  &  &  &  & Kodak 7: 0.346019\\ &  &  &  &  & Kodak 8: 0.348920\\ &  &  &  &  & Kodak 9: 0.342793\\ &  &  &  &  & Kodak 10: 0.392003\\ &  &  &  &  & Kodak 11: 0.354008\\ &  &  &  &  & Kodak 12: 0.345299\\ &  &  &  &  & Kodak 13: 0.347045\\ &  &  &  &  & Kodak 14: 0.346353\\ &  &  &  &  & Kodak 15: 0.347680\\ &  &  &  &  & Kodak 16: 0.348538\\ &  &  &  &  & Kodak 17: 0.346255\\ &  &  &  &  & Kodak 18: 0.348022\\ &  &  &  &  & Kodak 19: 0.342223\\ &  &  &  &  & Kodak 20: 0.338320\\ &  &  &  &  & Kodak 21: 0.347593\\ &  &  &  &  & Kodak 22: 0.346673\\ &  &  &  &  & Kodak 23: 0.394106\\ &  &  &  &  & Kodak 24: 0.345911\\\hline\hline180 & MSE & 0.0125 & 5x5deconv,2,259 & 5x5deconv,2,320 & Kodak 1: 0.507632\\ &  &  & 5x5deconv,2,366 & 5x5deconv,2,320 & Kodak 2: 0.489635\\ &  &  & 5x5deconv,2,320 & 5x5deconv,2,320 & Kodak 3: 0.489460\\ &  &  &  & 5x5deconv,2,3 & Kodak 4: 0.483541\\ &  &  &  &  & Kodak 5: 0.478572\\ &  &  &  &  & Kodak 6: 0.481162\\ &  &  &  &  & Kodak 7: 0.474292\\ &  &  &  &  & Kodak 8: 0.480121\\ &  &  &  &  & Kodak 9: 0.474764\\ &  &  &  &  & Kodak 10: 0.481494\\ &  &  &  &  & Kodak 11: 0.476263\\ &  &  &  &  & Kodak 12: 0.476121\\ &  &  &  &  & Kodak 13: 0.485092\\ &  &  &  &  & Kodak 14: 0.480931\\ &  &  &  &  & Kodak 15: 0.475661\\ &  &  &  &  & Kodak 16: 0.481130\\ &  &  &  &  & Kodak 17: 0.480652\\ &  &  &  &  & Kodak 18: 0.487483\\ &  &  &  &  & Kodak 19: 0.478254\\ &  &  &  &  & Kodak 20: 0.477079\\ &  &  &  &  & Kodak 21: 0.478612\\ &  &  &  &  & Kodak 22: 0.488374\\ &  &  &  &  & Kodak 23: 0.479055\\ &  &  &  &  & Kodak 24: 0.501886\\\hline\hline181 & MSE & 0.0125 & 5x5deconv,2,5 & 5x5deconv,2,8 & Kodak 1: 0.094022\\ &  &  & 5x5deconv,2,7 & 5x5deconv,2,11 & Kodak 2: 0.101600\\ &  &  & 5x5deconv,2,320 & 5x5deconv,2,1 & Kodak 3: 0.096164\\ &  &  &  & 5x5deconv,2,3 & Kodak 4: 0.098506\\ &  &  &  &  & Kodak 5: 0.102218\\ &  &  &  &  & Kodak 6: 0.100182\\ &  &  &  &  & Kodak 7: 0.096764\\ &  &  &  &  & Kodak 8: 0.099285\\ &  &  &  &  & Kodak 9: 0.096608\\ &  &  &  &  & Kodak 10: 0.100182\\ &  &  &  &  & Kodak 11: 0.101175\\ &  &  &  &  & Kodak 12: 0.097551\\ &  &  &  &  & Kodak 13: 0.099530\\ &  &  &  &  & Kodak 14: 0.096311\\ &  &  &  &  & Kodak 15: 0.098663\\ &  &  &  &  & Kodak 16: 0.099133\\ &  &  &  &  & Kodak 17: 0.099758\\ &  &  &  &  & Kodak 18: 0.095788\\ &  &  &  &  & Kodak 19: 0.099536\\ &  &  &  &  & Kodak 20: 0.095674\\ &  &  &  &  & Kodak 21: 0.098938\\ &  &  &  &  & Kodak 22: 0.109913\\ &  &  &  &  & Kodak 23: 0.096585\\ &  &  &  &  & Kodak 24: 0.095490\\\hline\hline182 & MSE & 0.0125 & 5x5deconv,2,280 & 5x5deconv,2,237 & Kodak 1: 0.279683\\ &  &  & 5x5deconv,2,164 & 5x5deconv,2,97 & Kodak 2: 0.265016\\ &  &  & 5x5deconv,2,320 & 5x5deconv,2,228 & Kodak 3: 0.261827\\ &  &  &  & 5x5deconv,2,3 & Kodak 4: 0.263034\\ &  &  &  &  & Kodak 5: 0.259177\\ &  &  &  &  & Kodak 6: 0.256857\\ &  &  &  &  & Kodak 7: 0.259893\\ &  &  &  &  & Kodak 8: 0.263974\\ &  &  &  &  & Kodak 9: 0.258426\\ &  &  &  &  & Kodak 10: 0.257766\\ &  &  &  &  & Kodak 11: 0.263722\\ &  &  &  &  & Kodak 12: 0.261144\\ &  &  &  &  & Kodak 13: 0.267292\\ &  &  &  &  & Kodak 14: 0.267852\\ &  &  &  &  & Kodak 15: 0.264286\\ &  &  &  &  & Kodak 16: 0.282401\\ &  &  &  &  & Kodak 17: 0.258513\\ &  &  &  &  & Kodak 18: 0.262791\\ &  &  &  &  & Kodak 19: 0.258958\\ &  &  &  &  & Kodak 20: 0.266447\\ &  &  &  &  & Kodak 21: 0.271954\\ &  &  &  &  & Kodak 22: 0.289626\\ &  &  &  &  & Kodak 23: 0.288730\\ &  &  &  &  & Kodak 24: 0.262968\\\hline\hline183 & MSE & 0.0125 & 5x5deconv,2,72 & 5x5deconv,2,320 & Kodak 1: 0.491970\\ &  &  & 5x5deconv,2,379 & 5x5deconv,2,320 & Kodak 2: 0.476454\\ &  &  & 5x5deconv,2,320 & 5x5deconv,2,320 & Kodak 3: 0.480409\\ &  &  &  & 5x5deconv,2,3 & Kodak 4: 0.491622\\ &  &  &  &  & Kodak 5: 0.494495\\ &  &  &  &  & Kodak 6: 0.489134\\ &  &  &  &  & Kodak 7: 0.491754\\ &  &  &  &  & Kodak 8: 0.479655\\ &  &  &  &  & Kodak 9: 0.469266\\ &  &  &  &  & Kodak 10: 0.472601\\ &  &  &  &  & Kodak 11: 0.541942\\ &  &  &  &  & Kodak 12: 0.472228\\ &  &  &  &  & Kodak 13: 0.468677\\ &  &  &  &  & Kodak 14: 0.469538\\ &  &  &  &  & Kodak 15: 0.469765\\ &  &  &  &  & Kodak 16: 0.517591\\ &  &  &  &  & Kodak 17: 0.469013\\ &  &  &  &  & Kodak 18: 0.476600\\ &  &  &  &  & Kodak 19: 0.468816\\ &  &  &  &  & Kodak 20: 0.472044\\ &  &  &  &  & Kodak 21: 0.472625\\ &  &  &  &  & Kodak 22: 0.522879\\ &  &  &  &  & Kodak 23: 0.472299\\ &  &  &  &  & Kodak 24: 0.474462\\\hline\hline184 & MSE & 0.0125 & 5x5deconv,2,10 & 5x5deconv,2,1 & Kodak 1: 0.088719\\ &  &  & 5x5deconv,2,10 & 5x5deconv,2,5 & Kodak 2: 0.094191\\ &  &  & 5x5deconv,2,320 & 5x5deconv,2,1 & Kodak 3: 0.095506\\ &  &  &  & 5x5deconv,2,3 & Kodak 4: 0.096563\\ &  &  &  &  & Kodak 5: 0.097066\\ &  &  &  &  & Kodak 6: 0.096717\\ &  &  &  &  & Kodak 7: 0.099371\\ &  &  &  &  & Kodak 8: 0.100270\\ &  &  &  &  & Kodak 9: 0.094508\\ &  &  &  &  & Kodak 10: 0.095678\\ &  &  &  &  & Kodak 11: 0.095957\\ &  &  &  &  & Kodak 12: 0.095835\\ &  &  &  &  & Kodak 13: 0.099700\\ &  &  &  &  & Kodak 14: 0.097535\\ &  &  &  &  & Kodak 15: 0.100999\\ &  &  &  &  & Kodak 16: 0.098675\\ &  &  &  &  & Kodak 17: 0.096959\\ &  &  &  &  & Kodak 18: 0.097901\\ &  &  &  &  & Kodak 19: 0.098764\\ &  &  &  &  & Kodak 20: 0.098603\\ &  &  &  &  & Kodak 21: 0.095175\\ &  &  &  &  & Kodak 22: 0.101083\\ &  &  &  &  & Kodak 23: 0.091447\\ &  &  &  &  & Kodak 24: 0.101984\\\hline\hline185 & MSE & 0.05 & 5x5deconv,2,76 & 5x5deconv,2,150 & Kodak 1: 0.187980\\ &  &  & 5x5deconv,2,107 & 5x5deconv,2,89 & Kodak 2: 0.170646\\ &  &  & 5x5deconv,2,320 & 5x5deconv,2,81 & Kodak 3: 0.178597\\ &  &  &  & 5x5deconv,2,3 & Kodak 4: 0.164819\\ &  &  &  &  & Kodak 5: 0.173699\\ &  &  &  &  & Kodak 6: 0.177930\\ &  &  &  &  & Kodak 7: 0.170581\\ &  &  &  &  & Kodak 8: 0.180944\\ &  &  &  &  & Kodak 9: 0.167729\\ &  &  &  &  & Kodak 10: 0.168607\\ &  &  &  &  & Kodak 11: 0.169597\\ &  &  &  &  & Kodak 12: 0.164297\\ &  &  &  &  & Kodak 13: 0.173647\\ &  &  &  &  & Kodak 14: 0.178460\\ &  &  &  &  & Kodak 15: 0.166762\\ &  &  &  &  & Kodak 16: 0.166881\\ &  &  &  &  & Kodak 17: 0.163149\\ &  &  &  &  & Kodak 18: 0.171846\\ &  &  &  &  & Kodak 19: 0.170759\\ &  &  &  &  & Kodak 20: 0.167110\\ &  &  &  &  & Kodak 21: 0.167543\\ &  &  &  &  & Kodak 22: 0.177368\\ &  &  &  &  & Kodak 23: 0.166455\\ &  &  &  &  & Kodak 24: 0.168746\\\hline\hline186 & MSE & 0.05 & 5x5deconv,2,10 & 5x5deconv,2,1 & Kodak 1: 0.090641\\ &  &  & 5x5deconv,2,10 & 5x5deconv,2,12 & Kodak 2: 0.102324\\ &  &  & 5x5deconv,2,320 & 5x5deconv,2,1 & Kodak 3: 0.098512\\ &  &  &  & 5x5deconv,2,3 & Kodak 4: 0.099905\\ &  &  &  &  & Kodak 5: 0.098929\\ &  &  &  &  & Kodak 6: 0.102909\\ &  &  &  &  & Kodak 7: 0.102863\\ &  &  &  &  & Kodak 8: 0.098351\\ &  &  &  &  & Kodak 9: 0.105421\\ &  &  &  &  & Kodak 10: 0.095097\\ &  &  &  &  & Kodak 11: 0.098865\\ &  &  &  &  & Kodak 12: 0.102337\\ &  &  &  &  & Kodak 13: 0.096802\\ &  &  &  &  & Kodak 14: 0.095557\\ &  &  &  &  & Kodak 15: 0.098839\\ &  &  &  &  & Kodak 16: 0.098755\\ &  &  &  &  & Kodak 17: 0.093870\\ &  &  &  &  & Kodak 18: 0.101576\\ &  &  &  &  & Kodak 19: 0.099053\\ &  &  &  &  & Kodak 20: 0.100704\\ &  &  &  &  & Kodak 21: 0.097757\\ &  &  &  &  & Kodak 22: 0.099408\\ &  &  &  &  & Kodak 23: 0.101306\\ &  &  &  &  & Kodak 24: 0.095834\\\hline\hline187 & MSE & 0.05 & 5x5deconv,2,10 & 5x5deconv,2,1 & Kodak 1: 0.095367\\ &  &  & 5x5deconv,2,10 & 5x5deconv,2,3 & Kodak 2: 0.103436\\ &  &  & 5x5deconv,2,320 & 5x5deconv,2,2 & Kodak 3: 0.097183\\ &  &  &  & 5x5deconv,2,3 & Kodak 4: 0.104762\\ &  &  &  &  & Kodak 5: 0.099778\\ &  &  &  &  & Kodak 6: 0.092536\\ &  &  &  &  & Kodak 7: 0.100160\\ &  &  &  &  & Kodak 8: 0.094272\\ &  &  &  &  & Kodak 9: 0.102982\\ &  &  &  &  & Kodak 10: 0.098239\\ &  &  &  &  & Kodak 11: 0.095258\\ &  &  &  &  & Kodak 12: 0.100732\\ &  &  &  &  & Kodak 13: 0.098490\\ &  &  &  &  & Kodak 14: 0.098086\\ &  &  &  &  & Kodak 15: 0.099683\\ &  &  &  &  & Kodak 16: 0.096337\\ &  &  &  &  & Kodak 17: 0.105326\\ &  &  &  &  & Kodak 18: 0.099547\\ &  &  &  &  & Kodak 19: 0.101231\\ &  &  &  &  & Kodak 20: 0.099908\\ &  &  &  &  & Kodak 21: 0.099454\\ &  &  &  &  & Kodak 22: 0.097354\\ &  &  &  &  & Kodak 23: 0.100052\\ &  &  &  &  & Kodak 24: 0.097259\\\hline\hline188 & MSE & 0.05 & 5x5deconv,2,10 & 5x5deconv,2,1 & Kodak 1: 0.086398\\ &  &  & 5x5deconv,2,10 & 5x5deconv,2,5 & Kodak 2: 0.098228\\ &  &  & 5x5deconv,2,320 & 5x5deconv,2,1 & Kodak 3: 0.100410\\ &  &  &  & 5x5deconv,2,3 & Kodak 4: 0.096640\\ &  &  &  &  & Kodak 5: 0.097739\\ &  &  &  &  & Kodak 6: 0.095757\\ &  &  &  &  & Kodak 7: 0.096358\\ &  &  &  &  & Kodak 8: 0.094149\\ &  &  &  &  & Kodak 9: 0.096858\\ &  &  &  &  & Kodak 10: 0.097035\\ &  &  &  &  & Kodak 11: 0.097837\\ &  &  &  &  & Kodak 12: 0.094789\\ &  &  &  &  & Kodak 13: 0.102947\\ &  &  &  &  & Kodak 14: 0.093680\\ &  &  &  &  & Kodak 15: 0.102369\\ &  &  &  &  & Kodak 16: 0.101785\\ &  &  &  &  & Kodak 17: 0.095666\\ &  &  &  &  & Kodak 18: 0.099149\\ &  &  &  &  & Kodak 19: 0.098351\\ &  &  &  &  & Kodak 20: 0.093926\\ &  &  &  &  & Kodak 21: 0.096339\\ &  &  &  &  & Kodak 22: 0.099676\\ &  &  &  &  & Kodak 23: 0.095750\\ &  &  &  &  & Kodak 24: 0.096786\\\hline\hline189 & MSE & 0.05 & 5x5deconv,2,88 & 5x5deconv,2,320 & Kodak 1: 0.501819\\ &  &  & 5x5deconv,2,289 & 5x5deconv,2,320 & Kodak 2: 0.474658\\ &  &  & 5x5deconv,2,320 & 5x5deconv,2,320 & Kodak 3: 0.480291\\ &  &  &  & 5x5deconv,2,3 & Kodak 4: 0.471158\\ &  &  &  &  & Kodak 5: 0.478964\\ &  &  &  &  & Kodak 6: 0.470920\\ &  &  &  &  & Kodak 7: 0.471655\\ &  &  &  &  & Kodak 8: 0.472885\\ &  &  &  &  & Kodak 9: 0.471309\\ &  &  &  &  & Kodak 10: 0.466981\\ &  &  &  &  & Kodak 11: 0.469421\\ &  &  &  &  & Kodak 12: 0.473141\\ &  &  &  &  & Kodak 13: 0.478846\\ &  &  &  &  & Kodak 14: 0.527865\\ &  &  &  &  & Kodak 15: 0.471504\\ &  &  &  &  & Kodak 16: 0.468302\\ &  &  &  &  & Kodak 17: 0.468427\\ &  &  &  &  & Kodak 18: 0.465625\\ &  &  &  &  & Kodak 19: 0.472588\\ &  &  &  &  & Kodak 20: 0.481144\\ &  &  &  &  & Kodak 21: 0.476037\\ &  &  &  &  & Kodak 22: 0.467989\\ &  &  &  &  & Kodak 23: 0.460921\\ &  &  &  &  & Kodak 24: 0.468940\\\hline\hline190 & MSE & 0.05 & 5x5deconv,2,62 & 5x5deconv,2,320 & Kodak 1: 0.494783\\ &  &  & 5x5deconv,2,52 & 5x5deconv,2,320 & Kodak 2: 0.477391\\ &  &  & 5x5deconv,2,320 & 5x5deconv,2,320 & Kodak 3: 0.468677\\ &  &  &  & 5x5deconv,2,3 & Kodak 4: 0.464514\\ &  &  &  &  & Kodak 5: 0.473569\\ &  &  &  &  & Kodak 6: 0.470127\\ &  &  &  &  & Kodak 7: 0.469487\\ &  &  &  &  & Kodak 8: 0.480378\\ &  &  &  &  & Kodak 9: 0.465157\\ &  &  &  &  & Kodak 10: 0.465168\\ &  &  &  &  & Kodak 11: 0.466671\\ &  &  &  &  & Kodak 12: 0.466518\\ &  &  &  &  & Kodak 13: 0.540718\\ &  &  &  &  & Kodak 14: 0.481302\\ &  &  &  &  & Kodak 15: 0.461873\\ &  &  &  &  & Kodak 16: 0.471496\\ &  &  &  &  & Kodak 17: 0.466374\\ &  &  &  &  & Kodak 18: 0.467062\\ &  &  &  &  & Kodak 19: 0.469834\\ &  &  &  &  & Kodak 20: 0.470154\\ &  &  &  &  & Kodak 21: 0.470411\\ &  &  &  &  & Kodak 22: 0.468162\\ &  &  &  &  & Kodak 23: 0.461978\\ &  &  &  &  & Kodak 24: 0.471161\\\hline\hline191 & MSE & 0.05 & 5x5deconv,2,10 & 5x5deconv,2,10 & Kodak 1: 0.096806\\ &  &  & 5x5deconv,2,3 & 5x5deconv,2,11 & Kodak 2: 0.109114\\ &  &  & 5x5deconv,2,320 & 5x5deconv,2,4 & Kodak 3: 0.101319\\ &  &  &  & 5x5deconv,2,3 & Kodak 4: 0.098683\\ &  &  &  &  & Kodak 5: 0.102173\\ &  &  &  &  & Kodak 6: 0.104632\\ &  &  &  &  & Kodak 7: 0.101605\\ &  &  &  &  & Kodak 8: 0.100489\\ &  &  &  &  & Kodak 9: 0.107547\\ &  &  &  &  & Kodak 10: 0.100915\\ &  &  &  &  & Kodak 11: 0.100234\\ &  &  &  &  & Kodak 12: 0.099053\\ &  &  &  &  & Kodak 13: 0.102042\\ &  &  &  &  & Kodak 14: 0.102448\\ &  &  &  &  & Kodak 15: 0.100120\\ &  &  &  &  & Kodak 16: 0.103059\\ &  &  &  &  & Kodak 17: 0.101942\\ &  &  &  &  & Kodak 18: 0.106251\\ &  &  &  &  & Kodak 19: 0.106173\\ &  &  &  &  & Kodak 20: 0.103477\\ &  &  &  &  & Kodak 21: 0.102577\\ &  &  &  &  & Kodak 22: 0.102605\\ &  &  &  &  & Kodak 23: 0.101329\\ &  &  &  &  & Kodak 24: 0.100974\\\hline\hline192 & MSE & 0.05 & 5x5deconv,2,459 & 5x5deconv,2,320 & Kodak 1: 0.528644\\ &  &  & 5x5deconv,2,256 & 5x5deconv,2,320 & Kodak 2: 0.491261\\ &  &  & 5x5deconv,2,320 & 5x5deconv,2,319 & Kodak 3: 0.484284\\ &  &  &  & 5x5deconv,2,3 & Kodak 4: 0.540462\\ &  &  &  &  & Kodak 5: 0.485789\\ &  &  &  &  & Kodak 6: 0.484724\\ &  &  &  &  & Kodak 7: 0.488218\\ &  &  &  &  & Kodak 8: 0.486942\\ &  &  &  &  & Kodak 9: 0.480459\\ &  &  &  &  & Kodak 10: 0.484623\\ &  &  &  &  & Kodak 11: 0.482871\\ &  &  &  &  & Kodak 12: 0.485033\\ &  &  &  &  & Kodak 13: 0.490891\\ &  &  &  &  & Kodak 14: 0.487802\\ &  &  &  &  & Kodak 15: 0.485869\\ &  &  &  &  & Kodak 16: 0.484456\\ &  &  &  &  & Kodak 17: 0.485411\\ &  &  &  &  & Kodak 18: 0.489072\\ &  &  &  &  & Kodak 19: 0.489249\\ &  &  &  &  & Kodak 20: 0.487254\\ &  &  &  &  & Kodak 21: 0.489521\\ &  &  &  &  & Kodak 22: 0.486942\\ &  &  &  &  & Kodak 23: 0.538074\\ &  &  &  &  & Kodak 24: 0.492538\\\hline\hline193 & MSE & 0.05 & 5x5deconv,2,10 & 5x5deconv,2,1 & Kodak 1: 0.094509\\ &  &  & 5x5deconv,2,10 & 5x5deconv,2,6 & Kodak 2: 0.106388\\ &  &  & 5x5deconv,2,320 & 5x5deconv,2,1 & Kodak 3: 0.099050\\ &  &  &  & 5x5deconv,2,3 & Kodak 4: 0.102959\\ &  &  &  &  & Kodak 5: 0.104580\\ &  &  &  &  & Kodak 6: 0.106726\\ &  &  &  &  & Kodak 7: 0.095636\\ &  &  &  &  & Kodak 8: 0.097985\\ &  &  &  &  & Kodak 9: 0.099930\\ &  &  &  &  & Kodak 10: 0.095946\\ &  &  &  &  & Kodak 11: 0.102085\\ &  &  &  &  & Kodak 12: 0.098444\\ &  &  &  &  & Kodak 13: 0.098104\\ &  &  &  &  & Kodak 14: 0.097455\\ &  &  &  &  & Kodak 15: 0.101744\\ &  &  &  &  & Kodak 16: 0.097409\\ &  &  &  &  & Kodak 17: 0.102187\\ &  &  &  &  & Kodak 18: 0.097752\\ &  &  &  &  & Kodak 19: 0.095807\\ &  &  &  &  & Kodak 20: 0.098773\\ &  &  &  &  & Kodak 21: 0.095452\\ &  &  &  &  & Kodak 22: 0.097736\\ &  &  &  &  & Kodak 23: 0.096363\\ &  &  &  &  & Kodak 24: 0.093461\\\hline\hline194 & MSE & 0.05 & 5x5deconv,2,252 & 5x5deconv,2,320 & Kodak 1: 0.508303\\ &  &  & 5x5deconv,2,227 & 5x5deconv,2,320 & Kodak 2: 0.472119\\ &  &  & 5x5deconv,2,320 & 5x5deconv,2,320 & Kodak 3: 0.496493\\ &  &  &  & 5x5deconv,2,3 & Kodak 4: 0.480904\\ &  &  &  &  & Kodak 5: 0.531055\\ &  &  &  &  & Kodak 6: 0.474418\\ &  &  &  &  & Kodak 7: 0.476616\\ &  &  &  &  & Kodak 8: 0.475445\\ &  &  &  &  & Kodak 9: 0.470417\\ &  &  &  &  & Kodak 10: 0.468349\\ &  &  &  &  & Kodak 11: 0.469921\\ &  &  &  &  & Kodak 12: 0.468752\\ &  &  &  &  & Kodak 13: 0.484635\\ &  &  &  &  & Kodak 14: 0.470529\\ &  &  &  &  & Kodak 15: 0.473866\\ &  &  &  &  & Kodak 16: 0.473456\\ &  &  &  &  & Kodak 17: 0.469753\\ &  &  &  &  & Kodak 18: 0.470965\\ &  &  &  &  & Kodak 19: 0.470672\\ &  &  &  &  & Kodak 20: 0.467795\\ &  &  &  &  & Kodak 21: 0.468527\\ &  &  &  &  & Kodak 22: 0.469535\\ &  &  &  &  & Kodak 23: 0.468780\\ &  &  &  &  & Kodak 24: 0.471893\\\hline\hline195 & MSE & 0.05 & 5x5deconv,2,10 & 5x5deconv,2,1 & Kodak 1: 0.088049\\ &  &  & 5x5deconv,2,10 & 5x5deconv,2,3 & Kodak 2: 0.097119\\ &  &  & 5x5deconv,2,320 & 5x5deconv,2,1 & Kodak 3: 0.099223\\ &  &  &  & 5x5deconv,2,3 & Kodak 4: 0.096761\\ &  &  &  &  & Kodak 5: 0.097959\\ &  &  &  &  & Kodak 6: 0.094737\\ &  &  &  &  & Kodak 7: 0.096507\\ &  &  &  &  & Kodak 8: 0.101378\\ &  &  &  &  & Kodak 9: 0.096789\\ &  &  &  &  & Kodak 10: 0.102337\\ &  &  &  &  & Kodak 11: 0.097888\\ &  &  &  &  & Kodak 12: 0.094244\\ &  &  &  &  & Kodak 13: 0.094676\\ &  &  &  &  & Kodak 14: 0.095432\\ &  &  &  &  & Kodak 15: 0.098881\\ &  &  &  &  & Kodak 16: 0.095210\\ &  &  &  &  & Kodak 17: 0.098468\\ &  &  &  &  & Kodak 18: 0.102805\\ &  &  &  &  & Kodak 19: 0.095671\\ &  &  &  &  & Kodak 20: 0.098857\\ &  &  &  &  & Kodak 21: 0.099783\\ &  &  &  &  & Kodak 22: 0.092909\\ &  &  &  &  & Kodak 23: 0.100584\\ &  &  &  &  & Kodak 24: 0.098602\\\hline\hline196 & MSE & 0.05 & 5x5deconv,2,106 & 5x5deconv,2,320 & Kodak 1: 0.506314\\ &  &  & 5x5deconv,2,351 & 5x5deconv,2,320 & Kodak 2: 0.472986\\ &  &  & 5x5deconv,2,320 & 5x5deconv,2,320 & Kodak 3: 0.475772\\ &  &  &  & 5x5deconv,2,3 & Kodak 4: 0.471882\\ &  &  &  &  & Kodak 5: 0.485752\\ &  &  &  &  & Kodak 6: 0.490591\\ &  &  &  &  & Kodak 7: 0.479999\\ &  &  &  &  & Kodak 8: 0.480854\\ &  &  &  &  & Kodak 9: 0.467549\\ &  &  &  &  & Kodak 10: 0.471060\\ &  &  &  &  & Kodak 11: 0.469383\\ &  &  &  &  & Kodak 12: 0.476788\\ &  &  &  &  & Kodak 13: 0.486368\\ &  &  &  &  & Kodak 14: 0.482346\\ &  &  &  &  & Kodak 15: 0.471183\\ &  &  &  &  & Kodak 16: 0.468805\\ &  &  &  &  & Kodak 17: 0.469706\\ &  &  &  &  & Kodak 18: 0.468759\\ &  &  &  &  & Kodak 19: 0.478241\\ &  &  &  &  & Kodak 20: 0.491747\\ &  &  &  &  & Kodak 21: 0.482151\\ &  &  &  &  & Kodak 22: 0.474670\\ &  &  &  &  & Kodak 23: 0.471389\\ &  &  &  &  & Kodak 24: 0.469166\\\hline\hline197 & MSE & 0.05 & 5x5deconv,2,26 & 5x5deconv,2,99 & Kodak 1: 0.133990\\ &  &  & 5x5deconv,2,19 & 5x5deconv,2,32 & Kodak 2: 0.127219\\ &  &  & 5x5deconv,2,320 & 5x5deconv,2,26 & Kodak 3: 0.129135\\ &  &  &  & 5x5deconv,2,3 & Kodak 4: 0.125994\\ &  &  &  &  & Kodak 5: 0.126064\\ &  &  &  &  & Kodak 6: 0.134413\\ &  &  &  &  & Kodak 7: 0.130285\\ &  &  &  &  & Kodak 8: 0.127093\\ &  &  &  &  & Kodak 9: 0.118786\\ &  &  &  &  & Kodak 10: 0.127128\\ &  &  &  &  & Kodak 11: 0.129679\\ &  &  &  &  & Kodak 12: 0.120897\\ &  &  &  &  & Kodak 13: 0.130166\\ &  &  &  &  & Kodak 14: 0.132972\\ &  &  &  &  & Kodak 15: 0.123939\\ &  &  &  &  & Kodak 16: 0.129447\\ &  &  &  &  & Kodak 17: 0.131366\\ &  &  &  &  & Kodak 18: 0.131213\\ &  &  &  &  & Kodak 19: 0.132870\\ &  &  &  &  & Kodak 20: 0.122116\\ &  &  &  &  & Kodak 21: 0.120352\\ &  &  &  &  & Kodak 22: 0.123288\\ &  &  &  &  & Kodak 23: 0.127013\\ &  &  &  &  & Kodak 24: 0.120389\\\hline\hline198 & MSE & 0.05 & 5x5deconv,2,103 & 5x5deconv,2,320 & Kodak 1: 0.493878\\ &  &  & 5x5deconv,2,103 & 5x5deconv,2,320 & Kodak 2: 0.472454\\ &  &  & 5x5deconv,2,320 & 5x5deconv,2,320 & Kodak 3: 0.468986\\ &  &  &  & 5x5deconv,2,3 & Kodak 4: 0.458945\\ &  &  &  &  & Kodak 5: 0.467565\\ &  &  &  &  & Kodak 6: 0.476920\\ &  &  &  &  & Kodak 7: 0.465441\\ &  &  &  &  & Kodak 8: 0.525998\\ &  &  &  &  & Kodak 9: 0.464813\\ &  &  &  &  & Kodak 10: 0.461440\\ &  &  &  &  & Kodak 11: 0.466472\\ &  &  &  &  & Kodak 12: 0.474341\\ &  &  &  &  & Kodak 13: 0.473029\\ &  &  &  &  & Kodak 14: 0.518383\\ &  &  &  &  & Kodak 15: 0.471497\\ &  &  &  &  & Kodak 16: 0.467752\\ &  &  &  &  & Kodak 17: 0.470432\\ &  &  &  &  & Kodak 18: 0.468486\\ &  &  &  &  & Kodak 19: 0.461914\\ &  &  &  &  & Kodak 20: 0.522673\\ &  &  &  &  & Kodak 21: 0.471015\\ &  &  &  &  & Kodak 22: 0.468083\\ &  &  &  &  & Kodak 23: 0.460362\\ &  &  &  &  & Kodak 24: 0.462362\\\hline\hline199 & MSE & 0.05 & 5x5deconv,2,9 & 5x5deconv,2,30 & Kodak 1: 0.114222\\ &  &  & 5x5deconv,2,14 & 5x5deconv,2,15 & Kodak 2: 0.120102\\ &  &  & 5x5deconv,2,320 & 5x5deconv,2,14 & Kodak 3: 0.113898\\ &  &  &  & 5x5deconv,2,3 & Kodak 4: 0.113607\\ &  &  &  &  & Kodak 5: 0.111320\\ &  &  &  &  & Kodak 6: 0.114552\\ &  &  &  &  & Kodak 7: 0.114598\\ &  &  &  &  & Kodak 8: 0.121266\\ &  &  &  &  & Kodak 9: 0.117799\\ &  &  &  &  & Kodak 10: 0.108079\\ &  &  &  &  & Kodak 11: 0.117917\\ &  &  &  &  & Kodak 12: 0.115463\\ &  &  &  &  & Kodak 13: 0.117226\\ &  &  &  &  & Kodak 14: 0.112419\\ &  &  &  &  & Kodak 15: 0.123050\\ &  &  &  &  & Kodak 16: 0.117403\\ &  &  &  &  & Kodak 17: 0.116473\\ &  &  &  &  & Kodak 18: 0.113495\\ &  &  &  &  & Kodak 19: 0.113656\\ &  &  &  &  & Kodak 20: 0.116975\\ &  &  &  &  & Kodak 21: 0.121814\\ &  &  &  &  & Kodak 22: 0.115917\\ &  &  &  &  & Kodak 23: 0.111338\\ &  &  &  &  & Kodak 24: 0.111286\\\hline\hline200 & MSE & 0.003125 & 5x5deconv,2,10 & 5x5deconv,2,1 & Kodak 1: 0.093596\\ &  &  & 5x5deconv,2,10 & 5x5deconv,2,3 & Kodak 2: 0.099939\\ &  &  & 5x5deconv,2,320 & 5x5deconv,2,1 & Kodak 3: 0.105866\\ &  &  &  & 5x5deconv,2,3 & Kodak 4: 0.095895\\ &  &  &  &  & Kodak 5: 0.100406\\ &  &  &  &  & Kodak 6: 0.097824\\ &  &  &  &  & Kodak 7: 0.101529\\ &  &  &  &  & Kodak 8: 0.097675\\ &  &  &  &  & Kodak 9: 0.095963\\ &  &  &  &  & Kodak 10: 0.095072\\ &  &  &  &  & Kodak 11: 0.103260\\ &  &  &  &  & Kodak 12: 0.102787\\ &  &  &  &  & Kodak 13: 0.093927\\ &  &  &  &  & Kodak 14: 0.098117\\ &  &  &  &  & Kodak 15: 0.102805\\ &  &  &  &  & Kodak 16: 0.095711\\ &  &  &  &  & Kodak 17: 0.095740\\ &  &  &  &  & Kodak 18: 0.103483\\ &  &  &  &  & Kodak 19: 0.097518\\ &  &  &  &  & Kodak 20: 0.097799\\ &  &  &  &  & Kodak 21: 0.104311\\ &  &  &  &  & Kodak 22: 0.108709\\ &  &  &  &  & Kodak 23: 0.103286\\ &  &  &  &  & Kodak 24: 0.108305\\\hline\hline201 & MSE & 0.003125 & 5x5deconv,2,10 & 5x5deconv,2,1 & Kodak 1: 0.089408\\ &  &  & 5x5deconv,2,10 & 5x5deconv,2,1 & Kodak 2: 0.096232\\ &  &  & 5x5deconv,2,320 & 5x5deconv,2,1 & Kodak 3: 0.104397\\ &  &  &  & 5x5deconv,2,3 & Kodak 4: 0.094185\\ &  &  &  &  & Kodak 5: 0.098732\\ &  &  &  &  & Kodak 6: 0.098295\\ &  &  &  &  & Kodak 7: 0.100754\\ &  &  &  &  & Kodak 8: 0.096942\\ &  &  &  &  & Kodak 9: 0.101081\\ &  &  &  &  & Kodak 10: 0.100206\\ &  &  &  &  & Kodak 11: 0.096961\\ &  &  &  &  & Kodak 12: 0.101319\\ &  &  &  &  & Kodak 13: 0.105446\\ &  &  &  &  & Kodak 14: 0.101041\\ &  &  &  &  & Kodak 15: 0.105349\\ &  &  &  &  & Kodak 16: 0.100968\\ &  &  &  &  & Kodak 17: 0.097771\\ &  &  &  &  & Kodak 18: 0.095942\\ &  &  &  &  & Kodak 19: 0.097214\\ &  &  &  &  & Kodak 20: 0.097111\\ &  &  &  &  & Kodak 21: 0.096309\\ &  &  &  &  & Kodak 22: 0.099043\\ &  &  &  &  & Kodak 23: 0.099910\\ &  &  &  &  & Kodak 24: 0.102514\\\hline\hline202 & MSE & 0.003125 & 5x5deconv,2,398 & 5x5deconv,2,188 & Kodak 1: 0.261360\\ &  &  & 5x5deconv,2,207 & 5x5deconv,2,101 & Kodak 2: 0.237359\\ &  &  & 5x5deconv,2,320 & 5x5deconv,2,188 & Kodak 3: 0.243190\\ &  &  &  & 5x5deconv,2,3 & Kodak 4: 0.247262\\ &  &  &  &  & Kodak 5: 0.236678\\ &  &  &  &  & Kodak 6: 0.242214\\ &  &  &  &  & Kodak 7: 0.281970\\ &  &  &  &  & Kodak 8: 0.239891\\ &  &  &  &  & Kodak 9: 0.244757\\ &  &  &  &  & Kodak 10: 0.267808\\ &  &  &  &  & Kodak 11: 0.274945\\ &  &  &  &  & Kodak 12: 0.274762\\ &  &  &  &  & Kodak 13: 0.243915\\ &  &  &  &  & Kodak 14: 0.245917\\ &  &  &  &  & Kodak 15: 0.243272\\ &  &  &  &  & Kodak 16: 0.245859\\ &  &  &  &  & Kodak 17: 0.277277\\ &  &  &  &  & Kodak 18: 0.282646\\ &  &  &  &  & Kodak 19: 0.241626\\ &  &  &  &  & Kodak 20: 0.239971\\ &  &  &  &  & Kodak 21: 0.247538\\ &  &  &  &  & Kodak 22: 0.246713\\ &  &  &  &  & Kodak 23: 0.242783\\ &  &  &  &  & Kodak 24: 0.242492\\\hline\hline203 & MSE & 0.003125 & 5x5deconv,2,74 & 5x5deconv,2,60 & Kodak 1: 0.124417\\ &  &  & 5x5deconv,2,74 & 5x5deconv,2,32 & Kodak 2: 0.127467\\ &  &  & 5x5deconv,2,320 & 5x5deconv,2,53 & Kodak 3: 0.136543\\ &  &  &  & 5x5deconv,2,3 & Kodak 4: 0.130703\\ &  &  &  &  & Kodak 5: 0.133479\\ &  &  &  &  & Kodak 6: 0.132121\\ &  &  &  &  & Kodak 7: 0.135542\\ &  &  &  &  & Kodak 8: 0.138238\\ &  &  &  &  & Kodak 9: 0.127985\\ &  &  &  &  & Kodak 10: 0.133661\\ &  &  &  &  & Kodak 11: 0.129758\\ &  &  &  &  & Kodak 12: 0.137430\\ &  &  &  &  & Kodak 13: 0.139050\\ &  &  &  &  & Kodak 14: 0.132966\\ &  &  &  &  & Kodak 15: 0.133186\\ &  &  &  &  & Kodak 16: 0.134032\\ &  &  &  &  & Kodak 17: 0.131135\\ &  &  &  &  & Kodak 18: 0.132392\\ &  &  &  &  & Kodak 19: 0.132919\\ &  &  &  &  & Kodak 20: 0.131260\\ &  &  &  &  & Kodak 21: 0.133721\\ &  &  &  &  & Kodak 22: 0.127949\\ &  &  &  &  & Kodak 23: 0.133522\\ &  &  &  &  & Kodak 24: 0.133854\\\hline\hline204 & MSE & 0.003125 & 5x5deconv,2,10 & 5x5deconv,2,1 & Kodak 1: 0.092829\\ &  &  & 5x5deconv,2,10 & 5x5deconv,2,4 & Kodak 2: 0.104815\\ &  &  & 5x5deconv,2,320 & 5x5deconv,2,1 & Kodak 3: 0.100739\\ &  &  &  & 5x5deconv,2,3 & Kodak 4: 0.102009\\ &  &  &  &  & Kodak 5: 0.098658\\ &  &  &  &  & Kodak 6: 0.099809\\ &  &  &  &  & Kodak 7: 0.099941\\ &  &  &  &  & Kodak 8: 0.098865\\ &  &  &  &  & Kodak 9: 0.099433\\ &  &  &  &  & Kodak 10: 0.099509\\ &  &  &  &  & Kodak 11: 0.094873\\ &  &  &  &  & Kodak 12: 0.097581\\ &  &  &  &  & Kodak 13: 0.102539\\ &  &  &  &  & Kodak 14: 0.099640\\ &  &  &  &  & Kodak 15: 0.099511\\ &  &  &  &  & Kodak 16: 0.098549\\ &  &  &  &  & Kodak 17: 0.103476\\ &  &  &  &  & Kodak 18: 0.098695\\ &  &  &  &  & Kodak 19: 0.104260\\ &  &  &  &  & Kodak 20: 0.097236\\ &  &  &  &  & Kodak 21: 0.098291\\ &  &  &  &  & Kodak 22: 0.095114\\ &  &  &  &  & Kodak 23: 0.096853\\ &  &  &  &  & Kodak 24: 0.105038\\\hline\hline205 & MSE & 0.003125 & 5x5deconv,2,12 & 5x5deconv,2,8 & Kodak 1: 0.103230\\ &  &  & 5x5deconv,2,11 & 5x5deconv,2,13 & Kodak 2: 0.100933\\ &  &  & 5x5deconv,2,320 & 5x5deconv,2,6 & Kodak 3: 0.109118\\ &  &  &  & 5x5deconv,2,3 & Kodak 4: 0.107326\\ &  &  &  &  & Kodak 5: 0.114632\\ &  &  &  &  & Kodak 6: 0.107196\\ &  &  &  &  & Kodak 7: 0.104969\\ &  &  &  &  & Kodak 8: 0.109173\\ &  &  &  &  & Kodak 9: 0.105393\\ &  &  &  &  & Kodak 10: 0.103687\\ &  &  &  &  & Kodak 11: 0.112418\\ &  &  &  &  & Kodak 12: 0.109319\\ &  &  &  &  & Kodak 13: 0.115812\\ &  &  &  &  & Kodak 14: 0.103803\\ &  &  &  &  & Kodak 15: 0.105810\\ &  &  &  &  & Kodak 16: 0.100425\\ &  &  &  &  & Kodak 17: 0.103774\\ &  &  &  &  & Kodak 18: 0.103240\\ &  &  &  &  & Kodak 19: 0.102608\\ &  &  &  &  & Kodak 20: 0.107290\\ &  &  &  &  & Kodak 21: 0.107832\\ &  &  &  &  & Kodak 22: 0.100058\\ &  &  &  &  & Kodak 23: 0.109246\\ &  &  &  &  & Kodak 24: 0.101456\\\hline\hline206 & MSE & 0.003125 & 5x5deconv,2,35 & 5x5deconv,2,27 & Kodak 1: 0.117312\\ &  &  & 5x5deconv,2,23 & 5x5deconv,2,21 & Kodak 2: 0.113621\\ &  &  & 5x5deconv,2,320 & 5x5deconv,2,10 & Kodak 3: 0.113748\\ &  &  &  & 5x5deconv,2,3 & Kodak 4: 0.118523\\ &  &  &  &  & Kodak 5: 0.120274\\ &  &  &  &  & Kodak 6: 0.111768\\ &  &  &  &  & Kodak 7: 0.117932\\ &  &  &  &  & Kodak 8: 0.117372\\ &  &  &  &  & Kodak 9: 0.108027\\ &  &  &  &  & Kodak 10: 0.102897\\ &  &  &  &  & Kodak 11: 0.110026\\ &  &  &  &  & Kodak 12: 0.115339\\ &  &  &  &  & Kodak 13: 0.111660\\ &  &  &  &  & Kodak 14: 0.108366\\ &  &  &  &  & Kodak 15: 0.109320\\ &  &  &  &  & Kodak 16: 0.110274\\ &  &  &  &  & Kodak 17: 0.115223\\ &  &  &  &  & Kodak 18: 0.108264\\ &  &  &  &  & Kodak 19: 0.110039\\ &  &  &  &  & Kodak 20: 0.120360\\ &  &  &  &  & Kodak 21: 0.104395\\ &  &  &  &  & Kodak 22: 0.104876\\ &  &  &  &  & Kodak 23: 0.120498\\ &  &  &  &  & Kodak 24: 0.115671\\\hline\hline207 & MSE & 0.003125 & 5x5deconv,2,121 & 5x5deconv,2,320 & Kodak 1: 0.494832\\ &  &  & 5x5deconv,2,316 & 5x5deconv,2,320 & Kodak 2: 0.469768\\ &  &  & 5x5deconv,2,320 & 5x5deconv,2,320 & Kodak 3: 0.473788\\ &  &  &  & 5x5deconv,2,3 & Kodak 4: 0.467977\\ &  &  &  &  & Kodak 5: 0.467127\\ &  &  &  &  & Kodak 6: 0.471951\\ &  &  &  &  & Kodak 7: 0.466982\\ &  &  &  &  & Kodak 8: 0.468523\\ &  &  &  &  & Kodak 9: 0.465351\\ &  &  &  &  & Kodak 10: 0.476288\\ &  &  &  &  & Kodak 11: 0.468099\\ &  &  &  &  & Kodak 12: 0.474387\\ &  &  &  &  & Kodak 13: 0.533650\\ &  &  &  &  & Kodak 14: 0.471074\\ &  &  &  &  & Kodak 15: 0.473696\\ &  &  &  &  & Kodak 16: 0.472049\\ &  &  &  &  & Kodak 17: 0.465898\\ &  &  &  &  & Kodak 18: 0.469561\\ &  &  &  &  & Kodak 19: 0.477750\\ &  &  &  &  & Kodak 20: 0.472596\\ &  &  &  &  & Kodak 21: 0.478737\\ &  &  &  &  & Kodak 22: 0.475598\\ &  &  &  &  & Kodak 23: 0.470628\\ &  &  &  &  & Kodak 24: 0.469402\\\hline\hline\hline\hline209 & MSE & 0.003125 & 5x5deconv,2,569 & 5x5deconv,2,320 & Kodak 1: 0.478854\\ &  &  & 5x5deconv,2,187 & 5x5deconv,2,273 & Kodak 2: 0.448432\\ &  &  & 5x5deconv,2,320 & 5x5deconv,2,319 & Kodak 3: 0.452975\\ &  &  &  & 5x5deconv,2,3 & Kodak 4: 0.455382\\ &  &  &  &  & Kodak 5: 0.444539\\ &  &  &  &  & Kodak 6: 0.447735\\ &  &  &  &  & Kodak 7: 0.444336\\ &  &  &  &  & Kodak 8: 0.457325\\ &  &  &  &  & Kodak 9: 0.440492\\ &  &  &  &  & Kodak 10: 0.455813\\ &  &  &  &  & Kodak 11: 0.443405\\ &  &  &  &  & Kodak 12: 0.543502\\ &  &  &  &  & Kodak 13: 0.450840\\ &  &  &  &  & Kodak 14: 0.449387\\ &  &  &  &  & Kodak 15: 0.453267\\ &  &  &  &  & Kodak 16: 0.447957\\ &  &  &  &  & Kodak 17: 0.455001\\ &  &  &  &  & Kodak 18: 0.456695\\ &  &  &  &  & Kodak 19: 0.448196\\ &  &  &  &  & Kodak 20: 0.449962\\ &  &  &  &  & Kodak 21: 0.501584\\ &  &  &  &  & Kodak 22: 0.447701\\ &  &  &  &  & Kodak 23: 0.449534\\ &  &  &  &  & Kodak 24: 0.449319\\\hline\hline210 & MSE & 0.003125 & 5x5deconv,2,167 & 5x5deconv,2,135 & Kodak 1: 0.210887\\ &  &  & 5x5deconv,2,121 & 5x5deconv,2,64 & Kodak 2: 0.181708\\ &  &  & 5x5deconv,2,320 & 5x5deconv,2,128 & Kodak 3: 0.191569\\ &  &  &  & 5x5deconv,2,3 & Kodak 4: 0.185986\\ &  &  &  &  & Kodak 5: 0.191935\\ &  &  &  &  & Kodak 6: 0.182512\\ &  &  &  &  & Kodak 7: 0.190579\\ &  &  &  &  & Kodak 8: 0.186016\\ &  &  &  &  & Kodak 9: 0.191439\\ &  &  &  &  & Kodak 10: 0.184501\\ &  &  &  &  & Kodak 11: 0.183844\\ &  &  &  &  & Kodak 12: 0.188102\\ &  &  &  &  & Kodak 13: 0.183625\\ &  &  &  &  & Kodak 14: 0.208289\\ &  &  &  &  & Kodak 15: 0.181000\\ &  &  &  &  & Kodak 16: 0.179821\\ &  &  &  &  & Kodak 17: 0.180982\\ &  &  &  &  & Kodak 18: 0.184764\\ &  &  &  &  & Kodak 19: 0.191856\\ &  &  &  &  & Kodak 20: 0.185940\\ &  &  &  &  & Kodak 21: 0.183742\\ &  &  &  &  & Kodak 22: 0.180765\\ &  &  &  &  & Kodak 23: 0.183356\\ &  &  &  &  & Kodak 24: 0.194728\\\hline\hline211 & MSE & 0.003125 & 5x5deconv,2,299 & 5x5deconv,2,273 & Kodak 1: 0.389332\\ &  &  & 5x5deconv,2,263 & 5x5deconv,2,178 & Kodak 2: 0.366968\\ &  &  & 5x5deconv,2,320 & 5x5deconv,2,304 & Kodak 3: 0.380990\\ &  &  &  & 5x5deconv,2,3 & Kodak 4: 0.360892\\ &  &  &  &  & Kodak 5: 0.364912\\ &  &  &  &  & Kodak 6: 0.362504\\ &  &  &  &  & Kodak 7: 0.357273\\ &  &  &  &  & Kodak 8: 0.361339\\ &  &  &  &  & Kodak 9: 0.414591\\ &  &  &  &  & Kodak 10: 0.365760\\ &  &  &  &  & Kodak 11: 0.368428\\ &  &  &  &  & Kodak 12: 0.420032\\ &  &  &  &  & Kodak 13: 0.365860\\ &  &  &  &  & Kodak 14: 0.362373\\ &  &  &  &  & Kodak 15: 0.380785\\ &  &  &  &  & Kodak 16: 0.358225\\ &  &  &  &  & Kodak 17: 0.357989\\ &  &  &  &  & Kodak 18: 0.363192\\ &  &  &  &  & Kodak 19: 0.366556\\ &  &  &  &  & Kodak 20: 0.362197\\ &  &  &  &  & Kodak 21: 0.361126\\ &  &  &  &  & Kodak 22: 0.360811\\ &  &  &  &  & Kodak 23: 0.369179\\ &  &  &  &  & Kodak 24: 0.361622\\\hline
